# Supplementary material for: Learning proofs for the classification of nilpotent semigroups
Source: arXiv:2106.03015 ancillary file (2021-06-06)

```

1 #####
2 #####   sgLearnNil4.ipynb
3 #####   a notebook for machine learning proofs for classification of nilpotent
4 #####   carlos.simpson@univ-cotedazur.fr
5 #####   https://github.com/carlostsimpson/sg-learn
6 #####   distributed under: GNU General Public License v3.0
7 #####

```

```

1 import numpy as np
2 import matplotlib.pyplot as plt
3 import random
4 import time
5 import copy
6 import math
7 import datetime
8
9 import gc
10
11 class CoherenceError(Exception):
12     pass

```

```

1 from __future__ import print_function
2 import torch
3
4 import torch.nn as nn
5 import torch.nn.functional as F
6
7 from torch import optim
8

```

```

1 # try to put everything on gpu if it exists
2
3 if torch.cuda.is_available():
4     Dvc = torch.device("cuda:0")
5     print("Running on GPU cuda:0")
6 else:
7     Dvc = torch.device("cpu")
8     print("Running on CPU")
9
10 CpuDvc = torch.device("cpu")
11

```

```

1 #Dvc = torch.device("cpu") # in case you need to force it to cpu (e.g. cuda com

```

```

1 ###

```

```

1 def zbinary(depth,z): # the smallest digits are first here (i.e. reads backward
2     binnum = [int(i) for i in bin(z)[2:]]
3     bnlength = len(binnum)
4     if bnlength > depth:

```

```

11     blength = depth
12     print("warning: applying zbinary to",z,"with depth",depth,"but bin length",blength)
13     outputarray = torch.zeros((depth),dtype = torch.bool,device=Dvc)
14     for j in range(depth):
15         if j < blength:
16             outputarray[j] = (binnum[blength - j-1] == 1)
17         else:
18             outputarray[j] = False
19     return outputarray
20
21 def binaryz(depth,binarray):
22     thez = 0
23     for i in range(depth):
24         thez += binarray.to(torch.int)[i] * 2**i
25     return thez
26
27 def binaryzbatch(length,depth,binarray_batch):
28     zbatch = torch.zeros((length),dtype = torch.int64,device=Dvc)
29     for i in range(depth):
30         zbatch += binarray_batch.to(torch.int)[: ,i] * (2**i)
31     return zbatch
32
33 def composepermutations(vector1,vector2):
34     vector2i64 = vector2.to(torch.int64)
35     composition = vector1[vector2i64]
36     return composition
37
38 def composedetections(length,detection1,detection2): # outputs the result of de
39     output = torch.zeros((length),dtype = torch.bool,device=Dvc)
40     output[detection1] = detection2
41     return output
42
43 def memReport(style): # by QuantScientist Solomon K @smth
44     if style == 'memory':
45         print("gc memory report")
46         for obj in gc.get_objects():
47             if torch.is_tensor(obj):
48                 print(type(obj), obj.size())
49     if style == 'mg':
50         print("gc memory and garbage report::",end=' ')
51         allobjects = gc.get_objects()
52         all_length = len(allobjects)
53         elements = torch.zeros((all_length),dtype = torch.int64,device=Dvc)
54         count = 0
55         loc = 0
56         for obj in allobjects:
57             if torch.is_tensor(obj):
58                 count += 1
59                 elements[loc]= torch.numel(obj)
60                 loc += 1
61         elcount = elements.sum(0)
62         print("there are",count,"torch tensors in play with",itp(elcount),"elements")
63         #
64         values,indices = torch.sort(elements,descending = True)
65         upper = 5
66         if upper > count:

```

```

60         upper = count
61     for i in range(upper):
62         indi = indices[i]
63         obji = allobjects[indi]
64         print(obji.size())
65     print("|||")
66     for obj in gc.garbage:
67         if torch.is_tensor(obj):
68             print(type(obj), obj.size())
69     return
70
71
72

```

```

1 def arangeic(x):
2     ar = torch.arange(x,dtype = torch.int64,device = Dvc)
3     return ar
4
5 def itp(x): # integer to print
6     return nump(x)
7
8 def itt(x): # integer to torch
9     if torch.is_tensor(x):
10        return x
11    else:
12        return torch.tensor(x,device = Dvc)
13
14 def itf(x): # integer to torch.float
15     return itt(x).to(torch.float)
16
17 torch_pi = torch.acos(torch.zeros(1)).item() * 2
18
19 def tdetach(x):
20     if torch.is_tensor(x):
21         return x.detach()
22     else:
23         return x
24
25 def nump(x):
26     if torch.is_tensor(x):
27         return x.detach().to(CpuDvc).numpy()
28     else:
29         return x
30
31 def numpr(x,k):
32     return np.round(nump(x),k)
33
34 def numpi(x):
35     return nump(x.to(torch.int))
36
37

```

```
1 ####
```

```
1 class Historical :
2     def __init__(self,hlength_max):
3         self.hlength_max = hlength_max
4         self.hwidth = 20
5         self.hfwidth = 10
6         self.prwidth = 20
7         #
8         self.hlength = 0
9         #
10        self.histi = torch.zeros((self.hlength_max,self.hwidth),dtype = torch.in
11        self.histf = torch.zeros((self.hlength_max,self.hfwidth),dtype = torch.f
12        #
13        self.proofrecord = torch.zeros((self.hlength_max,self.prwidth),dtype = t
14        self.prcursor = 0
15        self.local_tweak_cursor = 0
16        self.global_tweak_cursor = 0
17        #
18        self.current_proof_valency_frequency = torch.zeros((10),dtype = torch.in
19        self.current_proof_impossible_count = 0
20        self.current_proof_done_count = 0
21        self.current_proof_passive_count = 0
22        self.current_proof_benchmark = 0
23        #
24        self.title_text_sigma_proof = None
25        self.title_text_sigma_train = None
26        #
27        self.training_counter = 0
28        #
29        self.proof_nodes_max = 200000
30        #
31        self.D = {
32            'Global':0,
33            'Local':1,
34            'LocalCE':2,
35            'Benchmark':3,
36            'Regular':4,
37            'Adaptive':5,
38            'Uniform':6,
39            'Parameters':7,
40            'Driver':8,
41            'Model':9,
42            'Loss':10,
43            'Training':11,
44            'BenchmarkProof':12,
45            'FullProof':13,
46            'DropoutProof':14,
47        }
48
49
50
51        def reset_current_proof(self):
52            self.current_proof_valency_frequency[:] = 0
53            self.current_proof_impossible_count = 0
54            self.current_proof_done_count = 0
```

```

55     self.current_proof_passive_count = 0
56     self.current_proof_benchmark = 0
57     return
58
59
60     def record_current_proof(self,benchmark = False):
61         if self.prcursor >= self.hlength_max:
62             print("proof data recording overflow")
63             return
64         self.proofrecord[self.prcursor,0] = self.current_proof_impossible_count
65         self.proofrecord[self.prcursor,1] = self.current_proof_done_count
66         self.proofrecord[self.prcursor,2] = self.current_proof_passive_count
67         self.proofrecord[self.prcursor,3:13] = self.current_proof_valency_freque
68         self.proofrecord[self.prcursor,14] = 0
69         if benchmark:
70             self.proofrecord[self.prcursor,14] = 1
71             print("recorded benchmark proof",end=' ')
72         else:
73             print("recorded full proof",end=' ')
74         self.print_proof_recordi(self.prcursor,Pp)
75         self.prcursor += 1
76         return
77
78     def print_proof_recordi(self,i,Pp):
79         #
80         uperval = Pp.beta + 2
81         if uperval > 10:
82             uperval = 10
83         impcount = itp(self.proofrecord[i,0])
84         donecount = itp(self.proofrecord[i,1])
85         passivecount = itp(self.proofrecord[i,2])
86         valency = nump(self.proofrecord[i,3:3 + uperval])
87         #
88         print(". done",donecount,"impossible",impcount,"passive",passivecount,"b
89         return
90
91     def print_proof_records(self,Pp):
92         #
93         ###
94         if Pp.profile_filter_on:
95             prof_filt = 'on'
96         else:
97             prof_filt = 'off'
98         if Pp.halfones_filter_on:
99             ho_filt = 'on'
100        else:
101            ho_filt = 'off'
102        bl_iter = Pp.basicloop_iterations
103        bl_train = Pp.basicloop_training_iterations
104        #
105        global_p = itp(Pp.global_params)
106        local_p = itp(Pp.local_params)
107        ###
108        #
109        print("-----")

```

```

110     print("proof records for a,b =",itp(Pp.alpha),itp(Pp.beta),"model with n
111     print(F'with {bl_iter} basic loops per proof and {bl_train} training seg
112     print(F'global model has {global_p} and local rank+score model has {loca
113     print("-----")
114     proof_number = 0
115     for i in range(self.prcursor):
116         if self.proofrecord[i,14] > 0:
117             print("benchmark proof",end = ' ')
118         else:
119             print("proof",itp(proof_number),end=' ')
120             proof_number += 1
121             self.print_proof_recordi(i,Pp)
122     print("-----")
123     return
124
125
126
127     def noislevel(self,P,count_tensor):
128         counterf = count_tensor.to(torch.float)
129         counter_period_units = counterf / P.noise_period
130         phase = counter_period_units * 2 * torch_pi
131         one_plus_cos_over_two = (torch.cos(phase) +1.)/2
132         decay = P.noise_decay ** counter_period_units
133         level = P.noise_level * one_plus_cos_over_two * decay
134         return level
135
136
137     def reset(self):
138         self.histi[:,:] = 0
139         self.histf[:,:] = 0.
140         self.hlength = 0
141         self.training_counter = 0
142         self.prcursor = 0
143         self.local_tweak_cursor = 0
144         self.global_tweak_cursor = 0
145         print("reinitialized history")
146         return
147
148     def increment(self):
149         if self.hlength >= self.hlength_max:
150             print("Historical at maximum length, can't add any new entries")
151             raise CoherenceError("exiting")
152         cursor = self.hlength
153         self.hlength += 1
154         assert 0 <= cursor < self.hlength_max
155         return cursor
156
157     def record_parameters(self,alpha,beta):
158         cursor = self.increment()
159         self.histi[cursor,0] = self.D['Parameters']
160         self.histi[cursor,1] = alpha
161         self.histi[cursor,2] = beta
162         return
163
164     def record_driver(self,alpha,beta):

```

```
165     cursor = self.increment()
166     self.histi[cursor,0] = self.D['Driver']
167     self.histi[cursor,1] = alpha
168     self.histi[cursor,2] = beta
169     return
170
171     def record_model(self,n):
172         cursor = self.increment()
173         self.histi[cursor,0] = self.D['Model']
174         self.histi[cursor,1] = n
175         return
176
177
178     def record_loss(self,style,L1_loss,MSE_loss):
179         cursor = self.increment()
180         self.histi[cursor,0] = self.D['Loss']
181         if style != 'global' and style != 'local' and style != 'local_ce':
182             raise CoherenceError("unsupported style in record_loss")
183         if style == 'global':
184             self.histi[cursor,1] = self.D['Global']
185         if style == 'local':
186             self.histi[cursor,1] = self.D['Local']
187         if style == 'local_ce':
188             self.histi[cursor,1] = self.D['LocalCE']
189         if torch.is_tensor(MSE_loss):
190             MSE_loss_detach = MSE_loss.detach()
191         else:
192             MSE_loss_detach = MSE_loss
193         self.histf[cursor,0] = L1_loss.detach()
194         self.histf[cursor,1] = MSE_loss_detach
195         #
196         self.training_counter += 1
197         return
198
199
200     def record_training(self,style,iterations,explore_pre_pool,example_pre_pool,
201         cursor = self.increment()
202         #
203         self.histi[cursor,0] = self.D['Training']
204         if style != 'global' and style != 'local':
205             raise CoherenceError("unsupported style in record_training")
206         if style == 'global':
207             self.histi[cursor,1] = self.D['Global']
208         if style == 'local':
209             self.histi[cursor,1] = self.D['Local']
210         self.histi[cursor,2] = iterations
211         self.histi[cursor,3] = explore_pre_pool
212         self.histi[cursor,4] = example_pre_pool
213         self.histi[cursor,5] = example_pool
214         return
215
216     def record_full_proof(self,M,steps,cumulative_nodes,done_nodes):
217         cursor = self.increment()
218         #
219         if M.benchmark:
220             self.histi[cursor,0] = self.D['BenchmarkProof']
```

```

220         self.histi[cursor,0] = self.D[ 'BenchmarkProof' ]
221     else:
222         self.histi[cursor,0] = self.D[ 'FullProof' ]
223     self.histi[cursor,1] = steps
224     self.histi[cursor,2] = cumulative_nodes
225     self.histi[cursor,3] = done_nodes
226     return
227
228
229 def record_dropout_proof(self,style,dropout,steps,ECN):
230     cursor = self.increment()
231     #
232     if style != 'regular' and style != 'adaptive' and style != 'uniform':
233         raise CoherenceError("unsupported style in record_dropout_proof")
234     #
235     self.histi[cursor,0] = self.D[ 'DropoutProof' ]
236     if style == 'regular':
237         self.histi[cursor,1] = self.D[ 'Regular' ]
238     if style == 'adaptive':
239         self.histi[cursor,1] = self.D[ 'Adaptive' ]
240     if style == 'uniform':
241         self.histi[cursor,1] = self.D[ 'Uniform' ]
242     self.histi[cursor,2] = dropout
243     self.histi[cursor,3] = steps
244     ecnr = torch.round(ECN).to(torch.int64)
245     self.histi[cursor,4] = ecnr
246     return
247
248
249 def print_history(self):
250     length = self.hlength
251     print("-- -- -- -- -- -- -- -- -- -- -- -- -- -- --")
252     print("    printing history of length",itp(length))
253     print("-- -- -- -- -- -- -- -- -- -- -- -- -- -- --")
254     for cursor in range(length):
255         tag = self.histi[cursor,0]
256         a = itp(self.histi[cursor,1])
257         b = itp(self.histi[cursor,2])
258         c = itp(self.histi[cursor,3])
259         d = itp(self.histi[cursor,4])
260         e = itp(self.histi[cursor,5])
261         f = itp(self.histi[cursor,6])
262         #
263         x = numpr(self.histf[cursor,0],3)
264         y = numpr(self.histf[cursor,1],3)
265         #
266         print("(" ,cursor,")--",end=' ')
267         #
268         if tag == self.D[ 'Parameters' ]:
269             print("setting parameters for alpha=",a,"beta=",b)
270         #
271         if tag == self.D[ 'Driver' ]:
272             print("initialize driver for alpha=",a,"beta=",b)
273         #
274         if tag == self.D[ 'Model' ]:
275             print("initialize model with n =",a)

```

```

276     #
277     if tag == self.D['Loss']:
278         if a == self.D['Global']:
279             print("test global model, L1 loss",x,"MSE loss",y)
280         if a == self.D['Local']:
281             print("test local model, L1 loss",x,"MSE loss",y)
282         if a == self.D['LocalCE']:
283             print("test local model, CE loss",x)
284     #
285     if tag == self.D['Training']:
286         if a == self.D['Global']:
287             print("training global model",end=' ')
288         if a == self.D['Local']:
289             print("training local model",end=' ')
290         print("iterations",b,"explore prepool",c,"example prepool",d,"ex
291     #
292     if tag == self.D['BenchmarkProof']:
293         print("BENCHMARK PROOF in",a,"steps",b,"cumulative nodes",c,"don
294     #
295     if tag == self.D['FullProof']:
296         print("FULL PROOF in",a,"steps",b,"cumulative nodes",c,"done lea
297     #
298     if tag == self.D['DropoutProof']:
299         print("proof with dropout style",end='')
300         if a == self.D['Regular']:
301             print(" regular ",end='')
302         if a == self.D['Adaptive']:
303             print(" adaptive ",end='')
304         if a == self.D['Uniform']:
305             print(" uniform ",end='')
306         print("threshold",b,"in",c,"steps with estimated cumulative node
307     #
308     print("-- -- -- -- -- -- -- -- -- -- -- -- -- -- -- --")
309     print("      end printing history of length",itp(length))
310     print("-- -- -- -- -- -- -- -- -- -- -- -- -- -- -- --")
311     #
312     return
313
314
315
316 def graph_history(self,P,style):
317     #
318     alpha = P.alpha
319     beta = P.beta
320     nu = P.model_n
321     #
322     ###
323     if P.profile_filter_on:
324         prof_filt = 'on'
325     else:
326         prof_filt = 'off'
327     if P.halfones_filter_on:
328         ho_filt = 'on'
329     else:
330         ho_filt = 'off'

```

```

331     bl_iter = P.basicloop_iterations
332     bl_train = P.basicloop_training_iterations
333     #
334     global_p = itp(P.global_params)
335     local_p = itp(P.local_params)
336     ###
337     plotcount = 0
338     for cursor in range(self.hlength):
339         tag = self.histi[cursor,0]
340         if tag == self.D['FullProof']:
341             plotcount += 1
342     baseline = 0
343     ecn_graph = torch.zeros((plotcount),dtype = torch.int64,device=Dvc)
344     attempts = arangeic(plotcount)
345     attempt_number = 0
346     for cursor in range(self.hlength):
347         tag = self.histi[cursor,0]
348         b = self.histi[cursor,2]
349         if tag == self.D['BenchmarkProof']:
350             baseline = b
351         if tag == self.D['FullProof']:
352             ecn_graph[attempt_number] = b
353             attempt_number += 1
354     ecn_graph = torch.clamp(ecn_graph,0,self.proof_nodes_max)
355     plt.clf()
356     if style == 'big':
357         plt.figure(figsize = (17,8))
358     else:
359         plt.figure(figsize = (8,4))
360     ###
361     phrasel = F'Proofs for a= {alpha}, b={beta} for model with n= {nu} and h
362     phrase2 = F'with {bl_iter} basic loops per proof and {bl_train} training
363     phrase3 = F'global model has {global_p} and local rank+score model has {
364     plt.title(phrasel + '\n' + phrase2 + '\n' + phrase3)
365     ###
366     plt.xlabel('number of training rounds')
367     plt.ylabel('cumulative nodes')
368     plt.plot([0,plotcount - 1],[itp(baseline),itp(baseline)],'deepskyblue')
369     plt.plot(nump(attempts),nump(ecn_graph),'.-')
370     plt.show()
371     #
372     pcg = 0
373     pcl = 0
374     for cursor in range(self.hlength):
375         tag = self.histi[cursor,0]
376         a = self.histi[cursor,1]
377         if tag == self.D['Loss']:
378             if a == self.D['Global']:
379                 pcg += 1
380             if a == self.D['Local']:
381                 pcl += 1
382             if a == self.D['LocalCE']:
383                 pcl += 1
384     Llgraph_local = torch.zeros((pcl),dtype = torch.float,device=Dvc)
385     MSEgraph_local = torch.zeros((pcl),dtype = torch.float,device=Dvc)

```

```

386 CEgraph_local = torch.zeros((pcl),dtype = torch.float,device=Dvc)
387 Llgraph_global = torch.zeros((pcg),dtype = torch.float,device=Dvc)
388 MSEgraph_global = torch.zeros((pcg),dtype = torch.float,device=Dvc)
389 measurements_local = arangeic(pcl)
390 measurements_global = arangeic(pcg)
391 measurement_number_local = 0
392 measurement_number_global = 0
393 for cursor in range(self.hlength):
394     tag = self.histi[cursor,0]
395     a = self.histi[cursor,1]
396     x = self.histf[cursor,0]
397     y = self.histf[cursor,1]
398     if tag == self.D['Loss']:
399         if a == self.D['Global']:
400             Llgraph_global[measurement_number_global] = x
401             MSEgraph_global[measurement_number_global] = y
402             measurement_number_global += 1
403         if a == self.D['Local']:
404             Llgraph_local[measurement_number_local] = x
405             MSEgraph_local[measurement_number_local] = y
406             measurement_number_local += 1
407         if a == self.D['LocalCE']:
408             CEgraph_local[measurement_number_local] = x
409             measurement_number_local += 1
410 Llavg_global = (Llgraph_global[0:pcg-2] + Llgraph_global[1:pcg-1] + Llgr
411 Llavg_global = torch.clamp(Llavg_global,0.,0.2)
412 Llavg_local = (Llgraph_local[0:pcl-2] + Llgraph_local[1:pcl-1] + Llgraph
413 #
414 Llavg_local_red = Llavg_local /2. # so it fits on the graph better, wit
415 #
416 Llavg_local_red = torch.clamp(Llavg_local_red,0.,0.2)
417 MSEavg_global = (MSEgraph_global[0:pcg-2] + MSEgraph_global[1:pcg-1] + M
418 MSEavg_global = torch.clamp(MSEavg_global,0.,0.2)
419 MSEavg_local = (MSEgraph_local[0:pcl-2] + MSEgraph_local[1:pcl-1] + MSEg
420 MSEavg_local = torch.clamp(MSEavg_local,0.,0.2)
421 CEavg_local = (CEgraph_local[0:pcl-2] + CEgraph_local[1:pcl-1] + CEgraph
422 CEavg_local = CEavg_local / 10.
423 CEavg_local = torch.clamp(CEavg_local,0.,0.2)
424 #
425 #
426 noislevel = HST.noislevel(P,measurements_global)
427 #
428 plt.clf()
429 if style == 'big':
430     plt.figure(figsize = (17,8))
431 else:
432     plt.figure(figsize = (8,4))
433 ###
434 phraselb = F'Training for a= {alpha}, b={beta} for model with n= {nu}, {
435 # phrase 2 is the same as before
436 plt.title(phraselb + '\n' + phrase2 + '\n' + phrase3)
437 ###
438 plt.xlabel('training')
439 plt.ylabel('loss')
440 #

```

```

441 plt.plot(nump(measurements_local[5:pc1]),numpr(L1avg_local_red[3:pc1-2],
442 plt.plot(nump(measurements_global[5:pcg]),numpr(L1avg_global[3:pcg-2],4)
443 #
444 plt.plot(nump(measurements_local[5:pc1]),numpr(MSEavg_local[3:pc1 - 2],5)
445 plt.plot(nump(measurements_global[5:pcg]),numpr(MSEavg_global[3:pcg - 2]
446 #
447 plt.plot(nump(measurements_global[5:pcg]),numpr(noiselevel[3:pcg-2],5),1)
448 #
449 plt.legend()
450 plt.show()
451 ###
452 self.print_proof_records(P)
453 return
454
455
456
457
458
459
460
461
462
463

```

```
1 ###
```

```

1 class SymmetricGroup :
2     def __init__(self,p):
3         #
4         if p < 1:
5             print("can't initialize a symmetric group with size",p)
6             raise CoherenceError("exiting")
7         if p > 9:
8             print("symmetric group size",p,"is probably going to cause a memory
9             raise CoherenceError("exiting")
10        #
11        self.p = p
12        #self.subgroups_max = subgroups_max # this is not currently used
13        #
14        self.gtlength = 1
15        for i in range(self.p):
16            self.gtlength *= (i+1)
17        #
18        self.grouptable = self.makegrouptable()
19        self.gtbinary = self.makegrouptablebinary()
20        #self.multiplicationtable = self.makemult()
21        #self.inverse = self.makeinverse()
22        self.inversetable = self.makeinversetable()
23        #
24
25
26    def symmetricgrouptable(self,k):
27        assert k > 0
28        if k == 1:

```

```

29     sgt = torch.zeros((1),dtype = torch.int64,device = Dvc)
30     return 1,sgt
31     length_prev,sgtprev = self.symmetricgrouptable(k-1)
32     length = length_prev * k
33     krange = torch.arange((k),dtype = torch.int64,device=Dvc) # same as ara
34     krangevx = krange.view(k,1).expand(k,length_prev)
35     krangevx2 = krange.view(k,1,1).expand(k,length_prev,k-1)
36     #
37     sgtprev_vx = sgtprev.view(1,length_prev,k-1).expand(k,length_prev,k-1)
38     #
39     krangelvvr = krange.view(k,1).expand(k,k).reshape(k*k)
40     krange2vvr = krange.view(1,k).expand(k,k).reshape(k*k)
41     gappedtablev = krange2vvr[(krangelvvr != krange2vvr)]
42     gappedtable = gappedtablev.view(k,k-1)
43     #
44     afterpart = gappedtable[krangevx2,sgtprev_vx]
45     beforepart = krange.view(k,1,1).expand(k,length_prev,1)
46     newtablev = torch.cat((beforepart,afterpart),2)
47     newtable = newtablev.view(length,k)
48     return length,newtable
49
50     def makegrouptable(self):
51         length,table = self.symmetricgrouptable(self.p)
52         assert length == self.gtlength
53         #print("making group table for symmetric group, as an array of shape",ta
54         return table
55
56
57     def findpermutation(self,batchlength,vector):
58         vectorvx = vector.view(batchlength,1,self.p).expand(batchlength,self.gtl
59         grouptablevx = self.grouptable.view(1,self.gtlength,self.p).expand(batch
60         detection = (vectorvx == self.grouptable).all(2)
61         values,permutation = torch.max((detection.to(torch.int)),1)
62         assert (values == 1).all(0)
63         return permutation
64
65
66     def makemult(self):
67         if self.p > 7:
68             print("multiplication table for symmetric group of size",self.p,"would
69             raise CoherenceError("exiting")
70             print("setting up multiplication table...",end=' ')
71             mult = torch.zeros((self.gtlength,self.gtlength),dtype = torch.int64,dev
72             for x in range(self.gtlength):
73                 xvector = self.grouptable[x]
74                 comtable = xvector[self.grouptable]
75                 mult[x,:] = self.findpermutation(self.gtlength,comtable)
76             print("done")
77             return mult
78
79     def makeinverse(self):
80         invdetection = (self.multiplicationtable == 0)
81         values,inverse = torch.max((invdetection.to(torch.int)),1)
82         return inverse
83

```

```

84     def makeinversetable(self):
85         gl = self.gtlength
86         p=self.p
87         tablevx = self.grouptable.view(gl,p,1).expand(gl,p,p)
88         yrangevx = arangeic(p).view(1,1,p).expand(gl,p,p)
89         delta = (tablevx == yrangevx).to(torch.int64)
90         values,inversetable = torch.max(delta,1)
91         return inversetable
92
93
94
95     #####@ for the list of subgroups #####
96
97     def subgroupgen(self,thesubgroup,thex): # outputs the subgroup generated by
98         currentsubset = torch.zeros((self.gtlength),dtype = torch.bool,device=Dv
99         currentsubset[thesubgroup] = True
100        currentsubset[thex] = True
101        for i in range(1000):
102            currentlength = currentsubset.to(torch.int).sum(0).clone()
103            cl2 = currentlength * currentlength
104            #print("current length",itp(currentlength))
105            mtcurent1 = self.multiplicationtable[currentsubset]
106            mtcurent1p = mtcurent1.permute(1,0)
107            mtcurent2 = mtcurent1p[currentsubset]
108            mtcurent2vx = mtcurent2.view(1,cl2).expand(self.gtlength,cl2)
109            grouparangevx = arangeic(self.gtlength).view(self.gtlength,1).expand
110            products = (grouparangevx == mtcurent2vx).any(1)
111            currentsubset = currentsubset | products
112            newlength = currentsubset.to(torch.int).sum(0)
113            if newlength == currentlength:
114                #print("break")
115                break
116        return currentsubset
117
118     def findsubgroup(self,thesubgroup):
119         currentsglist = self.subgroup[0:self.sglistlength,:]
120         thesubgroupvx = thesubgroup.view(1,self.gtlength).expand(self.sglistleng
121         findsg = (currentsglist == thesubgroupvx).all(1)
122         if findsg.any(0):
123             assert findsg.to(torch.int).sum(0) == 1
124             sgrange = arangeic(self.sglistlength)
125             sgnumber = itp(sgrange[findsg][0])
126             return True,sgnumber
127         else:
128             return False, None
129
130
131     def addnextsubgroup(self):
132         for k in range(self.sglistlength):
133             thesubgroup = self.subgroup[k]
134             #print("try subgroup",k)
135             for x in range(self.gtlength):
136                 if not thesubgroup[x]:
137                     #print("try x=",x)
138                     ssgenx = self.subgroupgen(thesubgroup,x)

```

```

139         fsg,sgnumber = self.findsubgroup(sggenx)
140         if not fsg:
141             self.subgroup[self.sglistlength] = sggenx
142             self.sgsize[self.sglistlength] = sggenx.to(torch.int).su
143             #print("add subgroup",itp(self.sglistlength),"of length"
144             self.sglistlength += 1
145             return True
146     return False
147
148     def createsubgrouplist(self):
149         # the identity
150         self.sglistlength = 1
151         self.subgroup.masked_fill_(truetensor,False)
152         self.sgsize.masked_fill_(truetensor,0)
153         self.sgsize[0] = 1
154         self.subgroup[0,0] = True
155         for i in range(self.subgroups_max - 1):
156             ansg = self.addnextsubgroup()
157             if not ansg:
158                 break
159         print("created a list of",itp(self.sglistlength),"subgroups")
160         return
161
162
163     def findsubgroupbatch(self,batchsize,sgbatch):
164         currentsglist = self.subgroup[0:self.sglistlength,:]
165         currentsglistvx = currentsglist.view(1,self.sglistlength,self.gtlength).
166         sgbatchvx = sgbatch.view(batchsize,1,self.gtlength).expand(batchsize,sel
167         findsg = (currentsglist == thesubgroupvx).all(2)
168         #
169         assert(findsg.to(torch.int).sum(1) == 1).all(0)
170         #
171         sglistarangevx = arangeic(self.sglistlength).view(1,self.sglistlength).e
172         sglistarangevxv = sglistarangevx.reshape(batchsize*self.sglistlength)
173         findsgv = findsg.reshape(batchsize*self.sglistlength)
174         output = sglistarangevxv[findsgv]
175         return output
176
177     def makegrouptablebinary(self):
178         p = self.p
179         gl = self.gtlength
180         if p > 7:
181             print("warning: not making binary table for p=",itp(p),"> 7")
182             return None
183         blength = 2**p
184         brange = arangeic(blength)
185         zbinarytable = torch.zeros((blength,p),dtype = torch.bool,device=Dvc)
186         for z in range(blength):
187             zbinarytable[z,:] = zbinary(p,z)
188         gtb = self.grouptable.view(gl,1,p).expand(gl,blength,p).reshape(gl*bleng
189         brange = arangeic(blength).view(1,blength,1).expand(gl,blength,p).reshap
190         #
191         gtb_mod = zbinarytable[brange,gtb]
192         #
193         gt_binaryv = binaryzbatch(gl*blength,p,gtb_mod)
194         #

```

```

194 gt_binary = gt_binary.view(g1,blength)
195 #print("made group table binary")
196 return gt_binary
197
198
199
200

```

```

1 ### this is the cell where the neural networks are created. We include input and
2 ### template assertions in case one wants to experiment different network archit
3 ###
4
5 class PrepareInputLayer(nn.Module):
6
7     def __init__(self,pp):
8         super(PrepareInputLayer, self).__init__()
9         self.pp = pp
10        self.a = pp.alpha
11        self.b = pp.beta
12        self.bz = self.b + 1
13        #
14        self.n = self.pp.model_n
15        #
16        a=self.a
17        bz=self.bz
18        self.channels = 5*bz + 2*a
19        #
20
21
22    def forward(self,Data):
23        #
24        a = self.a
25        b = self.b
26        bz = self.bz
27        #
28        length = Data['length']
29        prod = Data['prod']
30        left = Data['left']
31        right = Data['right']
32        ternary = Data['ternary']
33        #
34        #####
35        # input template assertions:
36        #
37        assert prod.dtype == torch.bool
38        assert left.dtype == torch.bool
39        assert right.dtype == torch.bool
40        assert ternary.dtype == torch.bool
41        #
42        assert prod.size() == torch.Size([length,a,a,bz])
43        assert left.size() == torch.Size([length,a,bz,2])
44        assert right.size() == torch.Size([length,bz,a,2])
45        assert ternary.size() == torch.Size([length,a,a,a,2])
46        #
47        #####

```

```

48     #
49     prod_data = prod.permute(0,3,1,2).view(length,bz,a,a)
50     left_data = left.permute(0,3,2,1).reshape(length,2,bz,a,1).expand(length
51     right_data = right.permute(0,3,1,2).reshape(length,2,bz,1,a).expand(leng
52     ternary_data = ternary.permute(0,4,2,1,3).reshape(length,2,a,a,a)
53     with torch.no_grad():
54         prod_f = prod_data.float()
55         prod_denom = prod_f.sum(1).view(length,1,a,a).expand(length,bz,a,a)
56         prod_denom = torch.clamp(prod_denom,1.,100.)
57         prod_ren = prod_f / prod_denom
58         prod_ren = (bz * prod_ren) - 1.
59         #
60         left_f = left_data.float()
61         left_denom = left_f.sum(1).view(length,1,bz,a,a).expand(length,2,bz,
62         left_denom = torch.clamp(left_denom,1.,100.)
63         left_ren = (left_f / left_denom).view(length,2*bz,a,a)
64         left_ren = left_ren - 0.5
65         #
66         right_f = right_data.float()
67         right_denom = right_f.sum(1).view(length,1,bz,a,a).expand(length,2,b
68         right_denom = torch.clamp(right_denom,1.,100.)
69         right_ren = (right_f / right_denom).view(length,2*bz,a,a)
70         right_ren = right_ren - 0.5
71         #
72         ternary_f = ternary_data.float()
73         ternary_denom = ternary_f.sum(1).view(length,1,a,a,a).expand(length,
74         ternary_denom = torch.clamp(ternary_denom,1.,100.)
75         ternary_ren = (ternary_f / ternary_denom).reshape(length,2*a,a,a)
76         ternary_ren = ternary_ren - 0.5
77         #
78         initial_data = torch.cat((prod_ren,left_ren,right_ren,ternary_ren),1
79     #
80     assert initial_data.size() == torch.Size([length,self.channels,a,a])
81     #
82     return initial_data, prod_data
83
84
85
86 class OutputLayerScalar(nn.Module):
87
88     def __init__(self,pp,channels_in,channels_mid):
89         super(OutputLayerScalar, self).__init__()
90         self.pp = pp
91         self.a = self.pp.alpha
92         #
93         self.channels_in = channels_in
94         self.channels_mid = channels_mid
95         #
96         self.lrl = nn.LeakyReLU()
97         #
98         self.layerD1 = nn.Linear(channels_in,channels_mid,1)
99         self.layerD2 = nn.Linear(channels_mid,channels_mid,1)
100        self.layerD3 = nn.Linear(2*channels_mid,1,1)
101
102

```

```

103     def forward(self, layer_data):
104         #
105         length = layer_data.size()[0]
106         #
107         layer_in = layer_data.view(length, self.channels_in)
108         yD1 = self.lrl(self.layerD1(layer_in))
109         yD2 = self.lrl(self.layerD2(yD1))
110         yD3 = self.layerD3(torch.cat((yD1, yD2), 1))
111         #
112         yScore = yD3.view(length)
113         #
114         return yScore
115
116 class OutputLayer2d(nn.Module):
117
118     def __init__(self, pp, channels_array, channels_mid, channels_extra):
119         super(OutputLayer2d, self).__init__()
120         self.pp = pp
121         self.a = self.pp.alpha
122         #
123         self.channels_array = channels_array
124         self.channels_in = self.channels_array * self.a * self.a
125         self.channels_mid = channels_mid
126         self.channels_extra = channels_extra
127         #
128         self.lrl = nn.LeakyReLU()
129         #
130         self.layerD1 = nn.Linear(self.channels_in, channels_mid, 1)
131         self.layerD2 = nn.Linear(channels_mid, channels_mid, 1)
132         self.layerD3 = nn.Linear(2*channels_mid, channels_extra * self.a*self.a, 1)
133         #
134         self.layerD4 = nn.Conv2d(self.channels_array + self.channels_extra, self.a, 1)
135         self.layerD5 = nn.Conv2d(self.channels_mid, self.channels_mid, 1)
136         self.layerD6 = nn.Conv2d(2*self.channels_mid + self.channels_extra, 1, 1)
137
138     def forward(self, layer_data):
139         #
140         length = layer_data.size()[0]
141         #
142         layer_in = layer_data.view(length, self.channels_in)
143         yD1 = self.lrl(self.layerD1(layer_in))
144         yD2 = self.lrl(self.layerD2(yD1))
145         yD3 = self.layerD3(torch.cat((yD1, yD2), 1))
146         #
147         yD3v = yD3.view(length, self.channels_extra, self.a, self.a)
148         layer_array = layer_data.view(length, self.channels_array, self.a, self.a)
149         yDcat = torch.cat((yD3v, layer_array), 1)
150         yD4 = self.lrl(self.layerD4(yDcat))
151         yD5 = self.lrl(self.layerD5(yD4))
152         yD6 = self.layerD6(torch.cat((yD3v, yD4, yD5), 1))
153         #
154         yScore = yD6.view(length, self.a, self.a)
155         #
156         return yScore
157

```

```

158
159
160
161
162
163
164 class SGNetProcess(nn.Module):
165
166     def __init__(self,pp):
167         super(SGNetProcess, self).__init__()
168         #
169         self.pp = pp
170         self.a = self.pp.alpha
171         self.bz = self.pp.betaz
172         #
173         #
174         self.lrl = nn.LeakyReLU()
175         #
176         self.prep = PrepareInputLayer(self.pp)
177         #
178         self.channels = self.prep.channels
179         #
180         self.n = self.pp.model_n
181         n = self.n
182         #
183         self.array_channels = n
184         self.process_channels = self.array_channels*self.a*self.a
185         #
186         self.convA1 = nn.Conv2d(self.channels,8*n,1)
187         self.convA2 = nn.Conv2d(8*n,8*n,[5,1],padding = [2,0],padding_mode = 'ci
188         self.convA3 = nn.Conv2d(8*n,8*n,[1,5],padding = [0,2],padding_mode = 'ci
189         self.convA4 = nn.Conv2d(8*n,8*n,[5,1],padding = [2,0],padding_mode = 'ci
190         self.convA5 = nn.Conv2d(8*n,8*n,[1,5],padding = [0,2],padding_mode = 'ci
191         self.convA5tg = nn.Conv2d(40*n,8*n,1)
192         self.convA6 = nn.Conv2d(8*n,8*n,[5,1],padding = [2,0],padding_mode = 'ci
193         self.convA7 = nn.Conv2d(9*n,8*n,[1,5],padding = [0,2],padding_mode = 'ci
194         self.convA8 = nn.Conv2d(8*n,8*n,[5,1],padding = [2,0],padding_mode = 'ci
195         self.convA9 = nn.Conv2d(8*n,8*n,[1,5],padding = [0,2],padding_mode = 'ci
196         #
197         self.convB = nn.Conv2d(40*n,n,1)
198         #
199         self.convC1 = nn.Conv1d(8*n*self.a*self.a,8*n,1,groups=8*n)
200         self.convC2 = nn.Conv1d(8*n,n*self.a*self.a,1,groups = n)
201         #
202         ##
203
204     def forward(self,Data):
205         #
206         initial_data,prod_data = self.prep(Data)
207         length = Data['length']
208         n = self.n
209         #
210         yA1 = self.lrl(self.convA1(initial_data))
211         yA2 = self.lrl(self.convA2(yA1))
212         yA3 = self.lrl(self.convA3(yA2))

```

```

213     yA4 = self.lrl(self.convA4(yA3))
214     yA5 = self.lrl(self.convA5(yA4))
215     yA5tg = self.lrl(self.convA5tg(torch.cat((yA1,yA2,yA3,yA4,yA5),1)))
216     yA6 = self.lrl(self.convA6(yA5tg))
217     #
218     yA4side = yA4.view(length,8*n*self.a*self.a,1)
219     yC1 = self.lrl(self.convC1(yA4side))
220     yC2 = self.lrl(self.convC2(yC1)).view(length,n,self.a,self.a)
221     yA6side = torch.cat((yA6,yC2),1)
222     #
223     yA7 = self.lrl(self.convA7(yA6side))
224     yA8 = self.lrl(self.convA8(yA7))
225     yA9 = self.lrl(self.convA9(yA8))
226     #
227     yB = self.lrl(self.convB(torch.cat((yA1,yA3,yA5tg,yA7,yA9),1)))
228     #
229     yProcessed = yB.view(length,self.process_channels)
230     #
231     return yProcessed
232
233
234 class SGNetGlobal(nn.Module):
235
236     def __init__(self,pp):
237         super(SGNetGlobal, self).__init__()
238         #
239         self.pp = pp
240         self.a = self.pp.alpha
241         #
242         self.process = SGNetProcess(self.pp)
243         #
244         self.outlayer = OutputLayerScalar(self.pp,self.process.process_channels,
245
246
247     def forward(self,Data):
248         #
249         # see the PrepareInputLayer() class above for the input template asserti
250         #
251         yProcessed = self.process(Data)
252         #
253         yScore = self.outlayer(yProcessed)
254         #
255         #####
256         # output template assertions:
257         length = Data['length']
258         assert yScore.dtype == torch.float
259         assert yScore.size() == torch.Size([length])
260         #####
261         #
262         return yScore
263
264
265
266
267 class SGNetLocal(nn.Module):
268

```

```

269     def __init__(self,pp):
270         super(SGNetLocal, self).__init__()
271         # an affine operation: y = Wx + b
272         #
273         self.pp = pp
274         self.a = self.pp.alpha
275         #
276         self.process = SGNetProcess(self.pp)
277         #
278         self.outlayer = OutputLayer2d(self.pp,self.process.array_channels,32,4)
279
280
281     def forward(self,Data):
282         #
283         # see the PrepareInputLayer() class above for the input template asserti
284         #
285         yProcessed = self.process(Data)
286         #
287         yScore = self.outlayer(yProcessed)
288         #
289         #####
290         # output template assertions:
291         length = Data['length']
292         a = self.a
293         assert yScore.dtype == torch.float
294         assert yScore.size() == torch.Size([length,a,a])
295         #
296         #####
297         #
298         return yScore
299
300 #####
301
302
303
304 #####
305
306
307
308
309 class SgModel :
310     def __init__(self,pp):
311         self.pp = pp
312         #
313         self.network = SGNetGlobal(self.pp).to(Dvc)
314         #
315         self.network2 = SGNetLocal(self.pp).to(Dvc)
316         #
317         self.average_local_loss = itf(1.0)
318         #
319         #print(self.network)
320         print("set up model network and network2")
321         #
322         self.benchmark = False
323         #

```

```

324     self.learning_rate = 0.002 # was 0.002, then 0.003, ...
325     self.momentum = 0.95
326     #self.weight_decay = 0.0001
327     #
328     #self.optimizer = optim.SGD(self.network.parameters(), lr=self.learning_
329     #self.optimizer2 = optim.SGD(self.network2.parameters(), lr=self.learnin
330     self.optimizer = optim.SGD(self.network.parameters(), lr=self.learning_r
331     self.optimizer2 = optim.SGD(self.network2.parameters(), lr=self.learning
332     #
333     self.criterionCE = nn.CrossEntropyLoss()
334     self.criterionA = nn.L1Loss()
335     self.criterionB = nn.MSELoss()
336     #
337     self.network2_trainable = True
338     #
339     pp.global_params, pp.local_params = self.modelcount()
340     #
341     self.softmax = nn.Softmax(dim = 1)
342
343
344     def modelcount(self):
345         network_param = sum(p.numel() for p in self.network.parameters() if p.re
346         print("network parameters",itp(network_param))
347         network2_param = sum(p.numel() for p in self.network2.parameters() if p.
348         print("network2 parameters",itp(network2_param))
349         return network_param, network2_param
350
351     def tweak_network(self,N,density,epsilon):
352         for p in N.parameters():
353             if p.requires_grad:
354                 tirage_density = torch.rand(p.size(),device=Dvc)
355                 modif = torch.rand(p.size(),device=Dvc)
356                 modif *= (tirage_density < density).to(torch.float) * epsilon
357                 factor = modif + 1.0
358                 with torch.no_grad():
359                     p *= factor
360         return
361
362
363
364
365
366     def save_model(self,filename): # tries to save the two model state dicts an
367     # I haven't tried these but they should probably mostly work and are inc
368     torch.save({
369         'network_state_dict': self.network.state_dict(),
370         'network2_state_dict': self.network2.state_dict(),
371         'optimizer_state_dict': self.optimizer.state_dict(),
372         'optimizer2_state_dict': self.optimizer2.state_dict(),
373     }, filename)
374     print("saved to",filename)
375     return
376
377     def load_model(self,filename): # tries to load from the file
378     #

```

```

379     loadedmodels = torch.load(filename)
380     network_state_dict = loadedmodels['network_state_dict']
381     network2_state_dict = loadedmodels['network2_state_dict']
382     optimizer_state_dict = loadedmodels['optimizer_state_dict']
383     optimizer2_state_dict = loadedmodels['optimizer2_state_dict']
384     #
385     self.network.load_state_dict(network_state_dict)
386     self.network2.load_state_dict(network2_state_dict)
387     self.optimizer.load_state_dict(optimizer_state_dict)
388     self.optimizer2.load_state_dict(optimizer2_state_dict)
389     #
390     self.network.train()
391     self.network2.train()
392     print("loaded from",filename)
393     return
394
395
396 class ProtoModel :
397     def __init__(self,pp,style):
398         self.pp = pp
399         self.style = style
400         self.a = pp.alpha
401         self.a3z = self.a*self.a*self.a + 1
402         self.b = pp.beta
403         self.bz = self.b + 1
404         #
405         self.random_order = torch.randperm(self.a*self.a)
406         self.spiral, self.spiral_mix = self.makespiral()
407         self.rays = self.makerays()
408         #
409         self.network = SGNetGlobal(self.pp).to(Dvc)
410         # there is no network2
411         self.network2_trainable = False
412         #
413         #print(self.network)
414         print("set up the proto-model network---network2 is not trainable, this
415         #
416         self.benchmark = True
417         #
418         self.learning_rate = 0.002
419         #
420         self.optimizer = optim.SGD(self.network.parameters(), lr=self.learning_r
421         #
422         self.criterionA = nn.L1Loss()
423         self.criterionB = nn.MSELoss()
424         #
425         self.softmax = nn.Softmax(dim = 1)
426
427     def makespiral(self):
428         spiral_order = torch.zeros((self.a,self.a),dtype = torch.int64,device=Dv
429         spiral_order[0,0] = 0
430         count = 1
431         for x in range(1,self.a):
432             spiral_order[x,x] = count
433             count += 1

```

```

434         for y in range(x):
435             spiral_order[x,y] = count
436             count += 1
437             spiral_order[y,x] = count
438             count += 1
439     spiral_orderf = spiral_order.to(torch.float) / itt(self.a*self.a).to(torch.float)
440     thresh = self.pp.spiral_mix_threshold
441     over_thresh = (spiral_order > thresh).view(self.a*self.a)
442     spiral_mix = spiral_order.clone().view(self.a*self.a)
443     spiral_mix[over_thresh] = arangeic(self.a*self.a)[over_thresh] + thresh
444     spiral_mixf = spiral_mix.to(torch.float) / itt(self.a*self.a).to(torch.float)
445     return spiral_orderf, spiral_mixf
446
447     def makerays(self):
448         a = self.a
449         ray_order = torch.zeros((self.a,self.a),dtype = torch.int64,device=Dvc)
450         count = 0
451         for x in range(a):
452             ray_order[x,x] = count
453             count += 1
454         for x in range(a-1):
455             for y in range(x+1,a):
456                 ray_order[x,y] = count
457                 count += 1
458                 ray_order[y,x] = count
459                 count += 1
460         ray_orderf = ray_order.to(torch.float) / itt(a*a).to(torch.float)
461         return ray_orderf
462
463     def virtual_score(self,Data):
464         length = Data['length']
465         if self.style == 'random':
466             output = torch.rand((length,self.a,self.a),device=Dvc)
467         if self.style == 'random_order':
468             output = self.random_order.view(1,self.a,self.a).expand(length,self.a,self.a)
469         if self.style == 'spiral':
470             output = self.spiral.view(1,self.a,self.a).expand(length,self.a,self.a)
471         if self.style == 'spiral_mix':
472             output = self.spiral_mix.view(1,self.a,self.a).expand(length,self.a,self.a)
473         if self.style == 'rays':
474             output = self.rays.view(1,self.a,self.a).expand(length,self.a,self.a)
475         return output
476
477     def network2(self,Data):
478         #
479         a = self.a
480         #
481         length = Data['length']
482         prod = Data['prod']
483         #
484         prodsum = prod.to(torch.int64).sum(3)
485         availablexyv = (prodsum > 1).view(length*a*a)
486         #
487         vsv = self.virtual_score(Data).reshape(length*a*a)
488         #

```

```

489     vsv[~availablexyv] = 100.
490     #
491     values,xyvector = torch.min(vsv.view(length,a*a),1)
492     #
493     vs = vsv.view(length,a*a)
494     return vs
495
496
497
498
499

```

```
1
```

```
1 ### classes Relations1 to Relations4 are viewed as chapters
```

```

1 class Relations1 :
2     def __init__(self,pp):
3         #
4         self.pp = pp
5         #
6         self.alpha = self.pp.alpha
7         self.alpha2 = self.alpha * self.alpha
8         self.alpha3 = self.alpha * self.alpha * self.alpha
9         self.alpha3z = self.alpha3 + 1
10        self.beta = self.pp.beta
11        self.betaz = self.beta +1
12        #
13        #self.model = self.mm
14        #
15        self.qvalue = self.pp.qvalue
16        #
17        self.asure_max = self.pp.asure_max
18        #
19        self.infosize = self.pp.infosize
20        self.pastsize = self.pp.pastsize
21        self.futuresize = self.pp.futuresize
22        #
23        #
24        self.ar1 = arangeic(self.alpha).view(self.alpha,1).expand(self.alpha,self.alpha)
25        self.ar2 = arangeic(self.alpha).view(1,self.alpha).expand(self.alpha,self.alpha)
26        self.ida = (self.ar1 == self.ar2)
27        #
28        self.a3r1 = arangeic(self.alpha3).view(self.alpha3,1).expand(self.alpha3,self.alpha3)
29        self.a3r2 = arangeic(self.alpha3).view(1,self.alpha3).expand(self.alpha3,self.alpha3)
30        self.eqa3 = (self.a3r1 == self.a3r2)
31        #
32        self.a3zr1 = arangeic(self.alpha3z).view(self.alpha3z,1).expand(self.alpha3z,self.alpha3z)
33        self.a3zr2 = arangeic(self.alpha3z).view(1,self.alpha3z).expand(self.alpha3z,self.alpha3z)
34        self.eqa3z = (self.a3zr1 == self.a3zr2)
35        #
36        self.iblength = 2 ** (2*self.beta)
37        self.ibarray = torch.zeros((self.iblength,2*self.beta),dtype = torch.bool)

```

```

38     for z in range(self.iblength):
39         self.ibarray[z] = zbinary(2*self.beta , z)
40     #
41     self.betazsubsets = self.makebetazsubsets() # at location j,::: it is f
42     self.quantities = self.betazsubsets[:,0:self.beta].to(torch.int).sum(1)
43     #
44
45
46     ##### general manipulation of data
47
48     def printprod(self,Data,i):
49         length = Data['length']
50         prod = Data['prod']
51         a = self.alpha
52         bz = self.betaz
53         #
54         assert i < length
55         #
56         printarray = torch.zeros((a,a),dtype = torch.int,device=Dvc)
57         printarray += 9 * (10 ** bz)
58         for p in range(bz):
59             printarray += (10 ** p) * (prod[i,:::,p].to(torch.int))
60         print(nump(printarray))
61         return
62
63     def printrandprods(self,Data,number):
64         length = Data['length']
65         upper = number
66         if upper > length:
67             upper = length
68         indices = torch.randperm(length,device=Dvc)
69         for i in range(upper):
70             indexi = indices[i]
71             print("-----")
72             self.printprod(Data,indexi)
73         print("-----")
74         return
75
76
77     def makebetazsubsets(self):
78         b = self.beta
79         bz = self.betaz
80         bpower = 2**b
81         subsets = torch.ones((bpower,bz),dtype = torch.bool,device=Dvc)
82         for z in range(bpower):
83             subsets[z,0:b] = zbinary(b,z)
84         return subsets
85
86
87
88     def nulldata(self):
89         length = torch.tensor(0)
90         Output = {
91             'length': length,
92             'depth': None,

```

```

93         'prod': None,
94         'left': None,
95         'right': None,
96         'ternary': None,
97         'info': None,
98     }
99     return Output
100
101 def copydata(self,Data):
102     if Data['length'] == 0:
103         return self.nulldata()
104     Output = {}
105     Output['length'] = itt(Data['length']).clone().detach()
106     for ky in Data.keys():
107         if ky != 'length':
108             Output[ky] = (Data[ky]).clone().detach()
109     return Output
110
111
112 def duplicatedata(self,Data): # like copydata but it puts the same objects
113     if Data['length'] == 0:
114         return self.nulldata()
115     Output = {}
116     Output['length'] = itt(Data['length']).clone().detach()
117     for ky in Data.keys():
118         if ky != 'length':
119             Output[ky] = Data[ky]
120     return Output
121
122
123 def deletedata(self,Data):
124     #del Data['length'] # better avoid doing that
125     datakeyslist = list(Data.keys())
126     for ky in datakeyslist:
127         if ky != 'length':
128             del Data[ky]
129     del Data
130     return
131
132
133
134 def appenddata(self,Data1,Data2): # appends Data2 to Data1 and outputs the r
135     # there is a case where Data1 == None then we just output Data2
136     assert set(Data1.keys()) == set(Data2.keys())
137     if Data1['length'] == 0:
138         return self.copydata(Data2)
139     if Data2['length'] == 0:
140         return self.copydata(Data1)
141     Output = {}
142     Output['length'] = Data1['length'] + Data2['length']
143     #
144     for ky in Data1.keys():
145         if ky != 'length':
146             Output[ky] = torch.cat((Data1[ky],Data2[ky]),0)
147     return Output
148

```

```
148
149
150 def indexselectdata(self,Data,indices):
151     #
152     if len(indices) == 0:
153         return self.nulldata()
154     #
155     Output = {}
156     #
157     Output['length'] = len(indices)
158     #
159     for ky in Data.keys():
160         if ky != 'length':
161             Output[ky] = (Data[ky])[indices].clone().detach()
162     #
163     return Output
164
165
166 def detectsubdata(self,Data,detection):
167     #
168     assert len(detection) == Data['length']
169     #
170     sublength = detection.to(torch.int).sum(0)
171     if sublength == 0:
172         return self.nulldata()
173     #
174     Output = {}
175     #
176     Output['length'] = sublength
177     #
178     for ky in Data.keys():
179         if ky != 'length':
180             Output[ky] = (Data[ky])[detection].detach()
181     #
182     return Output
183
184 def insertdata(self,Data,detection,SubData):
185     #
186     assert set(Data.keys()) == set(SubData.keys())
187     #
188     sublength = SubData['length']
189     assert detection.to(torch.int).sum(0) == sublength
190     #
191     if sublength == 0:
192         return Data
193     #
194     Output = {}
195     Output['length'] = itt(Data['length'])
196     #
197     for ky in Data.keys():
198         if ky != 'length':
199             outputitem = Data[ky].clone().detach()
200             outputitem[detection] = SubData[ky]
201             Output[ky] = outputitem
202     #
203     return Output
```

```

204
205
206
207
208 #####
209
210
211
212 def filterpossible(self,Data): # here we just filter out the impossible cas
213     #
214     length = Data['length']
215     prod = Data['prod']
216     #
217     prodstats = prod.to(torch.int).sum(3)
218     impossible = ((prodstats == 0).any(2)).any(1)
219     #
220     detection = ~impossible
221     return detection
222
223
224
225 def knowledge(self,Data): # now it increases as we refine
226     a = self.alpha
227     a2 = self.alpha2
228     a3 = self.alpha3
229     a3z = self.alpha3z
230     bz = self.betaz
231     #
232     #
233     length = Data['length']
234     prod = Data['prod'] # mask of shape a.a.bz with boolean values
235     left = Data['left']
236     right = Data['right']
237     ternary = Data['ternary']
238     #
239     if length == 0:
240         zerokn = torch.zeros((1),dtype = torch.int,device=Dvc)
241         return zerokn
242     #
243     output = torch.zeros((length),dtype = torch.int64,device=Dvc)
244     output -= prod.to(torch.int64).view(length,a*a*bz).sum(1)
245     output -= left.to(torch.int64).view(length,a*bz*2).sum(1)
246     output -= right.to(torch.int64).view(length,bz*a*2).sum(1)
247     output -= ternary.to(torch.int64).view(length,a*a*a*2).sum(1)
248     return output
249
250
251
252
253
254 def availablexy(self,length,prod):
255     #
256     a = self.alpha
257     a2 = self.alpha2
258     a3 = self.alpha3

```

```

259     a3z = self.alpha3z
260     b = self.beta
261     bz = self.betaz
262     #
263     prodsum = prod.to(torch.int64).sum(3)
264     possible = ((prodsum > 0).all(2)).all(1)
265     possiblexy = possible.view(length,1).expand(length,a2)
266     #
267     optionalxy = (prodsum > 1).view(length,a2)
268     #
269     available_xy = possiblexy & optionalxy
270     return available_xy
271
272 def availablexyp(self,length,prod):
273     #
274     a = self.alpha
275     a2 = self.alpha2
276     a3 = self.alpha3
277     a3z = self.alpha3z
278     b = self.beta
279     bz = self.betaz
280     #
281     prodsum = prod.to(torch.int64).sum(3)
282     possible = ((prodsum > 0).all(2)).all(1)
283     possiblexyp = possible.view(length,1,1,1).expand(length,a,a,bz)
284     #
285     optionalxyp = (prodsum > 1).view(length,a,a,1).expand(length,a,a,bz)
286     #
287     available_xyp = prod & possiblexyp & optionalxyp
288     return available_xyp
289
290 ###
291
292 def upsplitting(self,Data,ivector,xvector,yvector,pvector): # setting x.y =
293     #
294     a = self.alpha
295     a2 = self.alpha2
296     a3 = self.alpha3
297     a3z = self.alpha3z
298     b = self.beta
299     bz = self.betaz
300     #
301     if len(ivector) == 0:
302         return self.rr1.nulldata()
303     #
304     UpData = self.indexselectdata(Data,ivector)
305     length = UpData['length']
306     prod = UpData['prod']
307     #
308     xrangevx = arangeic(a).view(1,a,1,1).expand(length,a,a,bz)
309     yrangevx = arangeic(a).view(1,1,a,1).expand(length,a,a,bz)
310     prangevx = arangeic(bz).view(1,1,1,bz).expand(length,a,a,bz)
311     #
312     xvectorvx = xvector.view(length,1,1,1).expand(length,a,a,bz)
313     yvectorvx = yvector.view(length,1,1,1).expand(length,a,a,bz)

```

```

314     pvectorvx = pvector.view(length,1,1,1).expand(length,a,a,bz)
315     #
316     newprod = prod & ( (xrangevx != xvectorvx) | (yrangevx != yvectorvx) | (
317     #
318     UpData['prod'] = newprod
319     UpData['depth'] += 1
320     #
321     return UpData
322
323
324
325

```

```

1 class Relations2 :
2     def __init__(self,pp):
3         #
4         self.pp = pp
5         #
6         self.rr1 = Relations1(pp)
7         #
8         self.alpha = self.pp.alpha
9         self.alpha2 = self.alpha * self.alpha
10        self.alpha2z = self.alpha2 + 1
11        self.alpha3 = self.alpha * self.alpha * self.alpha
12        self.alpha3z = self.alpha3 + 1
13        self.beta = self.pp.beta
14        self.betaz = self.beta +1
15        #
16        #
17        self.halfones_count = 0
18        self.impossible_basic_count = 0
19        #
20
21
22
23
24
25    def filterpossible(self,Data): # here we just filter out the impossible cas
26        #
27        length = Data['length']
28        prod = Data['prod']
29        #
30        prodstats = prod.to(torch.int).sum(3)
31        impossible = ((prodstats == 0).any(2)).any(1)
32        #
33        detection = ~impossible
34        return detection
35
36
37
38        #####
39        ##### new steps with prod, left, right, ternary
40
41    def modifyternaryStep(self,Data):
42        #

```

```

42     #
43     a = self.alpha
44     a2 = self.alpha2
45     a3 = self.alpha3
46     a3z = self.alpha3z
47     b = self.beta
48     bz = self.betaz
49     #
50     length = Data['length']
51     prod = Data['prod']
52     left = Data['left']
53     right = Data['right']
54     ternary = Data['ternary']
55     #
56     #
57     ivx = arangeic(length).view(length,1,1,1,1).expand(length,a,a,a,bz)
58     xvx = arangeic(a).view(1,a,1,1,1).expand(length,a,a,a,bz)
59     yvx = arangeic(a).view(1,1,a,1,1).expand(length,a,a,a,bz)
60     zvx = arangeic(a).view(1,1,1,a,1).expand(length,a,a,a,bz)
61     pvx = arangeic(bz).view(1,1,1,1,bz).expand(length,a,a,a,bz)
62     #
63     nter0_left = (prod[ivx,yvx,zvx,pvx] & left[ivx,xvx,pvx,0]).any(4)
64     nter1_left = (prod[ivx,yvx,zvx,pvx] & left[ivx,xvx,pvx,1]).any(4)
65     #
66     nter0_right = (prod[ivx,xvx,yvx,pvx] & right[ivx,pvx,zvx,0]).any(4)
67     nter1_right = (prod[ivx,xvx,yvx,pvx] & right[ivx,pvx,zvx,1]).any(4)
68     #
69     nter0v = (nter0_left & nter0_right)
70     nter1v = (nter1_left & nter1_right)
71     #
72     newternary = ternary.clone()
73     newternary[:, :, :, :, 0] = ternary[:, :, :, :, 0] & nter0v
74     newternary[:, :, :, :, 1] = ternary[:, :, :, :, 1] & nter1v
75     #
76     NewData = self.rr1.copydata(Data)
77     NewData['ternary'] = newternary.detach()
78     #
79     return NewData
80
81     def modifylefttrightStep(self,Data):
82         #
83         a = self.alpha
84         a2 = self.alpha2
85         a3 = self.alpha3
86         a3z = self.alpha3z
87         b = self.beta
88         bz = self.betaz
89         #
90         length = Data['length']
91         prod = Data['prod']
92         left = Data['left']
93         right = Data['right']
94         ternary = Data['ternary']
95         #
96         prodstats = prod.to(torch.int64).sum(3)
97         unique = (prodstats == 1)

```

```

97         unique = (prod[ivx, yvx, zvx, pvx],
98         #
99         ivx = arangeic(length).view(length, 1, 1, 1, 1).expand(length, a, a, a, bz)
100        xvx = arangeic(a).view(1, a, 1, 1, 1).expand(length, a, a, a, bz)
101        yvx = arangeic(a).view(1, 1, a, 1, 1).expand(length, a, a, a, bz)
102        zvx = arangeic(a).view(1, 1, 1, a, 1).expand(length, a, a, a, bz)
103        pvx = arangeic(bz).view(1, 1, 1, 1, bz).expand(length, a, a, a, bz)
104        #
105        nleft0 = (( (~prod[ivx, yvx, zvx, pvx]) | (~unique[ivx, yvx, zvx]) | ternary
106        nleft1 = (( (~prod[ivx, yvx, zvx, pvx]) | (~unique[ivx, yvx, zvx]) | ternary
107        #
108        nright0 = (( (~prod[ivx, xvx, yvx, pvx]) | (~unique[ivx, xvx, yvx]) | ternar
109        nright1 = (( (~prod[ivx, xvx, yvx, pvx]) | (~unique[ivx, xvx, yvx]) | ternar
110        #
111        newleft = left.clone()
112        newright = right.clone()
113        #
114        newleft[:, :, :, 0] = left[:, :, :, 0] & nleft0
115        newleft[:, :, :, 1] = left[:, :, :, 1] & nleft1
116        newright[:, :, :, 0] = right[:, :, :, 0] & (nright0.permute(0, 2, 1))
117        newright[:, :, :, 1] = right[:, :, :, 1] & (nright1.permute(0, 2, 1))
118        #
119        NewData = self.rr1.copydata(Data)
120        NewData['left'] = newleft.detach()
121        NewData['right'] = newright.detach()
122        #
123        return NewData
124
125
126
127
128    def modifyprodStep(self, Data):
129        #
130        a = self.alpha
131        a2 = self.alpha2
132        a3 = self.alpha3
133        a3z = self.alpha3z
134        b = self.beta
135        bz = self.betaz
136        #
137        length = Data['length']
138        prod = Data['prod']
139        left = Data['left']
140        right = Data['right']
141        ternary = Data['ternary']
142        #
143        lvx = arangeic(length).view(length, 1, 1, 1, 1).expand(length, a, a, a, bz)
144        xvx = arangeic(a).view(1, a, 1, 1, 1).expand(length, a, a, a, bz)
145        yvx = arangeic(a).view(1, 1, a, 1, 1).expand(length, a, a, a, bz)
146        zvx = arangeic(a).view(1, 1, 1, a, 1).expand(length, a, a, a, bz)
147        pvx = arangeic(bz).view(1, 1, 1, 1, bz).expand(length, a, a, a, bz)
148        #
149        leftbin01 = (left[lvx, xvx, pvx, 0] | ternary[lvx, xvx, yvx, zvx, 1])
150        leftbin10 = (left[lvx, xvx, pvx, 1] | ternary[lvx, xvx, yvx, zvx, 0])
151        #
152        rightbin01 = (right[lvx, pvx, zvx, 0] | ternary[lvx, xvx, yvx, zvx, 1])

```

```

153     rightbin10 = (right[lvx,pvx,zvx,1] | ternary[lvx,xvx,yvx,zvx,0])
154     #
155     newprod = prod.clone()
156     newprod = newprod & ( (leftbin01 & leftbin10).all(1) )
157     newprod = newprod & ( (rightbin01 & rightbin10).all(3) )
158     #
159     NewData = self.rr1.copydata(Data)
160     NewData['prod'] = newprod.detach()
161     #
162     return NewData
163
164
165     def process(self,Data):
166         length = Data['length']
167         if length == 0:
168             return Data
169         #
170         #
171         OutputData = self.rr1.copydata(Data)
172         nprod = Data['prod']
173         nprodstats = nprod.to(torch.int64).sum(3)
174         subset = ((nprodstats > 0).all(2)).all(1)
175         NextData = self.rr1.detectsubdata(Data,subset)
176         if subset.to(torch.int).sum(0) == 0:
177             return OutputData
178         for i in range(1000):
179             priorknowledge = self.rr1.knowledge(NextData)
180             #
181             #
182             NextData = self.modifyternaryStep(NextData)
183             #
184             NextData = self.modifyleftrightStep(NextData)
185             #
186             NextData = self.modifyprodStep(NextData)
187             #
188             nextknowledge = self.rr1.knowledge(NextData)
189             nextdonedetected = (priorknowledge >= nextknowledge)
190             subset_nextdone = composedetections(length,subset,nextdonedetected)
191             NextDoneData = self.rr1.detectsubdata(NextData,nextdonedetected)
192             OutputData = self.rr1.insertdata(OutputData,subset_nextdone,NextDoneData)
193             #
194             subset = subset & (~subset_nextdone)
195             if subset.to(torch.int).sum(0) == 0:
196                 break
197             NextData = self.rr1.detectsubdata(NextData, ~nextdonedetected )
198         return OutputData
199
200
201     def impossibleFilter(self,Data):
202         a = self.alpha
203         a2 = self.alpha2
204         a3 = self.alpha3
205         a3z = self.alpha3z
206         b = self.beta
207         bz = self.betaz

```

```

208     #
209     length = Data['length']
210     prod = Data['prod']
211     left = Data['left']
212     right = Data['right']
213     ternary = Data['ternary']
214     #
215     prodstats = prod.to(torch.int64).sum(3)
216     possible = ((prodstats > 0).all(2)).all(1)
217     #
218     leftv = left.view(length,a*bz,2)
219     rightv = right.view(length,bz*a,2)
220     ternaryv = ternary.view(length,a3,2)
221     left_possible = (leftv.any(2)).all(1)
222     right_possible = (rightv.any(2)).all(1)
223     ternary_possible = (ternaryv.any(2)).all(1)
224     #
225     detection = (~possible) | (~left_possible) | (~right_possible) | (~terna
226     return detection
227
228     def profileFilter(self,Data):
229         a = self.alpha
230         a2 = self.alpha2
231         a3 = self.alpha3
232         a3z = self.alpha3z
233         b = self.beta
234         bz = self.betaz
235         #
236         length = Data['length']
237         prod = Data['prod']
238         left = Data['left']
239         right = Data['right']
240         ternary = Data['ternary']
241         #
242         left_def = ( (left.to(torch.int64).sum(3)) == 1 )
243         right_def = ( (right.to(torch.int64).sum(3)) == 1 )
244         profile_def = ( left_def.all(1) ) & ( right_def.all(2) )
245         left_pro = ( left[:, :, :, 0] ).permute(0,2,1)
246         right_pro = right[:, :, :, 0]
247         profile = torch.cat((left_pro,right_pro),2)
248         profile_vx1 = profile.view(length,bz,1,2*a).expand(length,bz,bz,2*a)
249         profile_vx2 = profile.view(length,1,bz,2*a).expand(length,bz,bz,2*a)
250         same_profile = (profile_vx1 == profile_vx2).all(3)
251         #
252         profile_def1 = profile_def.view(length,bz,1).expand(length,bz,bz)
253         profile_def2 = profile_def.view(length,1,bz).expand(length,bz,bz)
254         #
255         same_profile_def = (profile_def1 & profile_def2 & same_profile)
256         prange1 = arangeic(bz).view(1,bz,1).expand(length,bz,bz)
257         prange2 = arangeic(bz).view(1,1,bz).expand(length,bz,bz)
258         #
259         detection = (( (prange1 != prange2) & same_profile_def ).any(2)).any(1)
260         #
261         return detection
262

```

```

263     def doneFilter(self,Data):
264         a = self.alpha
265         a2 = self.alpha2
266         a3 = self.alpha3
267         a3z = self.alpha3z
268         b = self.beta
269         bz = self.betaz
270         #
271         length = Data['length']
272         prod = Data['prod']
273         ternary = Data['ternary']
274         #
275         prodstats = prod.to(torch.int64).sum(3)
276         #
277         binsum = ternary.view(length,a3,2).to(torch.int64).sum(2)
278         ternary_all = (binsum == 1).all(1)
279         #
280         #detection = ( ((prodstats == 1).all(2)).all(1) ) | ternary_all
281         detection = ( ((prodstats == 1).all(2)).all(1) )
282         #
283         return detection
284
285     def halfonesFilter(self,Data): # only look at cases where the number of
286         # ones on the left is >= the number on the right
287         a = self.alpha
288         a2 = self.alpha2
289         a3 = self.alpha3
290         a3z = self.alpha3z
291         b = self.beta
292         bz = self.betaz
293         #
294         length = Data['length']
295         prod = Data['prod']
296         left = Data['left']
297         right = Data['right']
298         #
299         prodstats = prod.to(torch.int64).sum(3)
300         leftstats = left.to(torch.int64).sum(3)
301         rightstats = right.to(torch.int64).sum(3)
302         #
303         assert (((leftstats <= 1).all(2)).all(1)).all(0)
304         #
305         leftones = (left[:, :, :, 1].to(torch.int64).sum(2)).sum(1)
306         right_isone = (rightstats == 1) & right[:, :, :, 1]
307         rightones = (right_isone.to(torch.int64).sum(2)).sum(1)
308         #
309         #
310         detection = (rightones > leftones)
311         #
312         return detection
313
314     def filterdata(self,Data): #
315         #
316         #
317         impossibledetect = self.impossibleFilter(Data)

```

```

318 profiledetect = self.profileFilter(Data)
319 #
320 if self.pp.profile_filter_on:
321     impossibledetect = impossibledetect | profiledetect
322 #
323 self.impossible_basic_count += impossibledetect.to(torch.int64).sum(0)
324 # experimental:
325 if self.pp.halfones_filter_on:
326     halfonesdetect = self.halfonesFilter(Data)
327     self.halfones_count += (halfonesdetect & (~impossibledetect)).to(torch.int64).sum(0)
328 #
329     impossibledetect = impossibledetect | halfonesdetect
330 #
331 donedetect = self.doneFilter(Data)
332 donedetect = donedetect & (~impossibledetect)
333 #
334 activedetect = (~impossibledetect) & ~donedetect
335 #
336 return activedetect, donedetect, impossibledetect
337
338
339
340
341
342
343
344

```

```

1 class Relations3 :
2     def __init__(self,pp):
3         #
4         self.pp = pp
5         #
6         self.rr2 = Relations2(pp)
7         self.rr1 = self.rr2.rr1
8         #
9         self.alpha = self.pp.alpha
10        self.alpha2 = self.alpha * self.alpha
11        self.alpha2z = self.alpha2 + 1
12        self.alpha3 = self.alpha * self.alpha * self.alpha
13        self.alpha3z = self.alpha3 + 1
14        self.beta = self.pp.beta
15        self.betaz = self.beta + 1
16        #
17
18
19    def printmultiplicities(self,Data):
20        #
21        dlength = self.alpha2 + 1
22        #
23        length = Data['length']
24        depth = Data['depth']
25        if length == 0:
26            multiplicities = torch.zeros((dlength),dtype = torch.int,device=Dvc)
27            print(numpy(multiplicities))

```

```

28         return
29     #
30     dmax,dindices = torch.max(depth,0)
31     if dmax +2 > dlength:
32         dlength = dmax +2
33     if dlength > 50:
34         dlength = 50
35     #
36     depthvx = depth.view(length,1).expand(length,dlength)
37     drangevx = arangeic(dlength).view(1,dlength).expand(length,dlength)
38     rectangle = (depthvx == drangevx)
39     multiplicities = rectangle.sum(0)
40     #
41     #print("dlength",itp(dlength))
42     print("multiplicities in active pool by depth:")
43     print(nump(multiplicities))
44     return
45
46 def selectchunk(self,Data):
47     #
48     length = Data['length']
49     depth = Data['depth']
50     prod = Data['prod']
51     #
52     #
53     assert length > 0
54     #
55     prodstats = prod.to(torch.int).sum(3)
56     assert ((prodstats >0).all(2)).all(1)).all(0)
57     optional = (prodstats > 1)
58     assert ((optional.any(2)).any(1)).all(0)
59     #
60     values,indices = torch.sort(depth,0,descending = True)
61     upper = length
62     if upper > self.pp.chunksize:
63         upper = self.pp.chunksize
64     indices_upper = indices[0:upper]
65     #
66     cdetection = torch.zeros((length),dtype = torch.bool,device=Dvc)
67     cdetection[indices_upper] = True
68     #
69     ChunkData = self.rr1.detectsubdata(Data,cdetection)
70     #
71     if self.pp.verbose:
72         self.printmultiplicities(Data)
73     #
74     return ChunkData, cdetection
75
76 def network_vcuts(self,M,Data,randomize):
77     a = self.alpha
78     a2 = self.alpha2
79     a3 = self.alpha3
80     a3z = self.alpha3z
81     b = self.beta
82     bz = self.betaz

```

```

83     #
84     length = Data['length']
85     depth = Data['depth']
86     prod = Data['prod']
87     #
88     assert length > 0
89     #
90     #
91     prodstats = prod.to(torch.int64).sum(3)
92     #
93     assert (((prodstats > 0).all(2)).all(1)).all(0)
94     #
95     #
96     availablexyr = self.rr1.availablexy(length,prod).reshape(length*a2)
97     #
98     networkscorer = M.network2(Data).detach().reshape(length*a2)
99     #
100    if randomize:
101        #
102        epsilon_tirage = torch.rand(length*a2,device=Dvc)
103        alll = torch.clamp(M.average_local_loss,0.,0.5)
104        epsilon_factor = M.average_local_loss * self.pp.perturbation_factor
105        epsilon = torch.rand(length*a2,device=Dvc)
106        networkscorer += (epsilon_factor * epsilon)
107        #
108        phase = Data['info'][:,self.pp.phase]
109        tirage = torch.rand(length,device=Dvc)
110        detection = (phase == 1) | ( (tirage < 0.1) & (phase == 2) )
111        detectionvxr = detection.view(length,1).expand(length,a2).reshape(le
112        randomness = torch.rand(length*a2,device=Dvc)
113        networkscorer[detectionvxr] = randomness[detectionvxr]
114        #
115        #
116        networkscorer = torch.clamp(networkscorer, -1., 10.)
117        networkscorer[~availablexyr] = 20.
118        networkscore = networkscorer.view(length,a2)
119        #
120        values,xyvector = torch.min(networkscore,1)
121        #
122        return xyvector
123
124
125
126    def addvalencies(self,availablexyp,xyvector): # adds into the HST file the
127        # also adds the passive count (just the length of the xyvector)
128        #
129        a = self.alpha
130        a2 = self.alpha2
131        a2z = self.alpha2 +1
132        a3 = self.alpha3
133        a3z = self.alpha3z
134        b = self.beta
135        bz = self.betaz
136        #
137        length = len(xyvector)

```

```

138     HST.current_proof_passive_count += length
139     #
140     availablexypv = availablexyp.view(length,a2,bz)
141     lrange = arangeic(length)
142     available_cuts = availablexypv[lrange,xyvector]
143     valency = available_cuts.to(torch.int64).sum(1)
144     for v in range(bz + 1):
145         HST.current_proof_valency_frequency[v] += (valency == v).to(torch.in
146     return
147
148     def managesplit(self,M,DataToSplit,randomize):
149         #
150         a = self.alpha
151         a2 = self.alpha2
152         a2z = self.alpha2 +1
153         a3 = self.alpha3
154         a3z = self.alpha3z
155         b = self.beta
156         bz = self.betaz
157         #
158         #
159         length = DataToSplit['length']
160         prod = DataToSplit['prod']
161         #
162         availablexyp = self.rr1.availablexyp(length,prod).view(length,a2,bz)
163         #
164         xyvector = self.network_vcuts(M,DataToSplit,randomize)
165         #
166         self.addvalencies(availablexyp,xyvector)
167         #
168         lrangevxr = arangeic(length).view(length,1).expand(length,bz).reshape(le
169         xyvectorvxr = xyvector.view(length,1).expand(length,bz).reshape(length*b
170         bzrangevxr = arangeic(bz).view(1,bz).expand(length,bz).reshape(length*bz
171         #
172         verticaldetect = availablexyp[lrangevxr,xyvectorvxr,bzrangevxr]
173         #
174         #
175         ivector_vert = lrangevxr[verticaldetect]
176         xyvector_vert = xyvectorvxr[verticaldetect]
177         pvector_vert = bzrangevxr[verticaldetect]
178         #
179         prx = arangeic(a).view(a,1).expand(a,a).reshape(a2)
180         pry = arangeic(a).view(1,a).expand(a,a).reshape(a2)
181         #
182         xvector_vert = prx[xyvector_vert]
183         yvector_vert = pry[xyvector_vert]
184         #
185         NewData = self.rr1.upsplitting(DataToSplit,ivector_vert,xvector_vert,yve
186         #
187         #
188         ndlength = NewData['length']
189         #
190         #
191         AssocNewData = self.rr1.nullldata()
192         detection = torch.zeros((ndlength),dtype = torch.bool,device=Dvc)

```

```

193 newactive = torch.zeros((ndlength),dtype = torch.bool,device=Dvc)
194 newdone = torch.zeros((ndlength),dtype = torch.bool,device=Dvc)
195 newimpossible = torch.zeros((ndlength),dtype = torch.bool,device=Dvc)
196 lower = 0
197 for i in range(ndlength):
198     assert lower < ndlength
199     upper = lower + 1000
200     if upper > ndlength:
201         upper = ndlength
202     detection[:] = False
203     detection[lower:upper] = True
204     NewDataSlice = self.rr1.detectsubdata(NewData,detection)
205     AssocNewDataSlice = self.rr2.process(NewDataSlice)
206     AssocNewData = self.rr1.appenddata(AssocNewData,AssocNewDataSlice)
207     newactive_s,newdone_s,newimpossible_s = self.rr2.filterdata(AssocNew
208     newactive[lower:upper] = newactive_s
209     newdone[lower:upper] = newdone_s
210     newimpossible[lower:upper] = newimpossible_s
211     lower = upper
212     if lower >= ndlength:
213         break
214     #
215     NewActiveData = self.rr1.detectsubdata(AssocNewData,newactive)
216     #
217     NewDoneData = self.rr1.detectsubdata(AssocNewData,newdone)
218     #
219     if NewActiveData['length'] > 0:
220         phase1 = ( NewActiveData['info'][:,self.pp.phase] == 1)
221         phase2 = ( NewActiveData['info'][:,self.pp.phase] == 2)
222         tirage = torch.rand(NewActiveData['length'], device=Dvc)
223         phasechange = phase2 & (tirage < self.pp.splitting_probability)
224         newphase = NewActiveData['info'][:,self.pp.phase].clone()
225         newphase[phase1] = 0
226         newphase[phasechange] = 1
227         NewActiveData['info'][:,self.pp.phase] = newphase
228     #
229     HST.current_proof_impossible_count += newimpossible.to(torch.int64).sum(
230     HST.current_proof_done_count += newdone.to(torch.int64).sum(0)
231     #
232     if self.pp.verbose:
233         print(" >>>")
234         print("DataToSplit",itp(DataToSplit['length']))
235         print("NewData",itp(NewData['length']))
236         print("NewActiveData",itp(NewActiveData['length']))
237         print("NewDoneData",itp(NewDoneData['length']))
238         print("-----")
239     #
240     return NewActiveData, NewDoneData
241
242
243

```

```

1 class Relations4 :
2     def __init__(self,pp):
3         #

```

```
4     self.pp = pp
5     #
6     self.rr3 = Relations3(pp)
7     self.rr2 = self.rr3.rr2
8     self.rr1 = self.rr3.rr1
9     #
10    self.alpha = self.pp.alpha
11    self.alpha2 = self.alpha * self.alpha
12    self.alpha3 = self.alpha * self.alpha * self.alpha
13    self.alpha3z = self.alpha3 + 1
14    self.beta = self.pp.beta
15    self.betaz = self.beta +1
16    #
17    self.prooflooplength = self.pp.prooflooplength
18    self.done_max = 1000 # should be self.pp.done_max
19    #
20    self.sleeptime = self.pp.sleeptime
21    self.periodicity = self.pp.periodicity
22    self.stopthreshold = self.pp.stopthreshold
23    #
24    self.SamplePool = self.rr1.nullldata()
25    self.DroppedSamplePool = self.rr1.nullldata()
26    # these are by convention active (not done or impossible)
27    #
28    self.donecount = itt(0)
29    self.ECN = 0.
30    #
31    self.proofnumber = 0
32    self.allnumbers = 0
33    self.proofinstance = 0
34    self.dropoutratio = 1.
35
36    def resetsamples(self):
37        self.SamplePool = self.rr1.nullldata()
38        self.DroppedSamplePool = self.rr1.nullldata()
39        #
40        self.rr2.impossible_basic_count = 0
41        self.rr2.halfones_count = 0
42        self.dropoutratio = 1.
43        return
44
45    def printexamples(self,Data):
46        #
47        a = self.alpha
48        a2 = self.alpha2
49        a3 = self.alpha3
50        a3z = self.alpha3z
51        b = self.beta
52        bz = self.betaz
53        #
54        length = Data['length']
55        depth = Data['depth']
56        prod = Data['prod']
57        ternary = Data['ternary']
58        #
```

```

59     if length == 0:
60         print("length 0, no examples to print")
61         return
62     #
63     bini = ternary.to(torch.int64)
64     ternary_print = bini[:, :, 0] + 2*bini[:, :, 1] - 1
65     #
66     permutation = torch.randperm((length), device=Dvc)
67     upper = 5
68     if upper > length:
69         upper = length
70     for i in range(upper):
71         indexi = permutation[i]
72         print("-----")
73         self.rr1.printprod(Data, indexi)
74         print(nump(quad[indexi]))
75         print(nump(ternary_print[indexi]))
76     print("-----")
77
78
79
80     def transitionactive(self, ActivePool, cdetection, NewActiveData):
81         #
82         ResidualActive = self.rr1.detectsubdata(ActivePool, ~cdetection)
83         NextActivePool = self.rr1.appenddata(NewActiveData, ResidualActive)
84         #
85         NextActivePoolCopy = self.rr1.copydata(NextActivePool)
86         self.rr1.deletedata(NextActivePool)
87         #
88         return NextActivePoolCopy
89
90     def transitiondone(self, C, DonePool, DoneData, apleNGTH):
91         #
92         idl = DoneData['length']
93         #
94         self.donecount += idl
95         #
96         #
97         if self.pp.verbose:
98             print("new done count is", itp(self.donecount))
99         #
100        #
101        #NewDonePool = self.rr1.nullldata()
102        NewDonePool = self.rr1.appenddata(DonePool, DoneData)
103        ndlength = NewDonePool['length']
104        if ndlength > self.done_max:
105            #print("new done pool of length", itp(ndlength), "so we send to classi
106            print("/", end='')
107            DataToProcess = self.rr1.copydata(NewDonePool)
108            NewDonePool = self.rr1.nullldata()
109            C.process(DataToProcess)
110            #
111        return NewDonePool
112
113

```

```

114 def transitionsamples(self,ActivePool,DroppedPool):
115     #
116     # transitioning samples
117     #
118     slength = self.SamplePool['length']
119     aplength = ActivePool['length']
120     if aplength == 0:
121         assert DroppedPool['length'] == 0
122         return
123     apdepth = ActivePool['depth'].to(torch.int64)
124     #
125     aprectangle = ActivePool['info'][:,self.pp.sampleinfo.lower:self.pp.sample
126     #
127     aprange = arangeic(aplength)
128     #
129     # now add the new sample locations to the rectangle
130     newsloc = arangeic(aplength) + slength
131     #
132     aprectangle[aprange,apdepth] = newsloc
133     #
134     # this should modify active pool outside the present function:
135     ActivePool['info'][:,self.pp.sampleinfo.lower:self.pp.sampleinfo.upper] =
136     # that isn't needed for dropped pool since it doesn't get refered back t
137     #
138     self.SamplePool = self.rr1.appenddata(self.SamplePool, ActivePool)
139     self.DroppedSamplePool = self.rr1.appenddata(self.DroppedSamplePool, Dro
140     #
141     #print("sample pool has size",itp(self.SamplePool['length']))
142     #Fws.trace("transition samples Active Pool",ActivePool,5,0,0,0)
143     #Fws.trace("transition samples Sample Pool",self.SamplePool,5,0,0,0)
144     #self.printsampleex()
145     return
146
147
148 def proofloop(self,Mstrat,Mlearn,C,Input,dropoutlimit):
149     #
150     self.resettsamples()
151     #
152     if dropoutlimit > 0:
153         randomize = True
154     else:
155         randomize = False
156     #
157     InitialActiveData = self.rr2.process(Input)
158     activedetect, donedetect, impossibledetect = self.rr2.filterdata(Initial
159     implength = impossibledetect.to(torch.int).sum(0)
160     donelength = donedetect.to(torch.int).sum(0)
161     if self.pp.verbose:
162         print("initial filter finds",itp(implength),"impossibilities and",it
163     ActivePool = self.rr1.detectsubdata(InitialActiveData,activedetect)
164     #
165     napcount = 0
166     #
167     DonePool = self.rr1.detectsubdata(InitialActiveData,donedetect)
168     self.doncount = itt(0)

```

```

169     if ActivePool['length'] == 0:
170         DonePool = self.transitiondone(DonePool,self.rr1.nulldata(),ActivePo
171     #
172     #
173     self.ECN = itt(ActivePool['length']).to(torch.float).clone()
174     EDN = self.ECN.clone()
175     if self.pp.verbose:
176         print("starting with ECN = EDN from initial active pool",numpr(self.
177     #
178     if dropoutlimit > 0:
179         ActivePool,DroppedPool,newsum,droppedsum = self.dropoutdata(Mlearn,A
180         if self.pp.dropout_style == 'adaptive':
181             activelengthf = itt(ActivePool['length']).clone().to(torch.float
182             self.ECN = (activelengthf + droppedsum)
183             EDN = 0.
184     #
185     stepcount = 0
186     for i in range(self.proofloplength):
187         stepcount += 1
188         prooflength = i
189         if ActivePool['length'] > 0:
190             #
191             PreAPL = itt(ActivePool['length']).clone()
192             #
193             if self.pp.verbose:
194                 print("= = = = = loop",i,"= = = = =",end=' ')
195                 print(itp(self.proofnumber),"/",itp(self.allnumbers),"<",itp
196             else:
197                 print(".",end = ' ')
198                 if (i%50) == 49:
199                     print(" ")
200                 if (i%100) == 0:
201                     print(i)
202             napcount += 1
203             #
204             ChunkData, cdetection = self.rr3.selectchunk(ActivePool)
205             #
206             #
207             CurrentData, DoneData = self.rr3.managesplit(Mstrat,ChunkData,ra
208             #
209             #
210             ActivePool = self.transitionactive(ActivePool,cdetection,Current
211             # do the following before dropout
212             if dropoutlimit == 0:
213                 EDN = itt(ActivePool['length']).clone().to(torch.float)
214                 self.ECN += itt(CurrentData['length']).clone().to(torch.floa
215                 if self.ECN > HST.proof_nodes_max:
216                     print("break after maximum proof nodes")
217                     break
218             #
219             if dropoutlimit > 0:
220                 if self.pp.dropout_style == 'regular' or self.pp.dropout_sty
221                 PostAPL = itt(ActivePool['length']).clone().to(torch.flo
222                 ratio = PostAPL / PreAPL
223                 EDN *= ratio

```



```

277 doneLength = DonePool[ length ]
280 if doneLength > 0:
281     C.process(DonePool)
282     DonePool = self.rr1.nulldata()
283 #
284 if dropoutLimit == 0:
285     cumulative_nodes = torch.round(self.ECN).to(torch.int64)
286     HST.record_full_proof(Mstrat,stepcount,cumulative_nodes,self.donecou
287 else:
288     HST.record_dropout_proof(self.pp.dropout_style,dropoutLimit,stepcoun
289 #
290 if self.pp.verbose:
291     if activeLength > 0:
292         print("there remained",itp(activeLength),"active locations", end
293     else:
294         print("no further active locations", end=' ')
295     print("done pool has length",itp(doneLength))
296     print("Estimated Cumulative Nodes at end of proof",numpr(self.ECN,1)
297     print("done count is",itp(self.donecount))
298     print("impossible basic count is",itp(self.rr2.impossible_basic_coun
299     print("half ones count is",itp(self.rr2.halfones_count))
300 return True, ActivePool, DonePool, proofLength
301
302 def dropoutdata(self,M,Data,dropoutLimit):
303     if self.pp.dropout_style == 'regular':
304         NewData,DroppedData = self.dropoutdataRegular(Data,dropoutLimit)
305         newsum = 0.
306         droppedsum = 0.
307     if self.pp.dropout_style == 'adaptive':
308         NewData,DroppedData,newsum,droppedsum = self.dropoutdataAdaptive(M,D
309     if self.pp.dropout_style == 'uniform':
310         NewData,DroppedData,newsum,droppedsum = self.dropoutdataUniform(M,Da
311 #
312 return NewData,DroppedData, newsum,droppedsum
313
314
315 def dropoutdataRegular(self,Data,dropoutLimit):
316     length = Data['length']
317     if length == 0:
318         return Data, self.rr1.nulldata()
319     permutation = torch.randperm(length,device = Dvc)
320     upper = dropoutLimit
321     if upper > length:
322         NewData = self.rr1.copydata(Data)
323         DroppedData = self.rr1.nulldata()
324     else:
325         indices = permutation[0:upper]
326         indices_dropped = permutation[upper:length]
327         NewData = self.rr1.indexselectdata(Data,indices)
328         DroppedData = self.rr1.indexselectdata(Data,indices_dropped)
329     return NewData,DroppedData
330
331 def extent_sliced(self,M,Data):
332     #
333     length = Data['length']
334     if length <= 1000:

```

```

335         extent_log = M.network(Data).detach()
336         extent_log = torch.clamp(extent_log,0.,8.)
337         extent = 10**extent_log
338         return extent
339     extent = torch.zeros((length),dtype = torch.float,device=Dvc)
340     lrange = arangeic(length)
341     #
342     lower = 0
343     for i in range(length):
344         upper = lower + 1000
345         if upper > length:
346             upper = length
347         indices = lrange[lower:upper]
348         DataSlice = self.rr1.indexselectdata(Data,indices)
349         extent_log = M.network(DataSlice).detach()
350         extent_log = torch.clamp(extent_log,0.,8.)
351         extent[lower:upper] = 10**extent_log
352         lower = upper
353         if upper >= length:
354             break
355     return extent
356
357 def dropoutdataAdaptive(self,M,Data,dropoutlimit):
358     length = Data['length']
359     if length == 0:
360         return Data, self.rr1.nullldata(),0.,0.
361     #
362     extent = self.extent_sliced(M,Data)
363     denom = extent.sum(0)
364     proba = (dropoutlimit * extent)/denom
365     tirage = torch.rand(length,device=Dvc)
366     detection = (tirage < proba)
367     indices1 = arangeic(length)[detection]
368     dlenght = detection.to(torch.int64).sum(0)
369     if dlenght > dropoutlimit:
370         indices1 = arangeic(length)[detection]
371         permutation = torch.randperm(dlenght)
372         indices2 = permutation[dropoutlimit:dlenght]
373         indices3 = indices1[indices2]
374         detection[indices3] = False
375     if length <= dropoutlimit:
376         NewData = self.rr1.copydata(Data)
377         DroppedData = self.rr1.nullldata()
378         newsum = extent.sum(0)
379         droppedsum = 0.
380     else:
381         NewData = self.rr1.detectsubdata(Data,detection)
382         DroppedData = self.rr1.detectsubdata(Data,(~detection))
383         newsum = (extent[detection]).sum(0)
384         droppedsum = (extent[~detection]).sum(0)
385     return NewData,DroppedData, newsum, droppedsum
386
387
388 def dropoutdataUniform(self,M,Data,dropoutlimit):
389     length = Data['length']

```

```

390     if length == 0:
391         return Data, self.rr1.nulldata(),0.,0.
392     #
393     extent = self.extent_sliced(M,Data)
394     #
395     values,sort_indices = torch.sort(extent,0)
396     fraction = itf(length) / itf(dropoutlimit)
397     epsilon_multiplier = itf(length - dropoutlimit) / itf(length)
398     epsilon_multiplier = torch.clamp(epsilon_multiplier,0.,1.)
399     drange = arangeic(dropoutlimit).to(torch.float)
400     tirage = torch.rand(dropoutlimit,device=Dvc)
401     tirage2 = torch.rand(dropoutlimit,device=Dvc) - 0.5
402     tirage2vx = tirage2.view(dropoutlimit,1).expand(dropoutlimit,dropoutlimi
403     irange = arangeic(dropoutlimit).view(dropoutlimit,1).expand(dropoutlimit
404     jrange = arangeic(dropoutlimit).view(1,dropoutlimit).expand(dropoutlimit
405     tirage2_triangle = tirage2vx * ( (irange > jrange).to(torch.float) )
406     tirage2_integral = tirage2_triangle.sum(0)
407     epsilon = tirage * epsilon_multiplier
408     drange_mod = drange + epsilon + (0.05 * tirage2_integral)
409     #
410     float_indices = drange_mod * fraction
411     round_indices = torch.round(float_indices).to(torch.int64)
412     round_indices = torch.clamp(round_indices,0,length-1)
413     combined_indices = sort_indices[round_indices]
414     detection = torch.zeros((length),dtype = torch.bool,device=Dvc)
415     detection[combined_indices] = True
416     #
417     if length <= dropoutlimit:
418         NewData = self.rr1.copydata(Data)
419         DroppedData = self.rr1.nulldata()
420         newsum = extent.sum(0)
421         droppedsum = 0.
422     else:
423         NewData = self.rr1.detectsubdata(Data,detection)
424         DroppedData = self.rr1.detectsubdata(Data,(~detection))
425         newsum = (extent[detection]).sum(0)
426         droppedsum = (extent[~detection]).sum(0)
427     return NewData,DroppedData, newsum, droppedsum
428
429
430
431 def printsampleex(self):
432     samplelength = self.SamplePool['length']
433     if samplelength == 0:
434         return
435     upper = 20
436     if upper > samplelength:
437         upper = samplelength
438     permutation = torch.randperm(samplelength,device=Dvc)
439     depth = self.SamplePool['depth']
440     points = self.SamplePool['info'][ :,self.pp.samplepoints]
441     for i in range(upper):
442         ip = permutation[i]
443         print("number",ip,"depth",itp(depth[ip]),"points",itp(points[ip]))
444     return

```

445  
446  
447  
448  
449  
450

```

1 class Classifier :    # this is a very first part of classification up to isomor
2     def __init__(self,P):
3         #
4         #
5         self.Pp = P
6         self.rr4 = Relations4(self.Pp)
7         self.rr3 = self.rr4.rr2
8         self.rr2 = self.rr4.rr2
9         self.rr1 = self.rr4.rr1
10        self.alpha = self.Pp.alpha
11        self.alpha2 = self.Pp.alpha2
12        self.alpha3 = self.Pp.alpha3
13        self.alpha3z = self.Pp.alpha3z
14        self.beta = self.Pp.beta
15        self.betaz = self.Pp.betaz
16        #
17        self.sga = SymmetricGroup(self.alpha)
18        #
19        self.eqlength = 0
20        self.eqlist = None
21        #
22        #self.iota = 24*24*4
23        self.matrix = self.choosematrix()
24        self.ilength = 10
25        self.indices1,self.indices2,self.indices3,self.indices4,self.vector=self
26
27
28    def initialize(self):
29        self.eqlength = 0
30        self.eqlist = None
31        return
32
33    def choosestuff(self,ilength):
34        assert ilength <= 48
35        permutation1 = torch.randperm(48,device = Dvc)
36        permutation2 = torch.randperm(48,device = Dvc)
37        permutation3 = torch.randperm(48,device = Dvc)
38        permutation4 = torch.randperm(48,device = Dvc)
39        #
40        indices1 = permutation1[0:ilength]
41        indices2 = permutation2[0:ilength]
42        indices3 = permutation3[0:ilength]
43        indices4 = permutation4[0:ilength]
44        #
45        permutationV = torch.randperm(101,device = Dvc)
46        vector = permutationV[0:ilength] - 50
47        return indices1,indices2,indices3,indices4,vector
48

```

```

48
49     def choosematrix(self):
50         #
51         a = self.alpha
52         #
53         #thematrix = torch.zeros((a,a,a,a),dtype = torch.int64,device=Dvc)
54         for i in range(10):
55             permutation = torch.randperm((a*a*a*a),device=Dvc)
56             psquared = permutation*permutation
57             thematrix = psquared.view(a,a,a,a)
58         return thematrix
59
60     def geteq(self,Data):
61         #
62         a = self.alpha
63         a2 = self.alpha2
64         a3 = self.alpha3
65         a4 = self.alpha2 * self.alpha2
66         a3z = self.alpha3z
67         b = self.beta
68         bz = self.betaz
69         #
70         length = Data['length']
71         prod = Data['prod']
72         #
73         prodsum = prod.to(torch.int64).sum(3)
74         #
75         assert ((prodsum == 1).all(2)).all(1)).all(0)
76         #
77         values,table = torch.max(prod.to(torch.int64),3)
78         #
79         table1vx = table.view(length,a,a,1,1).expand(length,a,a,a,a)
80         table2vx = table.view(length,1,1,a,a).expand(length,a,a,a,a)
81         eq = (table1vx == table2vx)
82         iz = (table == b).view(length,a,a)
83         return eq,iz
84
85
86
87     def orderinvariantSlice(self,Data):
88         #
89         a = self.alpha
90         a2 = self.alpha2
91         a3 = self.alpha3
92         a4 = self.alpha2 * self.alpha2
93         a3z = self.alpha3z
94         b = self.beta
95         bz = self.betaz
96         #
97         length = Data['length']
98         #print("at start of orderinvariantSlice, length is",length)
99         prod = Data['prod']
100        #
101        eq,iz = self.geteq(Data)
102        #
103        eqview = eq.view(1,length,a,a,a,a)

```

```

103 eqview = eq.view(1,length,a,a,a,a)
104 izview = iz.view(1,length,a,a,1,1).expand(1,length,a,a,a,a)
105 eqiz = torch.cat((eqview,izview),0)
106 eqiz_p2 = eqiz.permute(0,1,2,3,5,4)
107 eqiz_p3 = eqiz.permute(0,1,2,4,3,5)
108 eqiz_p4 = eqiz.permute(0,1,2,4,5,3)
109 eqiz_p5 = eqiz.permute(0,1,2,5,3,4)
110 eqiz_p6 = eqiz.permute(0,1,2,5,4,3)
111 #
112 eqiz_c1 = torch.cat((eqiz,eqiz_p2,eqiz_p3,eqiz_p4,eqiz_p5,eqiz_p6),0)
113 eqiz_c2 = eqiz_c1.permute(0,1,3,4,5,2)
114 eqiz_c3 = eqiz_c1.permute(0,1,4,5,2,3)
115 eqiz_c4 = eqiz_c1.permute(0,1,5,2,3,4)
116 #
117 eqiz_cat = torch.cat((eqiz_c1,eqiz_c2,eqiz_c3,eqiz_c4),0) # size 48.len
118 #
119 eqiz_cat1 = eqiz_cat[self.indices1]
120 eqiz_cat2 = eqiz_cat[self.indices2]
121 eqiz_cat3 = eqiz_cat[self.indices3]
122 eqiz_cat4 = eqiz_cat[self.indices4]
123 #
124 eqiz_andor = (eqiz_cat1 | eqiz_cat2) & (eqiz_cat3 | eqiz_cat4)
125 #
126 eqiz_sum = ((eqiz_andor.to(torch.int64).sum(5)).sum(4)).sum(3)
127 #
128 vectorvx = self.vector.view(self.ilength,1,1).expand(self.ilength,length)
129 invariant = (eqiz_sum * vectorvx).sum(0)
130 #
131 return invariant
132
133 def orderinvariant(self,Data):
134 #
135 a = self.alpha
136 #
137 length = Data['length']
138 #
139 lrange = arangeic(length)
140 #
141 invariant = torch.zeros((length,a),dtype = torch.int64,device=Dvc)
142 #
143 lower = 0
144 for i in range(length):
145     upper = lower + 100
146     if upper > length:
147         upper = length
148     indices = lrange[lower:upper]
149     DataSlice = self.rr1.indexselectdata(Data,indices)
150     invariant[lower:upper] = self.orderinvariantSlice(DataSlice)
151     lower = upper
152     if lower >= length:
153         break
154 return invariant
155
156
157
158 def printtestinvariant(self,length,invariant):

```

```

159     #
160     a = self.alpha
161     #
162     assert length > 0
163     assert a > 1
164     #
165     invariant_sorted, indices = torch.sort(invariant, 1)
166     #
167     invariant_pre = invariant_sorted[:, 0:a-1]
168     invariant_post = invariant_sorted[:, 1:a]
169     invariant_delta = invariant_post - invariant_pre
170     #
171     assert ((invariant_delta >= 0).all(1)).all(0)
172     delta_avg = (invariant_delta.sum(1)).sum(0).to(torch.float) / (itf(length
173     #
174     delta_sum = (invariant_delta == 0).to(torch.int64).sum(1)
175     print("invariant delta average is", numpr(delta_avg, 1), "for length", itp(1
176     for k in range(a-1):
177         locnumber = (delta_sum == k).to(torch.int64).sum(0)
178         print("number of locations with delta sum", itp(k), "is", itp(locnumber
179     return
180
181
182     def matrixinvariant(self, Data, ivector, gvector):
183         #
184         a = self.alpha
185         #
186         length = Data['length']
187         #
188         eq, iz = self.geteq(Data)
189         #
190         vlength = len(ivector)
191         assert len(gvector) == vlength
192         #
193         irangevx = ivector.view(vlength, 1, 1, 1, 1).expand(vlength, a, a, a, a)
194         grangevx = gvector.view(vlength, 1, 1, 1, 1).expand(vlength, a, a, a, a)
195         xrangevx = arangeic(a).view(1, a, 1, 1, 1).expand(vlength, a, a, a, a)
196         yrangevx = arangeic(a).view(1, 1, a, 1, 1).expand(vlength, a, a, a, a)
197         zrangevx = arangeic(a).view(1, 1, 1, a, 1).expand(vlength, a, a, a, a)
198         wrangevx = arangeic(a).view(1, 1, 1, 1, a).expand(vlength, a, a, a, a)
199         #
200         xtransform = self.sga.grouptable[grangevx, xrangevx]
201         ytransform = self.sga.grouptable[grangevx, yrangevx]
202         ztransform = self.sga.grouptable[grangevx, zrangevx]
203         wtransform = self.sga.grouptable[grangevx, wrangevx]
204         #
205         eq_transform = eq[irangevx, xtransform, ytransform, ztransform, wtransform]
206         #
207         matrixvx = self.matrix.view(1, a, a, a, a).expand(vlength, a, a, a, a)
208         matrix_invariant = ((eq_transform.to(torch.int64)) * matrixvx).view(vlen
209         #
210         return matrix_invariant
211
212     def to_eqfunction(self, length, eq, iz):
213         #

```

```

214     a = self.alpha
215     a2 = a*a
216     #
217     eqview = eq.view(length*a2,a2)
218     izview = iz.view(length*a2)
219     #
220     numerical = arangeic(a2).view(1,a2).expand(length*a2,a2) + 1
221     numerical_eq = numerical * (eqview.to(torch.int64))
222     #
223     values,eqfunctionv = torch.max(numerical_eq,1)
224     eqfunctionv[izview] = a2
225     eqfunction = eqfunctionv.view(length,a2)
226     return eqfunction
227
228     def from_eqfunction(self,length,eqfunction):
229         #
230         #
231         a = self.alpha
232         a2 = a*a
233         #
234         eqf1vx = eqfunction.view(length,a2,1).expand(length,a2,a2)
235         eqf2vx = eqfunction.view(length,1,a2).expand(length,a2,a2)
236         #
237         eq = (eqf1vx == eqf2vx)
238         #
239         iz = (eqfunction.view(length,a2) == a2)
240         #
241         return eq,iz
242
243     def transform_eqfunction(self,length,eq,iz,gvector):
244         #
245         a = self.alpha
246         a2 = a*a
247         #
248         assert len(gvector)==length
249         #
250         eqv = eq.view(length,a,a,a,a)
251         izv = iz.view(length,a,a)
252         #
253         irangevx = arangeic(length).view(length,1,1,1,1).expand(length,a,a,a,a)
254         grangevx = gvector.view(length,1,1,1,1).expand(length,a,a,a,a)
255         xrangevx = arangeic(a).view(1,a,1,1,1).expand(length,a,a,a,a)
256         yrangevx = arangeic(a).view(1,1,a,1,1).expand(length,a,a,a,a)
257         zrangevx = arangeic(a).view(1,1,1,a,1).expand(length,a,a,a,a)
258         wrangevx = arangeic(a).view(1,1,1,1,a).expand(length,a,a,a,a)
259         #
260         xtransform = self.sga.grouptable[grangevx,xrangevx]
261         ytransform = self.sga.grouptable[grangevx,yrangevx]
262         ztransform = self.sga.grouptable[grangevx,zrangevx]
263         wtransform = self.sga.grouptable[grangevx,wrangevx]
264         #
265         eq_transform = eqv[xtransform,ytransform,ztransform,wtransform]
266         #
267         irangeZvx = arangeic(length).view(length,1,1).expand(length,a,a)
268         grangeZvx = gvector.view(length,1,1).expand(length,a,a)

```

```

269     xrangeZvx = arangeic(a).view(1,a,1).expand(length,a,a)
270     yrangeZvx = arangeic(a).view(1,1,a).expand(length,a,a)
271     #
272     xtransformZ = self.sga.grouptable[grangeZvx,xrangeZvx]
273     ytransformZ = self.sga.grouptable[grangeZvx,yrangeZvx]
274     #
275     iz_transform = izv[irangeZvx,xtransformZ,ytransformZ].view(length,a2)
276     #
277     eqfunction_transform = self.to_eqfunction(length,eq_transform,iz_transfo
278     return eqfunction_transform
279
280
281
282     def data_eqfunction_transform(self,Data,ivector,gvector):
283         #
284         a = self.alpha
285         a2 = a*a
286         #
287         DataVector = self.rri.indexselectdata(Data,ivector)
288         length = DataVector['length']
289         #
290         eq,iz = self.geteq(DataVector)
291         #
292         assert len(gvector) == length
293         #
294         #eqfunction = self.to_eqfunction(length,eq,iz)
295         #
296         eqfunction_transform = self.transform_eqfunction(length,eq,iz,gvector)
297         #
298         return eqfunction_transform
299
300     def uniqueinstances(self,length,eq_function):
301         #
302         a = self.alpha
303         a2= a*a
304         #
305         assert length > 0
306         #
307         eqflvx = eq_function.view(length,1,a2).expand(length,length,a2)
308         eqf2vx = eq_function.view(1,length,a2).expand(length,length,a2)
309         #
310         equivalent = (eqflvx == eqf2vx).all(2)
311         #
312         first = arangeic(length).view(length,1).expand(length,length)
313         second = arangeic(length).view(1,length).expand(length,length)
314         #
315         isrep = ((~equivalent) | (first <= second)).all(1)
316         #
317         unique_length = isrep.to(torch.int64).sum(0)
318         eq_unique = eq_function[isrep]
319         #
320         assert unique_length > 0
321         #
322         return unique_length,eq_unique
323

```

```

324
325
326 def addSlice(self,length,eq_function):
327     #
328     a = self.alpha
329     a2= a*a
330     #
331     ulength,eq_unique = self.uniqueinstances(length,eq_function)
332     #
333     alength = self.eqlength
334     #
335     if alength == 0:
336         self.eqlist = eq_unique
337         self.eqlength = ulength
338         return
339     alreadyvx = self.eqlist.view(1,alength,a2).expand(ulength,alength,a2)
340     newvx = eq_unique.view(ulength,1,a2).expand(ulength,alength,a2)
341     #
342     already_known = ( (alreadyvx == newvx).all(2) ).any(1)
343     #
344     detection = ~already_known
345     detected_length = detection.to(torch.int64).sum(0)
346     eq_detected = eq_unique[detection]
347     #
348     #
349     self.eqlist = torch.cat((self.eqlist,eq_detected),0)
350     #
351     self.eqlength += detected_length
352     #
353     return
354
355 def addinstances(self,length,eq_function):
356     #
357     if length == 0:
358         #print("no instances to add")
359         return
360     #
361     lower = 0
362     for i in range(length):
363         upper = lower + 500
364         if upper > length:
365             upper = length
366         length_slice = upper - lower
367         eq_slice = eq_function[lower:upper]
368         self.addSlice(length_slice,eq_slice)
369         lower = upper
370         if lower >= length:
371             break
372     return
373
374 def processBasic(self,Data):
375     #
376     a = self.alpha
377     assert a > 1
378     #
379     length = Data.shape[1]

```

```

379     length = Data['length']
380     print("current eqlength",itp(self.eqlength),"processing data of length",
381         #
382         eq,iz = self.geteq(Data)
383         #
384         eq_function = self.to_eqfunction(length,eq,iz)
385         #
386         self.addinstances(length,eq_function)
387         #
388         return
389
390     def process(self,Data):
391         #
392         a = self.alpha
393         assert a > 1
394         #
395         length = Data['length']
396         gl = self.sga.gtlength
397         #
398         invariant = self.orderinvariant(Data)
399         #
400         lrangevxr = arangeic(length).view(length,1,1).expand(length,gl,a).reshape
401         gtvxr =self.sga.grouptable.view(1,gl,a).expand(length,gl,a).reshape(leng
402         #
403         invariant_gt = invariant[lrangevxr,gtvxr]
404         detection = ((invariant_gt[:,0:a-1]) <= (invariant_gt[:,1:a])).all(1)
405         dlength = detection.to(torch.int64).sum(0)
406         ivector = (arangeic(length).view(length,1).expand(length,gl).reshape(len
407         gvector = (arangeic(gl).view(1,gl).expand(length,gl).reshape(length*gl)
408         #
409         verification = torch.zeros((length),dtype = torch.bool,device=Dvc)
410         verification[ivector] = True
411         #
412         assert verification.all(0)
413         #
414         eq_function = self.data_eqfunction_transform(Data,ivector,gvector)
415         #
416         self.addinstances(dlength,eq_function)
417         #
418         return
419
420     def checklocationSlice(self,length,eq_function):
421         #
422         a = self.alpha
423         a2 = a*a
424         #
425         location = torch.zeros((length),dtype = torch.int64,device=Dvc)
426         location[:] = -1
427         #
428         alength = self.eqlength
429         #
430         predetect_already = (self.eqlist.view(alength,a2)).sum(1)
431         predetect_current = (eq_function.view(length,a2)).sum(1)
432         predetect_already_vxr = predetect_already.view(alength,1).expand(alength
433         predetect_current_vxr = predetect_current.view(1,length).expand(alength,
434         #

```

```

435     predetection = (predetect_already_vxr == predetect_current_vxr)
436     #
437     alrangevvr = arangeic(alength).view(alength,1).expand(alength,length).re
438     lrangevvr = arangeic(length).view(1,length).expand(alength,length).resha
439     #
440     alrvector = alrangevvr[predetection]
441     currvector = lrangevvr[predetection]
442     #
443     eq_already = (self.eqlist.view(alength,a2))[alrvector]
444     eq_current = (eq_function.view(length,a2))[currvector]
445     #
446     detection = (eq_already == eq_current).all(1)
447     #
448     already_detected = alrvector[detection]
449     current_detected = currvector[detection]
450     #
451     location[current_detected] = already_detected
452     #
453     return location
454
455     def checklocation(self,length,eq_function):
456         #
457         a = self.alpha
458         a2 = a*a
459         #
460         location = torch.zeros((length),dtype = torch.int64,device=Dvc)
461         #
462         lower = 0
463         for i in range(length):
464             upper = lower + 100
465             if upper > length:
466                 upper = length
467             length_slice = upper - lower
468             eq_slice = eq_function[lower:upper]
469             location[lower:upper] = self.checklocationSlice(length_slice,eq_slic
470             lower = upper
471             if lower >= length:
472                 break
473         return location
474
475
476
477
478     def highestlocation(self,length,eq_function):
479         #
480         a = self.alpha
481         a2 = a*a
482         #
483         gl = self.sga.gtlength
484         #
485         eq_vxr = eq_function.view(length,1,a2).expand(length,gl,a2).reshape(leng
486         gvvector = arangeic(gl).view(1,gl).expand(length,gl).reshape(length*gl)
487         grouplength = length*gl
488         #
489         eq_iz = self.from eqfunction(grouplength,eq_vxr)

```

```

490     eq_transform = self.transform_eqfunction(grouplength,eq,iz,gvector)
491     #
492     location = self.checklocation(grouplength,eq_transform)
493     locationv = location.view(length,gl)
494     highest,indices = torch.max(locationv,1)
495     return highest
496
497     def sieve(self):
498         #
499         alength = self.eqlength
500         print("doing sieve on",itp(alength),"locations")
501         #
502         highest_location = torch.zeros((alength),dtype = torch.int64,device=Dvc)
503         #
504         lower = 0
505         for i in range(alength):
506             print("---",lower)
507             upper = lower + 100
508             if upper > alength:
509                 upper = alength
510             eq_slice = self.eqlist[lower:upper]
511             length_slice = upper - lower
512             #
513             highest_location[lower:upper] = self.highestlocation(length_slice,eq)
514             lower = upper
515             if lower >= alength:
516                 break
517         #
518         negative_detect = (highest_location < 0)
519         negative_count = negative_detect.to(torch.int64).sum(0)
520         print("unfortunate locations with negative values :",itp(negative_count))
521         alrange = arangeic(alength)
522         good_detect = (highest_location <= alrange)
523         good_count = good_detect.to(torch.int64).sum(0)
524         print("detected",itp(good_count),"good locations")
525         print("finished sieve")
526         return
527
528
529

```

```

1 class Learner :    # training the neural networks
2     def __init__(self,Rr4):
3         #
4         #
5         self.rr4 = Rr4
6         self.pp = self.rr4.pp
7         self.rr3 = self.rr4.rr3
8         self.rr2 = self.rr4.rr2
9         self.rr1 = self.rr4.rr1
10        self.alpha = self.pp.alpha
11        self.alpha2 = self.pp.alpha2
12        self.alpha3 = self.pp.alpha3
13        self.alpha3z = self.pp.alpha3z

```

```

14 self.beta = self.pp.beta
15 self.betaz = self.pp.betaz
16 #
17 #self.mm = Mm
18 self.explore_max = self.pp.explore_max
19 self.examples_max = self.pp.examples_max
20 self.new_examples_max = self.pp.new_examples_max
21 self.new_explore_max = self.pp.new_explore_max
22 self.outlier_max = self.pp.outlier_max
23 self.new_outliers_max = self.pp.new_outliers_max
24 #
25 self.trainingprint = True
26 #
27 # all the examples are by convention active (not done or impossible)
28 self.OutlierPrePool = self.rr1.nulldata()
29 self.ExplorePrePool = self.rr1.nulldata()
30 self.ExamplesPrePool = self.rr1.nulldata()
31 self.Examples = self.rr1.nulldata()
32 self.extent_log = None # log10 of the number of nodes below that node,
33 # so this number of nodes is never 0
34 self.localscores = None # at (x,y) it is log10 of the sum score over (x
35 #
36 #self.sga = SymmetricGroup(self.alpha)
37 #self.sgb = SymmetricGroup(self.beta)
38 #
39 self.globalL1level = 1.0
40
41
42 def pruneExamples(self,M): # remove the last ones, those were the earliest a
43 #
44 elength = self.Examples['length']
45 epplength = self.ExamplesPrePool['length']
46 xlength = self.ExplorePrePool['length']
47 olength = self.OutlierPrePool['length']
48 #
49 if elength > self.examples_max:
50     #self.specialPruneExamples(M)
51     permutation = torch.randperm(elength,device=Dvc)
52     indices = permutation[0:self.examples_max]
53     self.Examples = self.rr1.indexselectdata(self.Examples,indices)
54     self.extent_log = self.extent_log[indices]
55     self.localscores = self.localscores[indices]
56 if epplength > self.examples_max:
57     permutation = torch.randperm(epplength,device=Dvc)
58     indices = permutation[0:self.examples_max]
59     self.ExamplesPrePool = self.rr1.indexselectdata(self.ExamplesPrePool,
60 if xlength > self.explore_max:
61     permutation = torch.randperm(xlength,device=Dvc)
62     indices = permutation[0:self.explore_max]
63     self.ExplorePrePool = self.rr1.indexselectdata(self.ExplorePrePool,i
64 if olength > self.outlier_max:
65     permutation = torch.randperm(olength,device=Dvc)
66     indices = permutation[0:self.outlier_max]
67     self.OutlierPrePool = self.rr1.indexselectdata(self.OutlierPrePool,i
68 return

```

```

69
70
71 def check_availability(self,Data,comment):
72     #
73     prod = Data['prod']
74     #
75     available = (((prod.any(3)).all(2)).all(1)).all(0)
76     if not available:
77         print("with comment",comment)
78         raise CoherenceError("availability problem in data that should be ac
79     return
80
81
82
83 def prepoolSamples(self,M,Data,new_examples): # prepend new ones so that the
84     #
85     #
86     splength = Data['length']
87     #
88     if splength == 0:
89         return
90     permutation = torch.randperm(splength,device=Dvc)
91     upper = new_examples
92     if upper > splength:
93         upper = splength
94     indices = permutation[0:upper]
95     NewExamples = self.rr1.indexselectdata(Data,indices)
96     self.check_availability(NewExamples,"prepoolSamples")
97     self.ExamplesPrePool = self.rr1.appenddata(NewExamples,self.ExamplesPreP
98     #
99     self.pruneExamples(M)
100    return
101
102 def prepoolExplore(self,M,Data,new_examples): # prepend new ones so that the
103     #
104     #
105     splength = Data['length']
106     #
107     if splength == 0:
108         return
109     ppe_length = torch.round(itf(new_examples)/M.average_local_loss).to(torch
110     rectangle = arangeic(splength).view(splength,1).expand(splength,ppe_leng
111     permutation = torch.randperm(splength*ppe_length,device=Dvc)
112     upper = ppe_length
113     #
114     indices = rectangle[permutation[0:upper]]
115     NewExamples = self.rr1.indexselectdata(Data,indices)
116     self.check_availability(NewExamples,"prepoolExplore")
117     self.ExplorePrePool = self.rr1.appenddata(NewExamples,self.ExplorePrePoo
118     #
119     self.pruneExamples(M)
120    return
121
122 def transferexamples(self,M,TransferData,extent,localscore,epp_throw_detecti
123     # detection tells us the ones to remove from the epp
124     if self.Examples['length'] == 0:

```

```

124     if self.Examples['length'] == 0:
125         self.extent_log = extent
126         self.localscores = localscore
127     else:
128         self.extent_log = torch.cat((extent,self.extent_log),0)
129         self.localscores = torch.cat((localscore,self.localscores),0)
130     self.Examples = self.rr1.appenddata(TransferData,self.Examples)
131     #
132     keep_detection = ~epp_throw_detection
133     self.ExamplesPrePool = self.rr1.detectsubdata(self.ExamplesPrePool,keep_
134     #
135     delta = self.abs_diff_sup(M,TransferData,localscore)
136     seuil = self.pp.outlier_threshold * M.average_local_loss
137     NewOutliers = self.rr1.detectsubdata(TransferData,(delta > seuil))
138     self.OutlierPrePool = self.rr1.appenddata(NewOutliers,self.OutlierPrePoo
139     #
140     self.pruneExamples(M)
141     return
142
143     def scoreExamples(self,M):
144         epplength = self.ExamplesPrePool['length']
145         if epplength == 0:
146             print("no examples to locally score")
147             return
148         #
149         permutation = torch.randperm(epplength,device=Dvc)
150         upper = self.new_examples_max
151         if upper > epplength:
152             upper = epplength
153         indices = permutation[0:upper]
154         #
155         epp_throw_detection = torch.zeros((epplength),dtype = torch.bool,device=
156         epp_throw_detection[indices] = True
157         #
158         TransferData = self.rr1.indexselectdata(self.ExamplesPrePool,indices)
159         #
160         print("transferring data of length",itp(TransferData['length']))
161         #
162         xyscore_log, xyscore_min, LocalExamples = self.calculatescoresLocal(M,Tr
163         #
164         self.transferexamples(M,TransferData,xyscore_min,xyscore_log,epp_throw_d
165         #
166         self.check_availability(LocalExamples,"LocalExamples in scoreExamples")
167         self.prepoolExplore(M,LocalExamples,self.new_examples_max)
168         #
169         print("examples has size",itp(self.Examples['length']))
170         print("example pre pool has size",itp(self.ExamplesPrePool['length']))
171         return
172
173     def scoreExplore(self,M):
174         xlength = self.ExplorePrePool['length']
175         epplength = self.ExamplesPrePool['length']
176         if xlength == 0:
177             print("no examples to locally score")
178             return
179         #

```

```

180     permutation = torch.randperm(xlength,device=Dvc)
181     current_explore = 2*self.new_examples_max
182     if current_explore > self.new_explore_max:
183         current_explore = self.new_explore_max
184     upper = current_explore
185     if upper > xlength:
186         upper = xlength
187     indices = permutation[0:upper]
188     #
189     epp_throw_detection = torch.zeros((epplength),dtype = torch.bool,device=
190     #
191     TransferData = self.rrl.indexselectdata(self.ExplorePrePool,indices)
192     #
193     print("transferring explore data of length",itp(TransferData['length']))
194     #
195     xyscore_log, xyscore_min, LocalExamples = self.calculatescoresLocal(M,Tr
196     #
197     self.transferexamples(M,TransferData,xyscore_min,xyscore_log,epp_throw_d
198     #
199     self.check_availability(LocalExamples,"LocalExamples in scoreExplore")
200     self.prepoolExplore(M,LocalExamples,current_explore)
201     #
202     print("examples has size",itp(self.Examples['length']))
203     print("explore pre pool has size",itp(self.ExplorePrePool['length']))
204     return
205
206     def scoreOutlier(self,M):
207         xlength = self.OutlierPrePool['length']
208         epplength = self.ExamplesPrePool['length']
209         if xlength == 0:
210             print("no outliers to locally score")
211             return
212         #
213         permutation = torch.randperm(xlength,device=Dvc)
214         #
215         upper = self.new_outliers_max
216         if upper > xlength:
217             upper = xlength
218         indices = permutation[0:upper]
219         #
220         epp_throw_detection = torch.zeros((epplength),dtype = torch.bool,device=
221         #
222         TransferData = self.rrl.indexselectdata(self.OutlierPrePool,indices)
223         #
224         print("transferring outlier data of length",itp(TransferData['length']))
225         #
226         xyscore_log, xyscore_min, LocalExamples = self.calculatescoresLocal(M,Tr
227         #
228         delta = self.abs_diff_sup(M,TransferData,xyscore_log)
229         seuil = self.pp.outlier_threshold * M.average_local_loss
230         indices_throw = indices[(delta < seuil)]
231         throw_detection = torch.zeros((xlength),dtype = torch.bool,device=Dvc)
232         throw_detection[indices_throw] = True
233         self.OutlierPrePool = self.rrl.detectsubdata(self.OutlierPrePool,(~throw
234         #

```

```

235     self.transferexamples(M,TransferData,xyscore_min,xyscore_log,epp_throw_d
236     #
237     print("outlier pre pool has size",itp(self.OutlierPrePool['length']))
238     return
239
240     def abs_diff_sup(self,M,Data,xyscore_log):
241         #
242         a = self.alpha
243         a2 = self.alpha2
244         #
245         length = Data['length']
246         prod = Data['prod']
247         #
248         availablexyf = self.rr1.availablexy(length,prod).view(length,a,a)
249         net2 = M.network2(Data)
250         predicted = net2.view(length,a,a).detach()
251         delta_abs = torch.abs((availablexyf * (xyscore_log - predicted))).view(1
252         delta_sup,indices = torch.max(delta_abs,1)
253         return delta_sup
254
255
256     def addscoredexamples(self,M):
257         SamplePool = self.rr4.SamplePool
258         DroppedPool = self.rr4.DroppedSamplePool
259         #
260         splength = SamplePool['length']
261         dplength = DroppedPool['length']
262         #
263         sprectangle = SamplePool['info'][:,self.pp.sampleinfo.lower:self.pp.sampl
264         #
265         splrangevxr = arangeic(splength).view(splength,1).expand(splength,200).r
266         sprectangler = sprectangle.reshape(splength*200)
267         sp_detection = (sprectangler >= 0) & (sprectangler < splrangevxr)
268         #
269         ivector = splrangevxr[sp_detection]
270         jvector = sprectangler[sp_detection]
271         # note that jvector < ivector because of the second condition in sp_dete
272         # jvector is any previous location strictly above the ivector location i
273         #
274         incidence = torch.zeros((splength,splength),dtype = torch.float,device=D
275         #
276         incidence[ivector,jvector] = 1.
277         #
278         #
279         spnodes = incidence.sum(0) + 1. # this should be the number of nodes bel
280         #
281         if dplength > 0:
282             dprectangle = DroppedPool['info'][:,self.pp.sampleinfo.lower:self.pp.
283             #
284             dincidence = torch.zeros((dplength,splength),dtype = torch.float,dev
285             #
286             dplrangevxr = arangeic(dplength).view(dplength,1).expand(dplength,20
287             dprectangler = dprectangle.reshape(dplength*200)
288             dp_detection = (dprectangler >= 0)
289             #

```

```

290         idvector = dplrangevvr[dp_detection]
291         jdvector = dprectangler[dp_detection]
292         #
293         dincidence[idvector,jdvector] = 1.
294         #
295         #
296         dpextent_log = M.network(DroppedPool).detach()
297         # this approximates log10 of (the number of nodes at or below a drop
298         dpextent_log = torch.clamp(dpextent_log,0.,9.)
299         dpextent = (10**dpextent_log)
300         dpextentv = dpextent.view(1,dplength)
301         extent_transfer = (torch.matmul(dpextentv,dincidence)).view(splength)
302         #
303         extent = spnodes + extent_transfer
304     else:
305         extent = spnodes
306     #
307     logextent = torch.log10(extent)
308     #
309     #
310     permutation = torch.randperm(splength,device=Dvc)
311     upper = self.new_examples_max
312     if upper > splength:
313         upper = splength
314     indices = permutation[0:upper]
315     TransferData = self.rr1.indexselectdata(SamplePool,indices)
316     transfer_extent = logextent[indices]
317     #
318     epp_throw_detection = torch.zeros((self.ExamplesPrePool['length']),dtype
319     #
320     xyscore_log, xyscore_min, LocalExamples = self.calculatescoresLocal(M,Tr
321     #
322     positivephase = ( TransferData['info'][:,self.pp.phase] > 0 )
323     phased_extent = transfer_extent.clone()
324     phased_extent[positivephase] = xyscore_min[positivephase]
325     #
326     self.transferexamples(M,TransferData,phased_extent,xyscore_log,epp_throw
327     #
328     return
329
330
331
332     def noisetensor(self,thetensor):
333         #
334         length = len(thetensor)
335         tirage = torch.rand(length,device=Dvc)
336         noiselevel = HST.noiselevel(self.pp,torch.tensor(HST.training_counter,de
337         bruit = (tirage < noiselevel)
338         ntensor = ((~bruit) & thetensor) | (bruit & (~thetensor))
339         return ntensor
340
341
342     def noise(self,Data):
343         #
344         a = self.alpha

```

```

345     a2 = self.alpha2
346     a3 = self.alpha3
347     a3z = self.alpha3z
348     b = self.beta
349     bz = self.betaz
350     #
351     length = Data['length']
352     prodv = Data['prod'].view(length*a*a*bz)
353     leftv = Data['left'].view(length*a*bz*2)
354     rightv = Data['right'].view(length*bz*a*a*2)
355     ternaryv = Data['ternary'].view(length*a*a*a*2)
356     #
357     nprod = self.noisetensor(prodv).view(length,a,a,bz)
358     nleft = self.noisetensor(leftv).view(length,a,bz,2)
359     nright = self.noisetensor(rightv).view(length,bz,a,a,2)
360     nternary = self.noisetensor(ternaryv).view(length,a,a,a,2)
361     #
362     NoiseData = self.rri1.copydata(Data)
363     NoiseData['prod'] = nprod
364     NoiseData['left'] = nleft
365     NoiseData['right'] = nright
366     NoiseData['ternary'] = nternary
367     #
368     return NoiseData
369
370
371     def printexamplescores(self,number):
372         ExamplePool = self.Examples
373         xplength = ExamplePool['length']
374         xpdepth = ExamplePool['depth']
375         if xplength == 0:
376             print("no examples to print")
377             return
378         #
379         print("example pool has",itp(xplength),"elements")
380         #
381         permutation = torch.randperm(xplength,device=Dvc)
382         #
383         upper = number
384         if upper > xplength:
385             upper = xplength
386         for i in range(upper):
387             ip = permutation[i]
388             idepth = xpdepth[ip]
389             iextent = self.extent_log[ip]
390             print("sample number",itp(ip),"depth",itp(idepth),"log extent",numpr
391         return
392
393     def selectminibatch(self,minibatchsize):
394         ExamplePool = self.Examples
395         xplength = ExamplePool['length']
396         score = self.extent_log
397         if xplength < 10:
398             print("not enough examples to train on")
399             return False,None,None

```

```

400     #
401     permutation = torch.randperm(xplength,device=Dvc)
402     upper = minibatchsize
403     if upper > xplength:
404         upper = xplength
405     indices = permutation[0:upper]
406     DataBatch = self.rrl.indexselectdata(ExamplePool,indices)
407     scorebatch = score[indices]
408     return True,DataBatch,scorebatch
409
410
411
412 def trainingGlobal(self,M,numberofbatches,iterationsperbatch,style,minibatch
413     #
414     if style != 'score-A' and style != 'score-B' and style != 'score-C':
415         raise CoherenceError("only allowed styles are score-A or score-B or
416     #
417     if self.trainingprint:
418         print("/",style,numberofbatches,iterationsperbatch,partname,"/",end
419     for s in range(numberofbatches):
420         smb,DataBatch, scorebatch = self.selectminibatch(minibatchsize)
421         if not smb:
422             print("exit training")
423             return
424     #
425     for i in range(iterationsperbatch):
426         #
427         M.optimizer.zero_grad()
428         #
429         NoiseData = self.noise(DataBatch)
430         #
431         predictedscore = M.network(NoiseData)
432         #
433         if style == 'score-A':
434             loss = M.criterionA(predictedscore,scorebatch)
435         if style == 'score-B':
436             loss = M.criterionB(predictedscore,scorebatch)
437         if style == 'score-C':
438             lossA = M.criterionA(predictedscore,scorebatch)
439             lossB = M.criterionB(predictedscore,scorebatch)
440             loss = (lossA + lossB)/2
441         loss.backward()
442         M.optimizer.step()
443     #
444     #
445     print("-",end = ' ')
446     #
447     return
448
449 def printlossaftertrainingGlobal(self,M,minibatchsize,topicture):
450     #
451     smb,DataBatch,scorebatch = self.selectminibatch(minibatchsize)
452     if not smb:
453         print("data too small")
454     return
455     #

```

```

455 #
456 mblength = DataBatch['length']
457 predictedscore = M.network(DataBatch)
458 lossa= M.criterionA(predictedscore,scorebatch)
459 lra = numpr(lossa,3)
460 lossb = M.criterionB(predictedscore,scorebatch)
461 lrb = numpr(lossb,3)
462 #
463 with torch.no_grad():
464     self.globalL1level += lossa
465     self.globalL1level *= 0.5
466     self.globalL1level = torch.clamp(self.globalL1level,0.005,1.0)
467 #
468 print("on ",itp(mblength),"values network -- L1 loss",lra,"MSE loss",lrb)
469 #
470 if topicture:
471     #
472     print("global L1 loss level",numpr(self.globalL1level,4))
473     #
474     HST.record_loss('global',lossa,lossb)
475     #
476     dotsize = torch.zeros((mblength),dtype = torch.int,device=Dvc)
477     dotsize[:]=2
478     dotsize_np = numpr(dotsize)
479     #
480     calcscore_npr = numpr(scorebatch,3)
481     predscode_npr = numpr(predictedscore,3)
482     #
483     scoremax,index = torch.max(scorebatch,0)
484     linelimit = numpr(scoremax,1)
485     #
486     #
487     plt.clf()
488     plt.scatter(calcscore_npr,predscode_npr,dotsize_np)
489     #
490     plt.plot([0.0,linelimit],[0.0,0.0],'g-',lw=1)
491     plt.plot([0.0,0.0],[0.0,linelimit],'g-',lw=1)
492     plt.plot([0.0,linelimit],[0.0,linelimit],'r-',lw=1)
493     plt.show()
494     return
495
496 def learningGlobal(self,M,globaliterations):
497     #
498     self.printlossaftertrainingGlobal(M,500,True)
499     #
500     tweak_cursor = HST.global_tweak_cursor
501     tdensity = self.pp.tweak_density * (self.pp.tweak_decay ** tweak_cursor)
502     tepsilon = self.pp.tweak_epsilon * (self.pp.tweak_decay ** tweak_cursor)
503     HST.global_tweak_cursor += 1
504     print("tweaking global network at cursor",itp(tweak_cursor),"with densit
505     M.tweak_network(M.network,tdensity,tepsilon)
506     self.printlossaftertrainingGlobal(M,500,True)
507     print("training",end = ' ')
508     #
509     explore_pre_length = self.ExplorePrePool['length']
510     example_pre_length = self.ExamplesPrePool['length']

```

```

510     example_pre_length = self.Examples['pre_length']
511     example_length = self.Examples['length']
512     HST.record_training('global', globaliterations, explore_pre_length, example
513 #
514     for g in range(globaliterations):
515         print("/", end=' ')
516         self.trainingGlobal(M, 2, 20, 'score-C', 20, 'mb20')
517         self.trainingGlobal(M, 1, 30, 'score-C', 30, 'mb30')
518         self.trainingGlobal(M, 2, 10, 'score-C', 40, 'mb40')
519         self.trainingGlobal(M, 5, 10, 'score-C', 60, 'mb60')
520         self.trainingGlobal(M, 3, 8, 'score-C', 20, 'mb20')
521         self.trainingGlobal(M, 3, 5, 'score-C', 40, 'mb40')
522         self.trainingGlobal(M, 5, 3, 'score-C', 30, 'mb30')
523     #
524     print(" ")
525     self.printlossaftertrainingGlobal(M, 300, False)
526     print(" ")
527     self.printlossaftertrainingGlobal(M, 500, True)
528     print("===== end score training =====")
529     return
530
531 ##### Local stuff
532
533 def calculatetimesLocal(self, M, Data):
534     #
535     a = self.alpha
536     a2 = self.alpha2
537     a3 = self.alpha3
538     a3z = self.alpha3z
539     b = self.beta
540     bz = self.betaz
541     #
542     length = Data['length']
543     prod = Data['prod']
544     #
545     xypscore_exp = torch.zeros((length, a, a, bz), dtype = torch.float, device=Dv
546 #
547     availablexyp = self.rr1.availablexyp(length, prod)
548     availablexypr = availablexyp.reshape(length*a*a*bz)
549 #
550     lrangevxr = arangeic(length).view(length, 1, 1, 1).expand(length, a, a, bz).re
551     xrangevxr = arangeic(a).view(1, a, 1, 1).expand(length, a, a, bz).reshape(leng
552     yrangevxr = arangeic(a).view(1, 1, a, 1).expand(length, a, a, bz).reshape(leng
553     prangevxr = arangeic(bz).view(1, 1, 1, bz).expand(length, a, a, bz).reshape(le
554 #
555     ivector = lrangevxr[availablexypr]
556     xvector = xrangevxr[availablexypr]
557     yvector = yrangevxr[availablexypr]
558     pvector = prangevxr[availablexypr]
559 #
560     NewData = self.rr1.upsplitting(Data, ivector, xvector, yvector, pvector)
561 #
562 #
563     ndlength = NewData['length']
564 #
565 #

```

```

566     LocalExamples = self.rr1.nulldata()
567     detection = torch.zeros((ndlength), dtype = torch.bool, device=Dvc)
568     newextent_exp = torch.zeros((ndlength), dtype = torch.float, device=Dvc)
569     # that should be the (approximation of) the number of nodes below and in
570     newactive = torch.zeros((ndlength), dtype = torch.bool, device=Dvc)
571     lower = 0
572     for i in range(ndlength):
573         assert lower < ndlength
574         upper = lower + 1000
575         if upper > ndlength:
576             upper = ndlength
577         detection[:] = False
578         detection[lower:upper] = True
579         NewDataSlice = self.rr1.detectsubdata(NewData, detection)
580         AssocNewDataSlice = self.rr2.process(NewDataSlice)
581         newactive_s, newdone_s, newimpossible_s = self.rr2.filterdata(AssocNew
582         #
583         ActiveNewDataSlice = self.rr1.detectsubdata(AssocNewDataSlice, newact
584         LocalExamples = self.rr1.appenddata(ActiveNewDataSlice, LocalExamples
585         #
586         predictedscore_s = M.network(AssocNewDataSlice).detach()
587         if torch.isnan(predictedscore_s).any(0):
588             raise CoherenceException("predicted score nan")
589         # recall that approximates log10 of (the number of nodes below and i
590         predictedscore_s_clamp = torch.clamp(predictedscore_s, 0., 8.)
591         predictedscore_s_exp = 10.**predictedscore_s_clamp
592         predictedscore_s_exp[newdone_s] = 0.0
593         predictedscore_s_exp[newimpossible_s] = 0.1
594         newextent_exp[lower:upper] = predictedscore_s_exp
595         newactive[lower:upper] = newactive_s
596         lower = upper
597         if lower >= ndlength:
598             break
599     #
600     xypscore_exp[ivector, xvector, yvector, pvector] = newextent_exp
601     #
602     xyscore_sum = xypscore_exp.sum(3)
603     #
604     xyscore_log = torch.log10(xyscore_sum + 1.) # here the +1. is for the u
605     #
606     # now replace the global scores by these ones too: here output the min o
607     availablexyr = self.rr1.availablexy(length, prod).view(length*a2)
608     xyscorer = xyscore_log.view(length*a2)
609     xyscorer_mod = torch.clamp(xyscorer, 0., 8.)
610     xyscorer_mod[~availablexyr] = 20.
611     xyscore_min, xysm_indices = torch.min(xyscorer_mod.view(length, a2), 1)
612     assert (xyscore_min < 10.).all(0)
613     #
614     return xyscore_log, xyscore_min, LocalExamples
615
616
617 def printsomelocalscores(self, howmany):
618     elength = self.Examples['length']
619     if elength == 0:
620         print("no examples")

```

```

621         return
622         lsk = self.localscores_known
623         detection = lsk
624         detection_length = detection.to(torch.int64).sum(0)
625         if detection_length == 0:
626             print("no known score locations to print")
627             return
628         ivector = arangeic(elength)[detection]
629         permutation = torch.randperm(detection_length,device=Dvc)
630         upper = howmany
631         if upper > detection_length:
632             upper = detection_length
633         indices_pre = permutation[0:upper]
634         indices = ivector[indices_pre]
635         #
636         assert detection[indices].all(0)
637         #
638         for i in range(upper):
639             indexi = indices[i]
640             lsi = self.localscores[indexi]
641             print(numpr(lsi,2))
642         return
643
644     def predictedscoreLocal(self,M,ivector,xvector,yvector):
645         #
646         a = self.alpha
647         a2 = self.alpha2
648         a3 = self.alpha3
649         a3z = self.alpha3z
650         b = self.beta
651         bz = self.betaz
652         #
653         #
654         length = self.Examples['length']
655         prod = self.Examples['prod']
656         #
657         availablexy = self.rr1.availablexy(length,prod).view(length,a,a)
658         #
659         assert availablexy[ivector,xvector,yvector].all(0)
660         #
661         Data = self.rr1.indexselectdata(self.Examples,ivector)
662         dlength = Data['length']
663         dlrage = arangeic(dlength)
664         #
665         NoiseData = self.noise(Data)
666         #
667         pre_score = M.network2(NoiseData)
668         #
669         dlrangevxa = dlrage.view(dlength,1).expand(dlength,a)
670         arangevx = arangeic(a).view(1,a).expand(dlength,a)
671         #
672         predictedscore = pre_score[dlrange,xvector,yvector]
673         return predictedscore
674
675

```

```

676     def adapt_local_scores(self, ivector, xvector, yvector):
677         #
678         a = self.alpha
679         a2 = self.alpha2
680         a3 = self.alpha3
681         a3z = self.alpha3z
682         b = self.beta
683         bz = self.betaz
684         #
685         ExamplePool = self.Examples
686         #
687         length = len(ivector)
688         prod = (ExamplePool['prod'])[ivector]
689         availablexyv = self.rr1.availablexy(length, prod).reshape(length*a*a)
690         #
691         available_count = availablexyv.view(length, a*a).to(torch.int64).sum(1)
692         available_count_xf = available_count.view(length, 1).expand(length, a*a).t
693         available_count_xf -= 1.
694         available_count_xf = torch.clamp(available_count_xf, 1., 100.)
695         #
696         score = self.localscores[ivector].reshape(length*a*a)
697         score[~availablexyv] = 100.
698         values, indices = torch.sort(score.view(length, a*a), 1)
699         #
700         position = torch.zeros((length, a*a), dtype = torch.float, device=Dvc)
701         #
702         lrangevx = arangeic(length).view(length, 1).expand(length, a*a)
703         a2rangevx = arangeic(a*a).view(1, a*a).expand(length, a*a)
704         position[lrangevx, indices] = a2rangevx.to(torch.float) / available_count
705         #
706         position_score = position + score.view(length, a*a)
707         #
708         adapted_score = position_score.view(length, a, a)[arangeic(length), xvector
709         return adapted_score
710
711     def selectminibatchLocal(self, minibatchsize):
712         #
713         a = self.alpha
714         a2 = self.alpha2
715         a3 = self.alpha3
716         a3z = self.alpha3z
717         b = self.beta
718         bz = self.betaz
719         #
720         ExamplePool = self.Examples
721         xplength = ExamplePool['length']
722         if xplength == 0:
723             return False, None, None, None, None
724         xpprod = ExamplePool['prod']
725         xp_availablexy = self.rr1.availablexy(xplength, xpprod).view(xplength, a, a)
726         #
727         irangevxr = arangeic(xplength).view(xplength, 1, 1).expand(xplength, a, a).r
728         xrangevxr = arangeic(a).view(1, a, 1).expand(xplength, a, a).reshape(xplengt
729         yrangevxr = arangeic(a).view(1, 1, a).expand(xplength, a, a).reshape(xplengt
730         #

```

```

731     avdetect = xp_availablexy[irangevxr,xrangevxr,yrangevxr]
732     #
733     ivector_all = irangevxr[avdetect]
734     xvector_all = xrangevxr[avdetect]
735     yvector_all = yrangevxr[avdetect]
736     #
737     avlength = avdetect.to(torch.int64).sum(0)
738     #
739     permutation = torch.randperm(avlength,device=Dvc)
740     mblength = minibatchsize
741     if mblength > avlength:
742         mblength = avlength
743     indices = permutation[0:mblength]
744     #
745     ivector = ivector_all[indices]
746     xvector = xvector_all[indices]
747     yvector = yvector_all[indices]
748     #
749     scorebatch = self.adapt_local_scores(ivector,xvector,yvector)
750     #
751     return True,ivector,xvector,yvector,scorebatch
752
753 def trainingLocal(self,M,numberofbatches,iterationsperbatch,style,minibatchs
754     #
755     a = self.alpha
756     #
757     if style != 'score-A' and style != 'score-B' and style != 'score-C':
758         raise CoherenceError("only allowed styles are score-A or score-B or
759     #
760     if self.trainingprint:
761         print("/",style,numberofbatches,iterationsperbatch,partname,"/",end
762     for s in range(numberofbatches):
763         smb,ivector,xvector,yvector,scorebatch = self.selectminibatchLocal(m
764         if not smb:
765             print("exit training")
766             return
767         #
768         for i in range(iterationsperbatch):
769             #
770             M.optimizer2.zero_grad()
771             #
772             predictedscore = self.predictedscoreLocal(M,ivector,xvector,yvec
773             #
774             if style == 'score-C':
775                 lossA = M.criterionA(predictedscore,scorebatch)
776                 lossB = M.criterionB(predictedscore,scorebatch)
777                 loss = (lossA + lossB) / 2.
778                 loss.backward()
779                 M.optimizer2.step()
780             #
781             #
782             print("-",end = ' ')
783             #
784             return
785
786 def printlossoftentrainingscoreLocal(self,M,minibatchsize,partname):

```

```

786     def printlossaftertrainingLocal(self,M,minibatchsize,topicture):
787         #
788         a=M.pp.alpha
789         #
790         smb,ivector,xvector,yvector,scorebatch = self.selectminibatchLocal(minib
791         if not smb:
792             print("data too small")
793             return
794         #
795         mblength = len(ivector)
796         #
797         predictedscore = self.predictedscoreLocal(M,ivector,xvector,yvector)
798         #
799         lossa= M.criterionA(predictedscore,scorebatch)
800         lra = numpr(lossa,3)
801         #
802         lossb = M.criterionB(predictedscore,scorebatch)
803         lrb = numpr(lossb,3)
804         #
805         lossa_detach = lossa.detach()
806         M.average_local_loss = (0.9 * M.average_local_loss + 0.1 * lossa_detach)
807         #
808         print("on ",itp(mblength),"values network -- L1 loss",lra,"MSE loss",lrb)
809         #
810         if topicture:
811             #
812             HST.record_loss('local',lossa,lossb)
813             #
814             print("average local loss",numpr(M.average_local_loss,4))
815             #
816             dotsize = torch.zeros((mblength),dtype = torch.int,device=Dvc)
817             dotsize[:]=2
818             dotsize_np = nump(dotsize)
819             #
820             calcscore_npr = numpr(scorebatch,3)
821             predscode_npr = numpr(predictedscore,3)
822             #
823             scoremax,index = torch.max(scorebatch,0)
824             linelimit = numpr(scoremax,1)
825             #
826             plt.clf()
827             plt.scatter(calcscore_npr,predscode_npr,dotsize_np)
828             #
829             #linelimit = 1.0
830             plt.plot([0.0,linelimit],[0.0,0.0],'g-',lw=1)
831             plt.plot([0.0,0.0],[0.0,linelimit],'g-',lw=1)
832             plt.plot([0.0,linelimit],[0.0,linelimit],'r-',lw=1)
833             #
834             plt.show()
835         return
836
837     def learningLocal(self,M,globaliterations):
838         #
839         self.printlossaftertrainingLocal(M,500,True)
840         #
841         tweak_cursor = HST.local_tweak_cursor

```

```

841         tweak_cursor = HST.local_tweak_cursor
842         tdensity = self.pp.tweak_density * (self.pp.tweak_decay ** tweak_cursor)
843         tepsilon = self.pp.tweak_epsilon * (self.pp.tweak_decay ** tweak_cursor)
844         HST.local_tweak_cursor += 1
845         print("tweaking local network at cursor",itp(tweak_cursor),"with density
846         M.tweak_network(M.network2,tdensity,tepsilon)
847         self.printlossaftertrainingLocal(M,500,True)
848         print("training",end = ' ')
849         #
850         explore_pre_length = self.ExplorePrePool['length']
851         example_pre_length = self.ExamplesPrePool['length']
852         example_length = self.Examples['length']
853         HST.record_training('local',globaliterations,explore_pre_length,example_
854         #
855         for g in range(globaliterations):
856             print("/",end=' ')
857             self.trainingLocal(M,3,20,'score-C',20,'mb20')
858             self.trainingLocal(M,1,15,'score-C',30,'mb30')
859             self.trainingLocal(M,3,4,'score-C',60,'mb60')
860             self.trainingLocal(M,3,10,'score-C',40,'mb40')
861             self.trainingLocal(M,3,3,'score-C',20,'mb20')
862             self.trainingLocal(M,3,2,'score-C',40,'mb40')
863             self.trainingLocal(M,3,1,'score-C',30,'mb30')
864             #
865             print(" ")
866             self.printlossaftertrainingLocal(M,300,False)
867             print(" ")
868             self.printlossaftertrainingLocal(M,500,True)
869             print("=====  

870             return
871

```

```

1 class Driver :      # to run everything, it includes the sieve for instances sigma
2     def __init__(self,P):
3         #
4         #
5         self.Pp = P
6         self.rr4 = Relations4(self.Pp)
7         self.rr3 = self.rr4.rr2
8         self.rr2 = self.rr4.rr2
9         self.rr1 = self.rr4.rr1
10        self.alpha = self.Pp.alpha
11        self.alpha2 = self.Pp.alpha2
12        self.alpha3 = self.Pp.alpha3
13        self.alpha3z = self.Pp.alpha3z
14        self.beta = self.Pp.beta
15        self.betaz = self.Pp.betaz
16        #
17        self.sga = SymmetricGroup(self.alpha)
18        #
19        self.zbinatable = self.makezbinatable()
20        #
21        self.init_length,self.init_left_table = self.make_init_left_table()
22        #
23        self.donecount_collection = 0

```

```

24     self.ECN_collection = 0.
25     self.ECN_average = 0.
26     #
27     self.Cc = Classifier(self.Pp)
28     #
29     self.Ll = Learner(self.rr4)
30     #
31     HST.record_driver(self.alpha,self.beta)
32
33
34
35 def printprod(self,prod,loc):
36     #
37     a=self.alpha
38     a2=a*a
39     a3=a*a*a
40     a3z = a3+1
41     b=self.beta
42     bz = b+1
43     #
44     prodi = prod[loc]
45     prarray = torch.zeros((a,a),dtype = torch.int64,device=Dvc)
46     for x in range(a):
47         for y in range(a):
48             column = prod[loc,x,y]
49             prarray[x,y] = self.printcolumn(column)
50     print(nump(prarray))
51     return
52
53 def printcolumn(self,column):
54     #
55     a=self.alpha
56     a2=a*a
57     a3=a*a*a
58     a3z = a3+1
59     b=self.beta
60     bz = b+1
61     #
62     assert len(column) == bz
63     #
64     column_sum = column.to(torch.int64).sum(0)
65     #
66     if column_sum == 0:
67         return -8
68     #
69     if column_sum == 1:
70         value,prvalue = torch.max(column.to(torch.int64),0)
71         return prvalue
72     if column_sum == bz:
73         return -1
74     exponents = arangeic(bz)
75     powers = 10**exponents
76     prvalue = (column.to(torch.int64) * powers).sum(0)
77     prvalue += 3 * (10 ** bz)
78     return prvalue

```

```

79
80     def printcolumn2(self,column):
81         #
82         assert len(column) == 2
83         #
84         column_sum = column.to(torch.int64).sum(0)
85         #
86         if column_sum == 0:
87             return -8
88         if column_sum == 2:
89             return 3
90         #
91         return column[1]
92
93     def printleft(self,left,loc):
94         #
95         a=self.alpha
96         a2=a*a
97         a3=a*a*a
98         a3z = a3+1
99         b=self.beta
100        bz = b+1
101        #
102        prarray = torch.zeros((a,bz),dtype = torch.int64,device=Dvc)
103        for x in range(a):
104            for y in range(bz):
105                column = left[loc,x,y]
106                prarray[x,y] = self.printcolumn2(column)
107        print(numpy(prarray))
108        return
109
110    def printright(self,right,loc):
111        #
112        a=self.alpha
113        a2=a*a
114        a3=a*a*a
115        a3z = a3+1
116        b=self.beta
117        bz = b+1
118        #
119        prarray = torch.zeros((bz,a),dtype = torch.int64,device=Dvc)
120        for x in range(bz):
121            for y in range(a):
122                column = right[loc,x,y]
123                prarray[x,y] = self.printcolumn2(column)
124        print(numpy(prarray))
125        return
126
127    def print_prod_left_right(self,Data,i,as_sigma):
128        prod = Data['prod']
129        left = Data['left']
130        right = Data['right']
131        #
132        print("-----")
133        print("at instance",itp(as_sigma),"the prod, left and right are respecti

```

```

134     self.printprod(prod,i)
135     self.printleft(left,i)
136     self.printright(right,i)
137     print("-----")
138     return
139
140     def print_just_left(self,Data,i,as_sigma):
141         left = Data['left']
142         #
143         print("-----")
144         print("at instance",itp(as_sigma),"the left multiplication matrix is")
145         self.printleft(left,i)
146         print("-----")
147         return
148
149
150     #####
151
152     def makezbinatable(self):
153         #
154         a = self.alpha
155         #
156         power = 2**a
157         #
158         zbatable = torch.zeros((power,a),dtype = torch.bool,device=Dvc)
159         for z in range(power):
160             zbatable[z,:] = zbinary(a,z)
161         return zbatable
162
163     def collection(self,m): # this doesn't work perfectly, it needs to be re-si
164         #
165         a = self.alpha
166         a2 = self.alpha2
167         a3 = self.alpha3
168         a3z = self.alpha3z
169         b = self.beta
170         bz = self.betaz
171         #
172         power = 2**a
173         gl = self.sga.gtlength
174         #
175         gtbin = self.sga.gtbinary
176         #
177         if m <= 0:
178             print("m <= 0 not allowed")
179             raise CoherenceError("exiting")
180         if m == 1:
181             zrangepv = arangeic(power).view(1,power).expand(gl,power)
182             detection = (gtbin >= zrangepv).all(0)
183             clength = detection.to(torch.int64).sum(0)
184             collec = arangeic(power)[detection].view(clength,m)
185             #
186             zbatablev = self.zbinatable.view(power,1,a)
187             collec_bin = zbatablev[detection]
188             #
189             previous_possibilities = torch.ones((clength,power),dtype = torch.bo

```

```

187     previous_possibilities = torch.ones((clength,power),dtype = torch.bo
190     #
191     previous_subgroup = torch.ones((clength,gl),dtype = torch.bool,devic
192     #
193     else:
194         cp,collec_prev,collec_bin_prev,poss_prev,subgroup_prev = self.collec
195         #
196         detection_prev = poss_prev.view(cp*power)
197         #
198         subgroup_prev_vxr = subgroup_prev.view(cp,1,gl).expand(cp,power,gl).
199         z_current = arangeic(power).view(1,power,1).expand(cp,power,gl).resh
200         g_current = arangeic(gl).view(1,gl).expand(cp*power,gl)
201         detection_current = ((~subgroup_prev_vxr) | ( gtbin[g_current,z_curr
202         #
203         detection = detection_prev & detection_current
204         #
205         clength = detection.to(torch.int64).sum(0)
206         collec_prev_next = collec_prev.view(cp,1,m-1).expand(cp,power,m-1).r
207         zrangevxr = arangeic(power).view(1,power,1).expand(cp,power,1).resha
208         new_prev = collec_prev_next[detection]
209         zvector = zrangevxr[detection]
210         collec = torch.cat((new_prev,zvector),1)
211         #
212         collec_bin_prev_next = collec_bin_prev.view(cp,1,m-1,a).expand(cp,po
213         new_bin_prev = collec_bin_prev_next[detection]
214         zbatalevxr = self.zbinatable.view(1,power,1,a).expand(cp,power,1,a)
215         zbavector = zbatalevxr[detection]
216         collec_bin = torch.cat((new_bin_prev,zbavector),1)
217         #
218         poss_prev_vxr = poss_prev.view(cp,1,power).expand(cp,power,power).re
219         previous_possibilities = poss_prev_vxr[detection]
220         #
221         subgroup_prev_vxr = subgroup_prev.view(cp,1,gl).expand(cp,power,gl).
222         previous_subgroup = subgroup_prev_vxr[detection]
223         #
224         grange_vx = arangeic(gl).view(1,gl,1).expand(clength,gl,m)
225         collec_vx = collec.view(clength,1,m).expand(clength,gl,m)
226         transform = gtbin[grange_vx,collec_vx]
227         transform_sort,t_indices = torch.sort(transform,2)
228         #
229         subgroup = (collec_vx == transform_sort).all(2)
230         #
231         #
232         next_transform = gtbin.view(1,gl,power).expand(clength,gl,power)
233         prev_bound = (collec[:,m-1]).view(clength,1,1).expand(clength,gl,power)
234         prev_subgroupvx = previous_subgroup.view(clength,gl,1).expand(clength,gl
235         #
236         next_possib_prev = ( (~prev_subgroupvx) | (prev_bound <= next_transform)
237         possibilities = next_possib_prev & previous_possibilities
238         #
239         return clength,collec,collec_bin,possibilities,subgroup
240
241     def collectiontest(self,amount):
242         #
243         a = self.alpha
244         a2 = self.alpha2

```

```

245     a3 = self.alpha3
246     a3z = self.alpha3z
247     b = self.beta
248     bz = self.betaz
249     #
250     #
251     clength,collec,collec_bin,possibilities,subgroup = self.collection(b)
252     print("collection has length",itp(clength))
253     upper = 20
254     if upper > clength:
255         upper = clength
256     print("first",itp(upper),"elements are as follows")
257     #
258     collec_sum = (collec_bin.to(torch.int64).sum(2)).sum(1)
259     collec_sum1 = collec_bin.to(torch.int64).sum(1)
260     collec_sum2 = collec_bin.to(torch.int64).sum(2)
261     for q in range(a*b+1):
262         freq = (collec_sum == q).to(torch.int64).sum(0)
263         print("for amount",itp(q),"frequency",itp(freq))
264     amount_detect = (collec_sum == amount)
265     #
266     ad_freq = amount_detect.to(torch.int64).sum(0)
267     collec_detect = collec_bin[amount_detect]
268     print("ad freq",itp(ad_freq))
269     for i in range(ad_freq):
270         print("-----")
271         print(numpy(collec_detect[i]))
272         print("collec_sum1",numpy((collec_sum1[amount_detect])[i]))
273         print("collec_sum2",numpy((collec_sum2[amount_detect])[i]))
274     return
275
276 def lex_lt(self,width,z1,z2):
277     #
278     assert width > 0
279     #
280     if width == 1:
281         z1new = z1[:,0]
282         z2new = z2[:,0]
283         lt = (z1new < z2new)
284         return lt
285     z1prev = z1[:,0:width-1]
286     z2prev = z2[:,0:width-1]
287     #
288     lt_prev = self.lex_lt(width-1,z1prev,z2prev)
289     #
290     eq_prev = (z1prev == z2prev).all(1)
291     #
292     z1new = z1[:,width-1]
293     z2new = z2[:,width-1]
294     lt = ( lt_prev | (eq_prev & (z1new < z2new)) )
295     return lt
296
297
298 def collection_sieve(self):
299     #

```

```

300     a = self.alpha
301     a2 = self.alpha2
302     a3 = self.alpha3
303     a3z = self.alpha3z
304     b = self.beta
305     bz = self.betaz
306     #
307     power = 2**a
308     gl = self.sga.gtlength
309     #
310     gtbin = self.sga.gtbinary
311     #
312     clength,collec,collec_bin,possibilities,subgroup = self.collection(b)
313     #
314     collevxr = collec.view(clength,1,b).expand(clength,gl,b).reshape(clengt
315     grangevxr = arangeic(gl).view(1,gl,1).expand(clength,gl,b).reshape(cleng
316     #
317     transform = gtbin[grangevxr,collevxr]
318     transform_sort, t_indices = torch.sort(transform,1)
319     #
320     transform_ltv = self.lex_lt(b,transform_sort,collevxr)
321     transform_lt = transform_ltv.view(clength,gl)
322     #
323     throw = transform_lt.any(1)
324     #
325     detection = (~throw)
326     sieved_length = detection.to(torch.int64).sum(0)
327     sieved_collection = collec[detection]
328     sieved_collection_bin = collec_bin[detection]
329     #
330     return sieved_length, sieved_collection, sieved_collection_bin
331
332     def sieve_test(self):
333         sieved_length, sieved_collection, sieved_collection_bin = self.collectio
334         print("sieved collection has length",itp(sieved_length))
335         return
336
337
338     def make_init_left_table(self):
339         #
340         a = self.alpha
341         a2 = self.alpha2
342         a3 = self.alpha3
343         a3z = self.alpha3z
344         b = self.beta
345         bz = self.betaz
346         #
347         length, sieved_collection, sieved_collection_bin = self.collection_sieve
348         #
349         init_left_table = torch.zeros((length,a,bz,2),dtype = torch.bool,device=
350         #
351         left_value = sieved_collection_bin.permute(0,2,1)
352         init_left_table[:, :, 0:b, 1] = left_value
353         init_left_table[:, :, 0:b, 0] = ~left_value
354         init_left_table[:, :, b, 0] = True

```

```

355     #
356     print(" ")
357     print("available left table instances are 0 <= sigma <",itp(length))
358     print("    ---> these should be noted as the possible values of sigma for
359     #
360     zerocolumn = (~left_value).all(1)
361     zerocolumn_number = zerocolumn.to(torch.int64).sum(1)
362     overhalf = (2*zerocolumn_number > b)
363     overhalf_indices = arangeic(length)[overhalf]
364     print("    ")
365     print("locations with > half zero columns are",numpy(overhalf_indices))
366     print("    ---> it is suggested not to use the sigma instances in this li
367     print("    ")
368     #
369     return length,init_left_table
370
371     #####
372
373
374
375     def initialdata(self,instancevector,dropoutlimit):
376         #
377         a = self.alpha
378         a2 = self.alpha2
379         a3 = self.alpha3
380         a3z = self.alpha3z
381         b = self.beta
382         bz = self.betaz
383         #
384         length = len(instancevector)
385         prod = torch.ones((length,a,a,bz),dtype = torch.bool,device=Dvc)
386         #
387         left = self.init_left_table[instancevector]
388         right = torch.ones((length,bz,a,2),dtype = torch.bool,device=Dvc)
389         right[:,b,:,1] = False
390         #
391         if self.Pp.verbose:
392             print("initial prod at 0")
393             self.printprod(prod,0)
394             print("initial left at 0")
395             print(numpy(left[0,:,:,:1]))
396             print("initial right at 0")
397             print(numpy(right[0,:,:,:1]))
398         #
399         depth = torch.zeros((length),dtype = torch.int,device=Dvc)
400         #
401         ternary = torch.ones((length,a,a,a,2),dtype = torch.bool,device=Dvc)
402         #
403         info = torch.zeros((length,self.Pp.infosize),dtype = torch.int64,device=
404         info[:,self.Pp.sampleinfollower:self.Pp.sampleinfoupper] = -1
405         #
406         #
407         RawData = {
408             'length': length,
409             'depth': depth,

```

```

410         'prod': prod,
411         'left': left,
412         'right': right,
413         'ternary': ternary,
414         'info': info,
415     }
416     #
417     if dropoutlimit > 0:
418         rectangle = arangeic(length).view(length,1).expand(length,dropoutlim
419         index_slice = (torch.randperm(length*dropoutlimit,device=Dvc))[0:dro
420         indices = rectangle[index_slice]
421         AugmentedData = self.rr1.indexselectdata(RawData,indices)
422         # set phase
423         tirage = torch.rand((dropoutlimit),device = Dvc)
424         phasel_upper = 0.8 * self.Pp.splitting_probability
425         phasel2_upper = 0.8
426         phasel = (tirage < phasel_upper)
427         phase2 = (tirage < phasel2_upper) & (~phase1)
428         AugmentedData['info'][:,self.Pp.phase][phase2] = 2
429         AugmentedData['info'][:,self.Pp.phase][phase1] = 1
430         return AugmentedData
431     return RawData
432
433     def print_instances(self):
434         #
435         instancevector, training_instances, proof_title = self.instance_chooser(
436         InitialData = self.initialdata(instancevector,0)
437         length = InitialData['length']
438         print(proof_title)
439         print("initial data from this collection of instances has length",itp(le
440         for i in range(length):
441             as_sigma = instancevector[i]
442             #self.print_prod_left_right(InitialData,i,as_sigma)
443             self.print_just_left(InitialData,i,as_sigma)
444         print("- - - - -")
445         return
446
447
448     def classificationproof(self,Mstrat,Mlearn,dropoutlimit,proving_instances,ti
449         print("---   ---   ---   ---   ---   ---   ---   ---   ---")
450         print("           classification proof")
451         print("---   ---   ---   ---   ---   ---   ---   ---   ---")
452         #
453         HST.title_text_sigma_proof = title_text
454         #
455         self.rr4.proofnumber = 0
456         self.rr4.proofinstance = 0
457         self.rr4.allnumbers = 1
458         #
459         if dropoutlimit == 0:
460             HST.reset_current_proof()
461         #
462         self.Cc.initialize()
463         #
464         InitialData = self.initialdata(proving_instances,dropoutlimit)

```

```

465 #
466 if dropoutlimit > 0:
467     AssocInitialData = self.rr2.process(InitialData)
468     activedetect,donedetect,impossibledetect = self.rr2.filterdata(Assoc
469     ActiveInitialData = self.rr1.detectsubdata(AssocInitialData,activede
470 #
471     explore_upper = self.Pp.root_injection
472     if explore_upper > dropoutlimit:
473         explore_upper = dropoutlimit
474     self.Ll.prepoolExplore(Mlearn,ActiveInitialData,explore_upper)
475 #
476 pl,ActivePool,DonePool,prooflength = self.rr4.proofloop(Mstrat,Mlearn,se
477 #
478 print("---   ---   ---   ---   ---   ---   ---   ---")
479 print("this proof was treating alpha =",itp(self.alpha),"beta =",itp(sel
480 print("proof ended after step number",itp(prooflength))
481 if ActivePool['length'] > 0:
482     print("proof outputs Active Data of length",itp(ActivePool['length']
483 print("proof has done count",itp(self.rr4.doncount),end=' ')
484 print("and estimated cumulative nodes",numpr(self.rr4.ECN,1))
485 self.doncount_collection += self.rr4.doncount
486 self.ECN_collection += self.rr4.ECN
487 print("classifier eq pool has length",itp(self.Cc.eqlength))
488 #
489 if dropoutlimit == 0:
490     if Mstrat.benchmark:
491         HST.record_current_proof(benchmark = True)
492     else:
493         HST.record_current_proof()
494 #
495 print("---   ---   ---   ---   ---   ---   ---   ---")
496 print("           classification proof done")
497 print("---   ---   ---   ---   ---   ---   ---   ---")
498 print("===  ===  ===  ===  ===  ===  ===  ===  ===  ===  ===")
499 #
500 return
501
502 ##### mini programs for creation of the instancevector_title object (it is re
503
504 def InAll(self):
505     instance_vector = arangeic(self.init_length)
506 #
507     title_text = F'for all sigma instances'
508 #
509     return instance_vector, instance_vector, title_text
510
511 def InOne(self,instance):
512     assert 0 <= instance < self.init_length
513     instance_vector = torch.zeros((1),dtype = torch.int64,device=Dvc)
514     instance_vector[0] = instance
515 #
516     title_text = F'for sigma instance {instance}'
517 #
518     return instance_vector, instance_vector, title_text
519
520 def InSeq(self,lower_upper):

```

```

520 def inSeg(self, lower, upper):
521     assert 0 <= lower < self.init_length
522     assert lower < upper
523     if upper > self.init_length:
524         print("retracting the upper value to", self.init_length)
525     upper_mod = upper
526     if upper_mod > self.init_length:
527         upper_mod = self.init_length
528     instance_vector = arangeic(self.init_length)[lower:upper]
529     #
530     title_text = F'for sigma instances in range {lower}:{upper_mod}'
531     #
532     return instance_vector, instance_vector, title_text
533
534 def InSkip(self, skip, lower, upper):
535     assert 0 <= lower < self.init_length
536     assert lower < upper
537     upper_mod = upper
538     if upper_mod > self.init_length:
539         upper_mod = self.init_length
540     detection = torch.zeros((self.init_length), dtype = torch.bool, device=Dvc)
541     detection[lower:upper] = True
542     detection[skip] = False
543     training_vector = arangeic(self.init_length)[detection]
544     #
545     proving_vector = torch.zeros((1), dtype = torch.int64, device=Dvc)
546     proving_vector[0] = skip
547     #
548     title_text = F'training for sigma in range {lower}:{upper} skipping and
549     #
550     return proving_vector, training_vector, title_text
551
552 def InList(self, proving_list, training_list):
553     proving_vector = torch.tensor(proving_list, dtype = torch.int64, device=Dvc)
554     training_vector = torch.tensor(training_list, dtype = torch.int64, device=
555     #
556     title_text = F'training for sigma instances in list {training_list} and
557     #
558     return proving_vector, training_vector, title_text
559
560
561
562 def basicloop(self, Mstrat, Mlearn, training_instances, title_text):
563     #
564     dropout2 = 300
565     #
566     HST.title_text_sigma_train = title_text
567     #
568     for i in range(self.Pp.basicloop_iterations):
569         print("-----          basic loop", itp(i), "-----")
570         #
571         #
572         self.Pp.dropout_style = 'regular'
573         self.classificationproof(Mstrat, Mlearn, dropout2, training_instances, t
574         self.Ll.prepoolSamples(Mlearn, self.rr4.SamplePool, self.Ll.new_exempl
575         #

```

```

575         "
576         self.Ll.scoreExamples(Mlearn)
577         #
578         self.Pp.dropout_style = 'adaptive'
579         #
580         self.classificationproof(Mstrat,Mlearn,dropout2,training_instances,t
581         self.Ll.prepoolSamples(Mlearn,self.rr4.SamplePool,self.Ll.new_examp
582         self.classificationproof(Mstrat,Mlearn,100,training_instances,title_
583         self.Ll.addscoredexamples(Mlearn)
584         self.Ll.prepoolSamples(Mlearn,self.rr4.SamplePool,self.Ll.new_examp
585         #
586         self.Ll.scoreExamples(Mlearn)
587         self.Ll.scoreExplore(Mlearn)
588         self.Ll.scoreOutlier(Mlearn)
589         print("----- global learning --- ----",itp(i),"-----      ----
590         self.Ll.learningGlobal(Mlearn,self.Pp.basicloop_training_iterations)
591         if Mlearn.network2_trainable:
592             print("----- local learning --- ----",itp(i),"-----      -
593             self.Ll.learningLocal(Mlearn,self.Pp.basicloop_training_iteratio
594         else:
595             print("network 2 is not trainable")
596         print("=====  

597         gcc = gc.collect()
598         memReport('mg')
599         print("=====  

600         print("end of",itp(self.Pp.basicloop_iterations),"iterations of the basi
601         print("=====  

602         return
603
604     def basicloop_classificationproof(self,Mstrat,Mlearn,proving_instances,train
605         #
606         print("suggested number of proof cycles: between 20 and 50")
607         runs = int(input("input the number of proof cycles to do : "))
608         for s in range(runs):
609             Dd.basicloop(Mstrat,Mlearn,training_instances,title_text)
610             print(">>>",s+1," (out of ",runs," )")
611             Dd.classificationproof(Mstrat,Mlearn,0,proving_instances,title_text)
612             HST.graph_history(self.Pp,'big')
613         return
614
615     ##### the following function automates the process of choosing a collection o
616
617     def instance_chooser(self):
618         print("choose instances, this chooser allows : all, one, seg, skip (do
619         instance_type = input("input type : ")
620         if instance_type != "all" and instance_type != "one" and instance_type !=
621             print("please use one of : all one seg skip")
622             raise CoherenceError("exiting")
623         if instance_type == "all":
624             print(F"this will do all sigma instances in the existing range 0 <=
625             proving_instances, training_instances, title_text = self.InAll()
626         if instance_type == "one":
627             print(F"to do a single sigma instance, choose in range 0 <= sigma <
628             sigma_instance = int(input("input sigma instance : "))
629             proving_instances, training_instances, title_text = self.InOne(sigma
630         if instance_type == "seg":

```

```

631         print("to do sigma instances in a segment lower <= sigma < upper")
632         segment_lower = int(input("input lower : "))
633         segment_upper = int(input("input upper : "))
634         proving_instances, training_instances, title_text = self.InSeg(segment_lower, segment_upper)
635     if instance_type == "skip":
636         print("to train on a segment skipping a single value, and do proofs")
637         segment_lower = int(input("input training segment lower : "))
638         segment_upper = int(input("input training segment upper : "))
639         skip = int(input("input instance to prove, and to skip during training : "))
640         proving_instances, training_instances, title_text = self.InSkip(skip, segment_lower, segment_upper)
641     return proving_instances, training_instances, title_text
642
643

```

```

1 class Parameters : # records various parameters
2     def __init__(self):
3         #
4         print("please enter alpha, beta and model_n")
5         print("alpha = | A - A^2 | and beta = | A^2 - A^3 |, we are doing |A^3 - A^2|")
6         print("ranges 2 <= alpha, beta <= 6 and alpha + beta <= 10, GPU needed for alpha > 6")
7         print("model_n governs the size of the neural networks")
8         print("suggested value n=4, can go to n=8 for more difficult cases on GPU")
9         alpha = int(input("input alpha : "))
10        beta = int(input("input beta : "))
11        model_n = int(input("input model_n : "))
12        #
13        #
14        if alpha < 2 or beta < 2 or alpha > 6 or beta > 6 or alpha + beta > 10:
15            print("suggested range is alpha,beta in [2,...,6] and alpha + beta <= 10")
16            raise CoherenceError("exiting")
17        if model_n < 1 or model_n > 12:
18            print("suggested range for model_n is [2,...,12]")
19            raise CoherenceError("exiting")
20        #
21        self.model_n = model_n # could go up to 10 (that was what we did before)
22        #
23        self.alpha = alpha
24        self.alpha2 = alpha*alpha
25        self.alpha3 = alpha*alpha*alpha
26        self.alpha3z = self.alpha3+1
27        self.beta = beta
28        self.betaz = self.beta +1
29        #
30        HST.record_parameters(self.alpha,self.beta)
31        #
32        self.verbose = False
33        #
34        #
35        self.rdetect_max = 1000
36        #
37        self.global_params = 0
38        self.local_params = 0
39        #
40        # for rrl:

```

```
41 #
42 self.qvalue = 0.9
43 #
44 self.ascore_max = 7 # it is going to be a sum of a 0,1,2 and a 0,2,4
45 #
46 self.pastsize = 100
47 self.futuresize = 1000
48 #
49 # for rr2:
50 #
51 self.profile_filter_on = True
52 self.halfones_filter_on = True
53 #
54 # for rr3:
55 self.chunksize = 1000 # reduced this: for the 5,5 case 1000 led to memo
56 self.chunksize_extra = 10
57 self.exponent = 0.9
58 self.chunkconstant = 300
59 self.chunkextent = 10
60 #
61 self.ukseuil = 0.5
62 #
63 self.newratio = 0.8 # how much we use the model rather than benchmark v
64 self.search_epsilon = 0.3 # the proportion of randomized strategy choic
65 #
66 # for rr4:
67 self.prooflooplevelength = 4000
68 self.done_max = 30000
69 #
70 #self.sleeptime = 120 # use this on a laptop
71 self.sleeptime = 0 # was 5
72 self.periodicity = 5
73 self.stopthreshold = 100000 # too big for a notebook utilisation
74 if torch.cuda.is_available(): self.trainingiterations = 4 # was 8
75 else: self.trainingiterations = 1
76 #
77 self.root_injection = 100
78 self.randomize_q = 0.7
79 self.randomize_factor = 0.1
80 self.perturbation_factor = 0.3
81 #
82 self.spiral_mix_threshold = 10
83 self.dropout_style = 'regular'
84 #
85 #
86 # info ranges #####
87 #
88 self.infosize = 300 # currently we just need up to 250 for sample inf
89 #
90 self.samplepoints = 15
91 self.sampleinfofollower = 50
92 self.sampleinfoupper = 250 # on ecrase vilower
93 #
94 self.fulldata_location = 25
95 self.phase = 12
96 #
```

```

96      #
97      #####
98      #
99      self.basicloop_iterations = 3
100     self.basicloop_training_iterations = 3
101     #
102     self.tweak_start = 200
103     self.tweak_step = 4
104     self.tweak_density = 0.05
105     self.tweak_epsilon = 0.02
106     self.tweak_decay = 0.9
107     #
108     self.splitting_probability = 1. - ( 10**(-2. / ( itt(self.alpha).to(
109     print("splitting probability",numpr(self.splitting_probability,4) )
110     #
111     self.outlier_threshold = 2.5
112     #
113     ##### learner parameters
114     #
115     self.explore_max = 30000
116     self.examples_max = 5000
117     self.new_examples_max = 300
118     self.new_explore_max = 400
119     self.outlier_max = 2000
120     self.new_outliers_max = 300
121     #
122     self.noise_level = 0.05
123     self.noise_period = 50.
124     self.noise_decay = 0.5 # decay per period
125     #
126
127
128
129
130
131
132

```

```

1 ##### end of basic program cells #####
2 #def stopcompile():

```

```

1 ##### to set up the environment: please run this cell and enter the desired alph
2 ##### ( first suggested values are alpha = 3, beta = 2 and model_n = 4 )
3
4 HST = Historical(10000)
5 HST.proof_nodes_max = 100000 # can be used to set the upper limit for proof le
6 #
7 Pp = Parameters() # this will ask for alpha, beta and model_n
8 #
9 Pp.basicloop_iterations = 3 # default is 3
10 Pp.basicloop_training_iterations = 3 # default is 3
11 #
12 Dd = Driver(Pp)
13 #

```

```

14 # the following could be set to False to turn off those additional filters
15 Pp.profile_filter_on = True # the default is True
16 Pp.halfones_filter_on = True # the default is True
17 #
18 #####

```

```

1 ##### please run this cell to (re)initialize the model
2 #
3 Mm = SgModel(Pp)
4 Pp.spiral_mix_threshold = 4
5 Mmr = ProtoModel(Pp, 'spiral_mix')
6 #
7 #####

```

```
1
```

```
1 def stopcompile():
```

```

1 #####
2 #####
3 ##### do a classificationproof with Mmr to set benchmark, then one with Mm fo
4 ##### then do basicloop_classificationproof for example for 50 iterations
5 ##### the basicloop_classificationproof can be repeated. Cumulative results a
6 #####
7 ##### (a first suggested value for (alpha,beta)=(3,2) could be sigma = 3)
8 #####
9 #####

```

```

1 #####
2 #
3 proving_instances, training_instances, title_text = Dd.instance_chooser()
4 #
5 HST.reset()
6 Dd.classificationproof(Mmr,Mm,0,proving_instances,title_text) # sets the benchm
7 Dd.classificationproof(Mm,Mm,0,proving_instances,title_text) # to record proof

```

```
1 Dd.basicloop_classificationproof(Mm,Mm,proving_instances,training_instances,titl
```

```
1 #####
```

```

1 ##### this is the end of the main notebook part, further optional cells are incl
2 ##### also note that the previous basicloop_classificationproof cell can be repe
3 def stopcompile():

```

```
1 #####
```

```

1 ##### a function to view the initial data with instance input as above
2 Dd.print_instances()

```

```

1 ##### InList use case (this isn't covered by the instance chooser)
2 #####
3 ## modify the following as desired: proving list, training list
4 proving_instances, training_instances, title_text = Dd.InList([6,7],[5,8,9,10,11
5 #
6 HST.reset()
7 Dd.classificationproof(Mmr,Mm,0,proving_instances,title_text)
8 Dd.classificationproof(Mm,Mm,0,proving_instances,title_text)

```

```

1 Dd.basicloop_classificationproof(Mm,Mm,proving_instances,training_instances,titl

```

```

1 #####

```

```

1 def stopcompile():

```

```

1 #####

```

```

1 #####

```

```

1 ##### do the proofs in a range
2
3 for i in range(13):
4     print("instance",i)
5     proving_instances, training_instances, title_text = Dd.InOne(i)
6     Dd.classificationproof(Mm,Mm,0,proving_instances,title_text)

```

```

1 #####

```

```

1 def stopcompile():

```

```

1 #####

```

```

1 ##### next: the class used to prove the theoretical minimum (this is for alpha,be
2 ##### note that the parameters and model should be initialized for (3,2)

```

```

1 class Minimizer :    # this becomes the first element of the relations datatype
2     def __init__(self,model,sigma,cutx,cuty,cutp):
3         #
4         #
5         self.Mm = model
6         self.Pp = self.Mm.pp
7         self.Dd = Driver(self.Pp)
8         assert self.Pp.alpha == 3
9         assert self.Pp.beta == 2
10        #
11        self.sigma = sigma
12        #

```

```

12 #
13 print("Minimizer for sigma =",sigma)
14 #
15 self.rr4 = Relations4(self.Pp)
16 self.rr3 = self.rr4.rr3
17 self.rr2 = self.rr4.rr2
18 self.rr1 = self.rr4.rr1
19 self.alpha = self.Pp.alpha
20 self.alpha2 = self.Pp.alpha2
21 self.alpha3 = self.Pp.alpha3
22 self.alpha3z = self.Pp.alpha3z
23 self.beta = self.Pp.beta
24 self.betaz = self.Pp.betaz
25 #
26 self.length_max = 500000
27 #
28 instancevector, trainingvector, proof_title = self.Dd.InOne(self.sigma)
29 self.InitialData = self.Dd.initialdata(instancevector,0)
30 #
31 self.CurrentData = self.rr1.nulldata()
32 self.FullData = self.rr1.nulldata()
33 self.FullDoneData = self.rr1.nulldata()
34 #
35 self.up = torch.zeros((self.length_max),dtype = torch.int64,device=Dvc)
36 self.xvalue = torch.zeros((self.length_max),dtype = torch.int64,device=D
37 self.yvalue = torch.zeros((self.length_max),dtype = torch.int64,device=D
38 self.pvalue = torch.zeros((self.length_max),dtype = torch.int64,device=D
39 #
40 self.lowerbound = torch.zeros((self.length_max),dtype = torch.int64,devi
41 self.upperbound = torch.zeros((self.length_max),dtype = torch.int64,devi
42 #
43 self.down = torch.zeros((self.length_max,self.alpha,self.alpha,self.beta
44 self.down[:, :, :, :] = -2
45 #
46 self.split = torch.zeros((self.length_max),dtype = torch.bool,device=Dvc
47 self.inplay = torch.zeros((self.length_max),dtype = torch.bool,device=Dv
48 #
49 self.availablexyp = torch.zeros((self.length_max,self.alpha,self.alpha,s
50 self.availablexy = torch.zeros((self.length_max,self.alpha,self.alpha),d
51 #
52 self.cutx = cutx
53 self.cuty = cuty
54 self.cutp = cutp
55 print("cut to check is x y p =",cutx,cuty,cutp)
56 #
57 self.combo_all()
58
59
60 def next_stage_data(self,DataToSplit):
61 #
62 a = self.alpha
63 a2 = self.alpha2
64 a2z = self.alpha2 +1
65 a3 = self.alpha3
66 a3z = self.alpha3z
67 h = self.beta

```

```

67     bz = self.betaz
68     #
69     #
70     length = DataToSplit['length']
71     prod = DataToSplit['prod']
72     #
73     availablexyp = self.rr1.availablexyp(length,prod).view(length,a2,bz)
74     #
75     avxyp_amount = availablexyp.to(torch.float).sum(2).sum(1).sum(0)
76     avxyp_denom = itt(length).to(torch.float)
77     if avxyp_denom < 0.1:
78         avxyp_denom = 1.
79     availablexyp_average = avxyp_amount / avxyp_denom
80     ##print("average available xyp is",numpr(availablexyp_average,2))
81     #
82     lrangevxr = arangeic(length).view(length,1,1).expand(length,a2,bz).resha
83     xyvectorvxr = arangeic(a2).view(1,a2,1).expand(length,a2,bz).reshape(len
84     bzrangevxr = arangeic(bz).view(1,1,bz).expand(length,a2,bz).reshape(leng
85     #
86     verticaldetect = availablexyp[lrangevxr,xyvectorvxr,bzrangevxr]
87     #
88     #
89     ivector_vert = lrangevxr[verticaldetect]
90     xyvector_vert = xyvectorvxr[verticaldetect]
91     pvector_vert = bzrangevxr[verticaldetect]
92     #
93     prx = arangeic(a).view(a,1).expand(a,a).reshape(a2)
94     pry = arangeic(a).view(1,a).expand(a,a).reshape(a2)
95     #
96     xvector_vert = prx[xyvector_vert]
97     yvector_vert = pry[xyvector_vert]
98     #
99     #
100    #
101    NewData = self.rr1.upsplitting(DataToSplit,ivector_vert,xvector_vert,yve
102    #
103    #
104    ndlength = NewData['length']
105    #
106    #
107    AssocNewData = self.rr1.nulldata()
108    detection = torch.zeros((ndlength),dtype = torch.bool,device=Dvc)
109    newactive = torch.zeros((ndlength),dtype = torch.bool,device=Dvc)
110    newdone = torch.zeros((ndlength),dtype = torch.bool,device=Dvc)
111    newimpossible = torch.zeros((ndlength),dtype = torch.bool,device=Dvc)
112    lower = 0
113    for i in range(ndlength):
114        assert lower < ndlength
115        upper = lower + 1000
116        if upper > ndlength:
117            upper = ndlength
118        detection[:] = False
119        detection[lower:upper] = True
120        NewDataSlice = self.rr1.detectsubdata(NewData,detection)
121        AssocNewDataSlice = self.rr2.process(NewDataSlice)
122        AssocNewData = self.rr1.appenddata(AssocNewData,AssocNewDataSlice)

```

```

123         newactive_s,newdone_s,newimpossible_s = self.rr2.filterdata(AssocNew
124         newactive[lower:upper] = newactive_s
125         newdone[lower:upper] = newdone_s
126         newimpossible[lower:upper] = newimpossible_s
127         lower = upper
128         if lower >= ndlength:
129             break
130     #
131     NewActiveData = self.rr1.detectsubdata(AssocNewData,newactive)
132     #
133     NewDoneData = self.rr1.detectsubdata(AssocNewData,newdone)
134     #
135     assert len(newactive) == len(ivector_vert)
136     assert newactive.to(torch.int64).sum(0) == NewActiveData['length']
137     #
138     return ivector_vert,xvector_vert,yvector_vert,pvector_vert,newactive,new
139
140
141
142
143
144
145     def manage_initial_stage(self):
146         #
147         self.FullData = self.rr1.copydata(self.InitialData)
148         #
149         fdlength = self.FullData['length']
150         assert fdlength == 1
151         #
152         #
153         self.up[0] = -1
154         self.xvalue[0] = -1
155         self.yvalue[0] = -1
156         self.pvalue[0] = -1
157         #
158         self.lowerbound[0] = 1
159         self.upperbound[0] = 1000
160         #
161         #
162         self.split[0] = False
163         self.inplay[0] = True
164         #
165         newactive_length = self.InitialData['length']
166         newactive_prod = self.InitialData['prod']
167         #
168         new_availablexyp = self.rr1.availablexyp(newactive_length,newactive_prod)
169         new_availablexy = new_availablexyp.any(3)
170         #
171         self.availablexyp[0] = new_availablexyp
172         self.availablexy[0] = new_availablexy
173         #
174         new_fdlength = self.FullData['length']
175         #
176         self.FullData['info'][:,self.Pp.fullldata_location] = arangeic(new_fdleng
177         #

```

```

178     ##print("initialized full data that now has length",itp(new_fdlength))
179     return
180
181
182     def manage_next_stage(self):
183         #
184         fdlength = self.FullData['length']
185         if fdlength == 0:
186             self.manage_initial_stage()
187             return
188         #
189         fd_split = self.split[0:fdlength]
190         fd_inplay = self.inplay[0:fdlength]
191         #
192         fd_current = fd_inplay & ~fd_split
193         DataToSplit = self.rr1.detectsubdata(self.FullData,fd_current)
194         #
195         fd_index = arangeic(fdlength)[fd_current]
196         #
197         ivector_vert,xvector_vert,yvector_vert,pvector_vert,newactive,newdone,ne
198         #
199         inew = fd_index[ivector_vert[newactive]]
200         xnew = xvector_vert[newactive]
201         ynew = yvector_vert[newactive]
202         pnew = pvector_vert[newactive]
203         #
204         newactive_length = NewActiveData['length']
205         newactive_prod = NewActiveData['prod']
206         #
207         lower = itt(fdlength).clone()
208         upper = fdlength + newactive_length
209         if upper > self.length_max:
210             print("upper is",itp(upper),"whereas max length is",itp(self.length_
211                 raise CoherenceError("length overflow")
212         self.FullData = self.rr1.appenddata(self.FullData,NewActiveData)
213         self.FullDoneData = self.rr1.appenddata(self.FullDoneData,NewDoneData)
214         #
215         self.up[lower:upper] = inew
216         self.xvalue[lower:upper] = xnew
217         self.yvalue[lower:upper] = ynew
218         self.pvalue[lower:upper] = pnew
219         #
220         self.lowerbound[lower:upper] = 1
221         self.upperbound[lower:upper] = 1000
222         #
223         assert (~self.split[inew]).all(0)
224         assert self.inplay[inew].all(0)
225         #
226         self.split[inew] = True
227         self.split[lower:upper] = False
228         self.inplay[lower:upper] = True
229         #
230         self.down[inew,xnew,ynew,pnew] = arangeic(newactive_length) + lower
231         #
232         newimpossible = newimpossible | newdone

```

```

233     inew_id = fd_index[ivector_vert[newimpdone]]
234     xnew_id = xvector_vert[newimpdone]
235     ynew_id = yvector_vert[newimpdone]
236     pnew_id = pvector_vert[newimpdone]
237     #
238     self.down[inew_id,xnew_id,ynew_id,pnew_id] = -1
239     #
240     new_availablexyp = self.rr1.availablexyp(newactive_length,newactive_prod
241     new_availablexy = new_availablexyp.any(3)
242     #
243     self.availablexyp[lower:upper] = new_availablexyp
244     self.availablexy[lower:upper] = new_availablexy
245     #
246     #
247     new_fdlength = self.FullData['length']
248     #
249     self.FullData['info'][:,self.Pp.fullldata_location] = arangeic(new_fdleng
250     #
251     ##print("added",itp(newactive_length),"new instances to full data that n
252     return
253
254
255
256 def fd_location(self,Data):
257     length = Data['length']
258     assert length > 0
259     return Data['info'][:,self.Pp.fullldata_location]
260
261
262
263 def bounding_proofloop(self,Mstrat,fd_instances):
264     #
265     self.upperbound[fd_instances] = 1
266     #
267     Input = self.rr1.indexselectdata(self.FullData, fd_instances)
268     #
269     InitialActiveData = self.rr2.process(Input)
270     activedetect, donedetected, impossibledetect = self.rr2.filterdata(Initial
271     #
272     ActivePool = self.rr1.detectsubdata(InitialActiveData,activedetect)
273     #
274     stepcount = 0
275     #
276     ##print("at step",itp(stepcount),"currently proof nodes for fd instances
277     ##print(numpy(self.upperbound[fd_instances]))
278     #
279     for i in range(self.rr4.prooflooplength):
280         stepcount += 1
281         prooflength = i
282         if ActivePool['length'] > 0:
283             #
284             print(".",end = '')
285             if (i%50) == 49:
286                 print(" ")
287             if (i%100) == 0:

```



```

343     rd_inplay = self.inplay[0:rdlength]
344     #
345     fd_current = fd_inplay & ~fd_split
346     #
347     fd_instances = arangeic(fdlength)[fd_current]
348     #
349     self.bounding_proofloop(self.Mm,fd_instances)
350     return
351
352     def recursive_bound_step(self):
353         #
354         fdlength = self.FullData['length']
355         assert fdlength > 0
356         #
357         fd_up = self.up[0:fdlength]
358         fd_xvalue = self.xvalue[0:fdlength]
359         fd_yvalue = self.yvalue[0:fdlength]
360         fd_pvalue = self.pvalue[0:fdlength]
361         #
362         fd_lowerbound = self.lowerbound[0:fdlength]
363         fd_upperbound = self.upperbound[0:fdlength]
364         #
365         fd_down = self.down[0:fdlength]
366         #
367         fd_split = self.split[0:fdlength]
368         fd_inplay = self.inplay[0:fdlength]
369         #
370         fd_current = fd_inplay & ~fd_split
371         fd_lookat = fd_inplay & fd_split
372         fd_uppable = (fd_up >= 0)
373         #
374         fd_availablexyp = self.availablexyp[0:fdlength]
375         fd_availablexy = self.availablexy[0:fdlength]
376         #
377         #fd_impdone_xyp = (fd_down == -1)
378         #
379         fd_lowerbound_xyp = torch.zeros((fdlength,self.alpha,self.alpha,self.beta))
380         fd_upperbound_xyp = torch.zeros((fdlength,self.alpha,self.alpha,self.beta))
381         #
382         ivalue_uppable = fd_up[fd_uppable]
383         xvalue_uppable = fd_xvalue[fd_uppable]
384         yvalue_uppable = fd_yvalue[fd_uppable]
385         pvalue_uppable = fd_pvalue[fd_uppable]
386         #
387         fd_lowerbound_xyp[ivalue_uppable,xvalue_uppable,yvalue_uppable,pvalue_uppable] = fd_lowerbound_xyp[ivalue_uppable,xvalue_uppable,yvalue_uppable,pvalue_uppable]
388         fd_upperbound_xyp[ivalue_uppable,xvalue_uppable,yvalue_uppable,pvalue_uppable] = fd_upperbound_xyp[ivalue_uppable,xvalue_uppable,yvalue_uppable,pvalue_uppable]
389         #
390         fd_lowerbound_xy_r = fd_lowerbound_xyp.sum(3).reshape(fdlength*self.alpha*self.alpha)
391         fd_upperbound_xy_r = fd_upperbound_xyp.sum(3).reshape(fdlength*self.alpha*self.alpha)
392         fd_availablexy_r = fd_availablexy.reshape(fdlength*self.alpha*self.alpha)
393         #
394         fd_lowerbound_xy_r[~fd_availablexy_r] = 10000
395         fd_upperbound_xy_r[~fd_availablexy_r] = 10000
396         #
397         fd_lowerbound_xy_rv = fd_lowerbound_xy_r.view(fdlength,self.alpha*self.alpha)
398         fd_upperbound_xy_rv = fd_upperbound_xy_r.view(fdlength,self.alpha*self.alpha)

```

```

398     fd_upperbound_xy_rv = fd_upperbound_xy_r.view(fdlength, self.alpha * self.a
399     #
400     fd_lowerbound_min, fdlbmindices = torch.min(fd_lowerbound_xy_rv, 1)
401     fd_upperbound_min, fdubmindices = torch.min(fd_upperbound_xy_rv, 1)
402     #
403     fd_lowerbound_new = fd_lowerbound.clone()
404     fd_upperbound_new = fd_upperbound.clone()
405     fd_lowerbound_new[fd_lookat] = fd_lowerbound_min[fd_lookat]
406     fd_upperbound_new[fd_lookat] = fd_upperbound_min[fd_lookat]
407     #
408     ##print("new lower bound")
409     ##print(nump(fd_lowerbound_new))
410     ##print("new upper bound")
411     ##print(nump(fd_upperbound_new))
412     #
413     self.lowerbound[0:fdlength] = fd_lowerbound_new
414     self.upperbound[0:fdlength] = fd_upperbound_new
415     return
416
417     def recursive_bound(self, iterations):
418         #
419         fdlength = self.FullData['length']
420         assert fdlength > 0
421         #
422         lower_all = self.lowerbound[0:fdlength].sum(0)
423         upper_all = self.upperbound[0:fdlength].sum(0)
424         ##print("init with lower sum", itp(lower_all), "upper sum", itp(upper_all))
425         for i in range(iterations):
426             self.recursive_bound_step()
427             lower_new = self.lowerbound[0:fdlength].sum(0)
428             upper_new = self.upperbound[0:fdlength].sum(0)
429             ##print("iteration", i, "with lower sum", itp(lower_new), "upper sum", itp(upper_new))
430             #
431             if lower_new == lower_all and upper_new == upper_all:
432                 ##print("stabilizes")
433                 break
434             else:
435                 lower_all = lower_new
436                 upper_all = upper_new
437         ##print("done with recursive bound steps")
438         return
439
440
441
442     def remove_from_play(self, subset):
443         #
444         #
445         fdlength = self.FullData['length']
446         #
447         fd_up = self.up[0:fdlength]
448         fd_up_mod = torch.clamp(fd_up, 0, fdlength)
449         #
450         inplay_prev = self.inplay[0:fdlength].to(torch.int64).sum(0)
451         ##print("previous in play count is", itp(inplay_prev))
452         ##print("removing", itp(subset.to(torch.int64).sum(0)), "locations from pl
453         #

```

```

454     self.inplay[0:fdlength] = self.inplay[0:fdlength] & (~subset)
455     #
456     for i in range(100):
457         inplay_count = self.inplay[0:fdlength].to(torch.int64).sum(0)
458         inplay_up = self.inplay[fd_up_mod]
459         self.inplay[0:fdlength] = self.inplay[0:fdlength] & inplay_up
460         if self.inplay[0:fdlength].to(torch.int64).sum(0) == inplay_count:
461             break
462         inplay_new = self.inplay[0:fdlength].to(torch.int64).sum(0)
463         ##print("new in play count is",itp(inplay_new))
464         #
465     return
466
467     def random_remove_from_play(self,threshold):
468         fdlength = self.FullData['length']
469         tirage = torch.rand((fdlength),device=Dvc)
470         subset = (tirage < threshold)
471         subset[0] = False
472         self.remove_from_play(subset)
473     return
474
475     def leave_in_play(self,instance): # for now we assume that this is at the f
476         fdlength = self.FullData['length']
477         subset = torch.ones((fdlength),dtype = torch.bool,device=Dvc)
478         subset[0] = False
479         subset[instance] = False
480         self.remove_from_play(subset)
481     return
482
483     def initial_cut(self,x,y,p):
484         fdlength = self.FullData['length']
485         #assert fdlength == 28
486         instance = self.down[0,x,y,p]
487         subset = torch.ones((fdlength),dtype = torch.bool,device=Dvc)
488         subset[0] = False
489         subset[instance] = False
490         self.remove_from_play(subset)
491     return
492
493     def prune(self):
494         #
495         fdlength = self.FullData['length']
496         #
497         fd_lowerbound = self.lowerbound[0:fdlength]
498         fd_upperbound = self.upperbound[0:fdlength]
499         fd_inplay = self.inplay[0:fdlength]
500         #
501         badlocations = (fd_lowerbound > fd_upperbound) & fd_inplay
502         badlocations_count = badlocations.to(torch.int64).sum(0)
503         #
504         ##if badlocations_count > 0:
505             ##print("warning, we found",itp(badlocations_count),"bad locations")
506         ##else:
507             ##print("all locations are good")
508         #

```

```

509     attained = (fd_lowerbound == fd_upperbound) & fd_inplay
510     attained_count = attained.to(torch.int64).sum(0)
511     #
512     up_mod = torch.clamp(self.up[0:fdlength], 0, fdlength)
513     #
514     upperbound_up = self.upperbound[up_mod]
515     nonoptimal = (fd_lowerbound + 1) >= upperbound_up
516     nonoptimal[0] = False
517     nonoptimal_count = nonoptimal.to(torch.int64).sum(0)
518     #
519     to_remove = nonoptimal | attained
520     #
521     ##print("found",itp(attained_count),"attained and",itp(nonoptimal_count))
522     self.remove_from_play(to_remove)
523     ##print("done pruning")
524     return
525
526
527 def combo_init(self):
528     #print("----- initial combo segments -----")
529     #print("----- manage next stage (two iterations)")
530     self.manage_next_stage()
531     self.manage_next_stage()
532     print("----- make initial cut at",self.cutx,self.cuty,self.cutp)
533     self.initial_cut(self.cutx,self.cuty,self.cutp)
534     #print("----- calculate current upper bound")
535     self.calculate_current_upperbound()
536     #print("----- recursive bound")
537     self.recursive_bound(100)
538     #print("----- prune")
539     self.prune()
540     #print("----- done with initial combo segment -----")
541     return
542
543 def combo_step(self):
544     #print("----- combo segment -----")
545     checkdone = self.check_done()
546     if checkdone:
547         print("|||")
548         return 'done'
549     #print("----- manage next stage")
550     self.manage_next_stage()
551     #print("----- calculate current upper bound")
552     self.calculate_current_upperbound()
553     #print("----- recursive bound")
554     self.recursive_bound(100)
555     #print("----- prune")
556     self.prune()
557     #print("----- done with combo segment -----")
558     return 'continue'
559
560 def check_done(self):
561     fdlength = self.FullData['length']
562     #
563     fd_lowerbound = self.lowerbound[0:fdlength]

```

```

564     fd_upperbound = self.upperbound[0:fdlength]
565     fd_inplay = self.inplay[0:fdlength]
566     #
567     inplay_count = fd_inplay.to(torch.int64).sum(0)
568     if inplay_count > 1:
569         return False
570     else:
571         assert fd_inplay[0]
572         cutx = self.cutx
573         cuty = self.cuty
574         cutp = self.cutp
575         cut_instance = self.down[0,cutx,cuty,cutp]
576         assert self.lowerbound[cut_instance] == self.upperbound[cut_instance]
577         print("at initial cut location",cutx,cuty,cutp,"lower bound = upper
578         print("this was for sigma =",self.sigma)
579         #
580         lb_next = torch.zeros((self.alpha,self.alpha),dtype = torch.int64,de
581         ub_next = torch.zeros((self.alpha,self.alpha),dtype = torch.int64,de
582         for x in range(self.alpha):
583             for y in range(self.alpha):
584                 if self.availablexy[cut_instance,x,y]:
585                     lb_next[x,y] = 1
586                     ub_next[x,y] = 1
587                     for p in range(self.betaz):
588                         if self.availablexyp[cut_instance,x,y,p]:
589                             down_xyp = self.down[cut_instance,x,y,p]
590                             if down_xyp > 0:
591                                 lb_next_xyp = self.lowerbound[down_xyp]
592                                 assert lb_next_xyp > 0
593                                 lb_next[x,y] += lb_next_xyp
594                                 #
595                                 ub_next_xyp = self.upperbound[down_xyp]
596                                 ub_next[x,y] += ub_next_xyp
597         #
598         ##print("lower bounds for the next cut locations x,y are as follows:
599         ##print(nump(lb_next))
600         ##print("upper bounds")
601         ##print(nump(ub_next))
602         ##print("full data length was",itp(fdlength))
603         ##self.show_neural_network_results()
604         #
605     return True
606
607 def check_done_print(self):
608     fdlength = self.FullData['length']
609     #
610     fd_lowerbound = self.lowerbound[0:fdlength]
611     fd_upperbound = self.upperbound[0:fdlength]
612     fd_inplay = self.inplay[0:fdlength]
613     #
614     inplay_count = fd_inplay.to(torch.int64).sum(0)
615     if inplay_count > 1:
616         print("not done: there are remaining locations in play")
617         return False
618     else:

```

```

619         assert fd_inplay[0]
620         cutx = self.cutx
621         cuty = self.cuty
622         cutp = self.cutp
623         cut_instance = self.down[0,cutx,cuty,cutp]
624         assert self.lowerbound[cut_instance] == self.upperbound[cut_instance]
625         print("at initial cut location",cutx,cuty,cutp,"lower bound = upper
626         print("this was for sigma =",self.sigma)
627         #
628         lb_next = torch.zeros((self.alpha,self.alpha),dtype = torch.int64,de
629         ub_next = torch.zeros((self.alpha,self.alpha),dtype = torch.int64,de
630         for x in range(self.alpha):
631             for y in range(self.alpha):
632                 if self.availablexy[cut_instance,x,y]:
633                     lb_next[x,y] = 1
634                     ub_next[x,y] = 1
635                     for p in range(self.betaz):
636                         if self.availablexyp[cut_instance,x,y,p]:
637                             down_xyp = self.down[cut_instance,x,y,p]
638                             if down_xyp > 0:
639                                 lb_next_xyp = self.lowerbound[down_xyp]
640                                 assert lb_next_xyp > 0
641                                 lb_next[x,y] += lb_next_xyp
642                                 #
643                                 ub_next_xyp = self.upperbound[down_xyp]
644                                 ub_next[x,y] += ub_next_xyp
645         #
646         print("lower bounds for the next cut locations x,y are as follows:")
647         print(nump(lb_next - 1))
648         print("upper bounds")
649         print(nump(ub_next - 1))
650         print("lower and upper bounds should coincide. Add 1 to plug back in
651         print("full data length was",itp(fdlength))
652         #self.show_neural_network_results()
653         #
654         return True
655
656     def show_neural_network_results(self): # not currently working, also our ne
657         #
658         fdlength = self.FullData['length']
659         #
660         subset = torch.zeros((fdlength),dtype = torch.bool,device=Dvc)
661         subset[0:500] = True
662         TruncatedFullData = self.rr1.detectsubdata(self.FullData,subset)
663         fd_network_output = self.Mm.network(TruncatedFullData).detach()
664         net2 = M.network2(TruncatedFullData)
665         fd_network2_output = net2.detach()
666         #
667         fdn2_exp_rootv = (10**fd_network2_output[0]).view(self.alpha*self.alpha)
668         avxy_rootv = self.availablexy[0].view(self.alpha*self.alpha)
669         fdn2_exp_rootv[~avxy_rootv] = 0.
670         fdn2_exp_rootmod = fdn2_exp_rootv.view(self.alpha,self.alpha)
671         print("network 2 output at root")
672         print(numpr(fdn2_exp_rootmod,2))
673         #

```



```

727 #
730 sigma = int(input("input sigma : "))
731 self.sigma = sigma
732 #
733 print("Minimizer History for sigma =",sigma)
734 print("with profile_filter_on =",self.Pp.profile_filter_on,"and halfones
735
736 #
737 self.rr4 = Relations4(self.Pp)
738 self.rr3 = self.rr4.rr3
739 self.rr2 = self.rr4.rr2
740 self.rr1 = self.rr4.rr1
741 self.alpha = self.Pp.alpha
742 self.alpha2 = self.Pp.alpha2
743 self.alpha3 = self.Pp.alpha3
744 self.alpha3z = self.Pp.alpha3z
745 self.beta = self.Pp.beta
746 self.betaz = self.Pp.betaz
747 #
748 instancevector, trainingvector, proof_title = self.Dd.InOne(self.sigma)
749 self.InitialData = self.Dd.initialdata(instancevector,0)
750 #
751 self.results = torch.zeros((self.alpha,self.alpha,self.betaz),dtype = to
752 #
753 idlength = self.InitialData['length']
754 idprod = self.InitialData['prod']
755 self.availablexyp = self.rr1.availablexyp(idlength,idprod)[0]
756 #
757
758 def print_results(self):
759 #
760 results_sum = self.results.sum(2)
761 #
762 minimal = results_sum[0,0]
763 for x in range(self.alpha):
764     for y in range(self.alpha):
765         if results_sum[x,y] < minimal:
766             minimal = results_sum[x,y]
767 root_minimum = minimal + 1
768 print("+= += += += += += += += += += +=
769 print("+= += += += += += += += += += +=
770 print("          aggregation of results for sigma =",itp(self.sigma
771 print("+= += += += += += += += += += +=
772 print("+= += += += += += += += += += +=
773 #
774 print("summed results according to initial cut location are:")
775 print(numpy(results_sum))
776 print("the minimal number of nodes including the root is",itp(root_minim
777 print("this was with profile_filter_on =",self.Pp.profile_filter_on,"and
778 print("-----
779 return
780
781 def minimize_all(self):
782 #
783 for x in range(self.alpha):
784     for v in range(self.alpha):

```

```

785         for p in range(self.betaz):
786             if self.availablexyp[x,y,p]:
787                 Min = Minimizer(self.Mm,self.sigma,x,y,p)
788                 cut_instance = Min.down[0,x,y,p]
789                 assert Min.lowerbound[cut_instance] == Min.upperbound[cut_instance]
790                 self.results[x,y,p] = Min.lowerbound[cut_instance]
791     self.print_results()
792     return
793
794
795

```

```

1 Pp.profile_filter_on = True
2 Pp.halfones_filter_on = True

```

```

1 MH = MinimizerHistory(Mmr) # asks to choose sigma
2 MH.minimize_all() # this does all the cases in a row

```

```

1 def stopcompile():

```

```

1 Min = Minimizer(Mm,3,0,0,0) # individual cases: sigma, x, y, p
2 Min.check_done_print()
3 #time.sleep(60)

```

```

1 Min = Minimizer(Mm,3,0,0,1) # individual cases: sigma, x, y, p
2 Min.check_done_print()
3 #time.sleep(60)

```

```

1 Min = Minimizer(Mm,3,0,0,2) # individual cases: sigma, x, y, p
2 Min.check_done_print()
3 #time.sleep(60)

```

```

1

```

```

1 ##### next: a class that can be used to search for specific examples, it was a

```

```

1 class FindWeirdStuff :
2     def __init__(self,Dd,Mm):
3         #
4         #
5         self.Dd = Dd
6         self.Ll = self.Dd.Ll
7         self.Mm = Mm
8         #
9         self.Pp = self.Dd.Pp
10        #
11        self.rr4 = self.Dd.rr4
12        self.rr3 = self.rr4.rr3
13        self.rr2 = self.rr4.rr2

```

```

13
14     self.rr1 = self.rr4.rr1
15     self.alpha = self.Pp.alpha
16     self.alpha2 = self.Pp.alpha2
17     self.alpha3 = self.Pp.alpha3
18     self.alpha3z = self.Pp.alpha3z
19     self.beta = self.Pp.beta
20     self.betaz = self.Pp.betaz
21     #
22
23     def sample_box(self,xlower,xupper,ylower,yupper):
24         #
25         smb,DataBatch,scorebatch = self.Ll.selectminibatch(500)
26         #
27         if not smb:
28             print("select mini batch fails")
29             return False,None
30         predictedscore = self.Mm.network(DataBatch)
31         #
32         detectionx = (xlower < scorebatch) & (scorebatch < xupper)
33         detectiony = (ylower < predictedscore) & (predictedscore < yupper)
34         detection = detectionx & detectiony
35         #
36         DetectedData = self.rr1.detectsubdata(DataBatch,detection)
37         #
38         return True, DetectedData
39
40     def printright(self,right,loc):
41         #
42         a=self.alpha
43         a2=a*a
44         a3=a*a*a
45         a3z = a3+1
46         b=self.beta
47         bz = b+1
48         #
49         prarray = torch.zeros((bz,a),dtype = torch.int64,device=Dvc)
50         for x in range(bz):
51             for y in range(a):
52                 column = right[loc,x,y]
53                 prarray[x,y] = self.Dd.printcolumn2(column)
54         print(nump(prarray))
55         return
56
57     def print_prod_left_right(self,Data,i):
58         prod = Data['prod']
59         left = Data['left']
60         right = Data['right']
61         #
62         print("-----")
63         print("at location",itp(i),"the prod, left and right are respectively")
64         self.Dd.printprod(prod,i)
65         self.Dd.printleft(left,i)
66         self.printright(right,i)
67         print("-----")
68         return

```

```

69
70 def print_column_bool(self,column):
71     clength = len(column)
72     toprint = 3 * (10 ** (clength))
73     for q in range(clength):
74         toprint += (column[q].to(torch.int64) * (10 ** q) )
75     return toprint
76
77 def print_bool_tensor(self,a,b,c,btensor):
78     prarray = torch.zeros((a,b),dtype = torch.int64,device=Dvc)
79     for x in range(a):
80         for y in range(b):
81             column = btensor[x,y]
82             prarray[x,y] = self.print_column_bool(column)
83     print(nump(prarray))
84     return
85
86
87 def print_one_sample_from_box(self,xlower,xupper,ylower,yupper):
88     #
89     sb,DetectedData = self.sample_box(xlower,xupper,ylower,yupper)
90     #
91     if not sb:
92         print("exit from one sample box")
93         return
94     length = DetectedData['length']
95     if length == 0:
96         print("didn't detect any samples in this box")
97         return
98     #
99     AssocData = self.rr2.process(DetectedData)
100    activedetect, donedetected, impossibledetect = self.rr2.filterdata(AssocDa
101    permutation = torch.randperm(length,device=Dvc)
102    loc = permutation[0]
103    print("before processing:")
104    self.print_prod_left_right(DetectedData,loc)
105    print("after processing:")
106    self.print_prod_left_right(AssocData,loc)
107    print("the status of this location is :",end = ' ')
108    if activedetect[loc]:
109        print("active")
110    if donedetected[loc]:
111        print("done")
112    if impossibledetect[loc]:
113        print("impossible")
114    return
115
116 def av_root(self,DataToSplit,i):
117     a = self.alpha
118     a2 = self.alpha2
119     a2z = self.alpha2 +1
120     a3 = self.alpha3
121     a3z = self.alpha3z
122     b = self.beta
123     bz = self.betaz

```

```

124     #
125     #
126     length = DataToSplit['length']
127     prod = DataToSplit['prod']
128     #
129     availablexypi = self.rr1.availablexyp(length,prod).view(length,a,a,bz)[i
130     #
131     print("at root, availablexyp is:")
132     self.print_bool_tensor(a,a,bz,availablexypi)
133     #
134     return
135
136     def split_by_hand(self,DataToSplit,i,x,y,p):
137         a = self.alpha
138         a2 = self.alpha2
139         a2z = self.alpha2 +1
140         a3 = self.alpha3
141         a3z = self.alpha3z
142         b = self.beta
143         bz = self.betaz
144         #
145         #
146         length = DataToSplit['length']
147         prod = DataToSplit['prod']
148         #
149         availablexypi = self.rr1.availablexyp(length,prod).view(length,a,a,bz)[i
150         #
151         available_instance = availablexypi[x,y,p]
152         if available_instance:
153             print("this instance",itp(x),itp(y),itp(p),"is available")
154         else:
155             print("this instance",itp(x),itp(y),itp(p),"is not available")
156             return
157         #
158         ivector = torch.zeros((1),dtype = torch.int64,device=Dvc)
159         ivector[:] = i
160         xvector = torch.zeros((1),dtype = torch.int64,device=Dvc)
161         xvector[:] = x
162         yvector = torch.zeros((1),dtype = torch.int64,device=Dvc)
163         yvector[:] = y
164         pvector = torch.zeros((1),dtype = torch.int64,device=Dvc)
165         pvector[:] = p
166         #
167         #
168         NewData = self.rr1.upsplitting(DataToSplit,ivector,xvector,yvector,pvect
169         #
170         #
171         ndlength = NewData['length']
172         assert ndlength == 1
173         #
174         AssocNewData = self.rr2.process(NewData)
175         #
176         newactive,newdone,newimpossible = self.rr2.filterdata(AssocNewData)
177         if newactive[0]:
178             print("active")

```

```

179     if newdone[0]:
180         print("done")
181     if newimpossible[0]:
182         print("impossible")
183     #
184     AND_prod = AssocNewData['prod']
185     AND_length = 1
186     AND_availablexyp = self.rr1.availablexyp(AND_length,AND_prod).view(1,a,a
187     print("after cut at",itp(x),itp(y),itp(p),"availablexyp is:")
188     self.print_bool_tensor(a,a,bz,AND_availablexyp)
189     print("prod is")
190     self.print_bool_tensor(a,a,bz,AND_prod[0])
191     #
192     #
193     return AND_prod
194
195     def show_cut_column(self,sigma,x,y): # shows the results of (x,y,p) cut sta
196     #
197     instancevector, trainingvector, title_text = self.Dd.InOne(sigma)
198     InitialData = self.Dd.initialdata(instancevector, 0)
199     #
200     self.av_root(InitialData,0)
201     #
202     for p in range(self.betaz):
203         #
204         andprod = self.split_by_hand(InitialData,0,x,y,p)
205     return
206
207     def searchprod(self,Data,trprod):
208     #
209     a = self.alpha
210     bz = self.betaz
211     #
212     length = Data['length']
213     prod = Data['prod']
214     #
215     if length == 0:
216         print("length is 0")
217         return 0,None
218     prodv = prod.view(length,a*a*bz)
219     trprodv = trprod.view(1,a*a*bz).expand(length,a*a*bz)
220     #
221     detection = (prodv == trprodv).all(1)
222     #
223     detected_indices = arangeic(length)[detection]
224     detected_length = detection.to(torch.int64).sum(0)
225     print("detected",itp(detected_length),"occurences out of",itp(length))
226     return detected_length, detected_indices
227
228
229     def tracer(self,trprod):
230     #
231     print("Examples:",end=' ')
232     dl,di = self.searchprod(self.L1.Examples,trprod)
233     print("ExamplesPrePool:",end=' ')

```

```

234     dl,di = self.searchprod(self.Ll.ExamplesPrePool,trprod)
235     print("ExplorePrePool:",end=' ')
236     dl,di = self.searchprod(self.Ll.ExplorePrePool,trprod)
237     print("OutlierPrePool:",end=' ')
238     dl,di = self.searchprod(self.Ll.OutlierPrePool,trprod)
239     #
240     #
241     return
242
243     def tracer_root(self,sigma):
244         #
245         instancevector, trainingvector, title_text = self.Dd.InOne(sigma)
246         InitialData = self.Dd.initialdata(instancevector, 0)
247         #
248         trprod = InitialData['prod'][0]
249         #
250         self.tracer(trprod)
251         #
252         return
253
254     def tracer_subroot(self,sigma,x,y,p):
255         #
256         instancevector, trainingvector, title_text = self.Dd.InOne(sigma)
257         InitialData = self.Dd.initialdata(instancevector,0)
258         #
259         trprod = self.split_by_hand(InitialData,0,x,y,p)
260         #
261         self.tracer(trprod)
262         #
263         return
264
265     def trace(self,stringtoprint,Data,sigma,x,y,p):
266         #
267         instancevector, trainingvector, title_text = self.Dd.InOne(sigma)
268         InitialData = self.Dd.initialdata(instancevector,0)
269         #
270         trprod = self.split_by_hand(InitialData,0,x,y,p)
271         #
272         print(stringtoprint,end=' ')
273         dl,di = self.searchprod(Data,trprod)
274         return
275
276
277
278

```

```
1 Fws = FindWeirdStuff(Dd,Mm)
```

```
1 ### a few things to do with that
```

```
1 Fws.tracer_root(5)
```

```
1 Fws.tracer_subroot(5,0,0,0)
```

```
1 Fws.show_cut_column(5,2,1)
```

```
1 Fws.print_one_sample_from_box(0.25,0.35,0.0,0.2)
```

```
1 Fws.print_one_sample_from_box(0.0,0.05,0.0,0.2)
```

1

1

```

1 #####
2 #####
3 #####
4
5 #####
6 #####
7 #####
8
9 #####
10 #####
11 #####
12
13 #####
14 #####
15 #####
16
17 #####
18 #####
19 #####

```

1

1

1

1

1

1

1

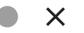

Supplement: Supplementary file 1 [file sgLearnNil4_ipynb.pdf]
